# Supplementary material for: Optimizing performance of quantum operations with non-Markovian decoherence: the tortoise or the hare?
Source: arXiv:2303.16002 ancillary file (2023-11-20)

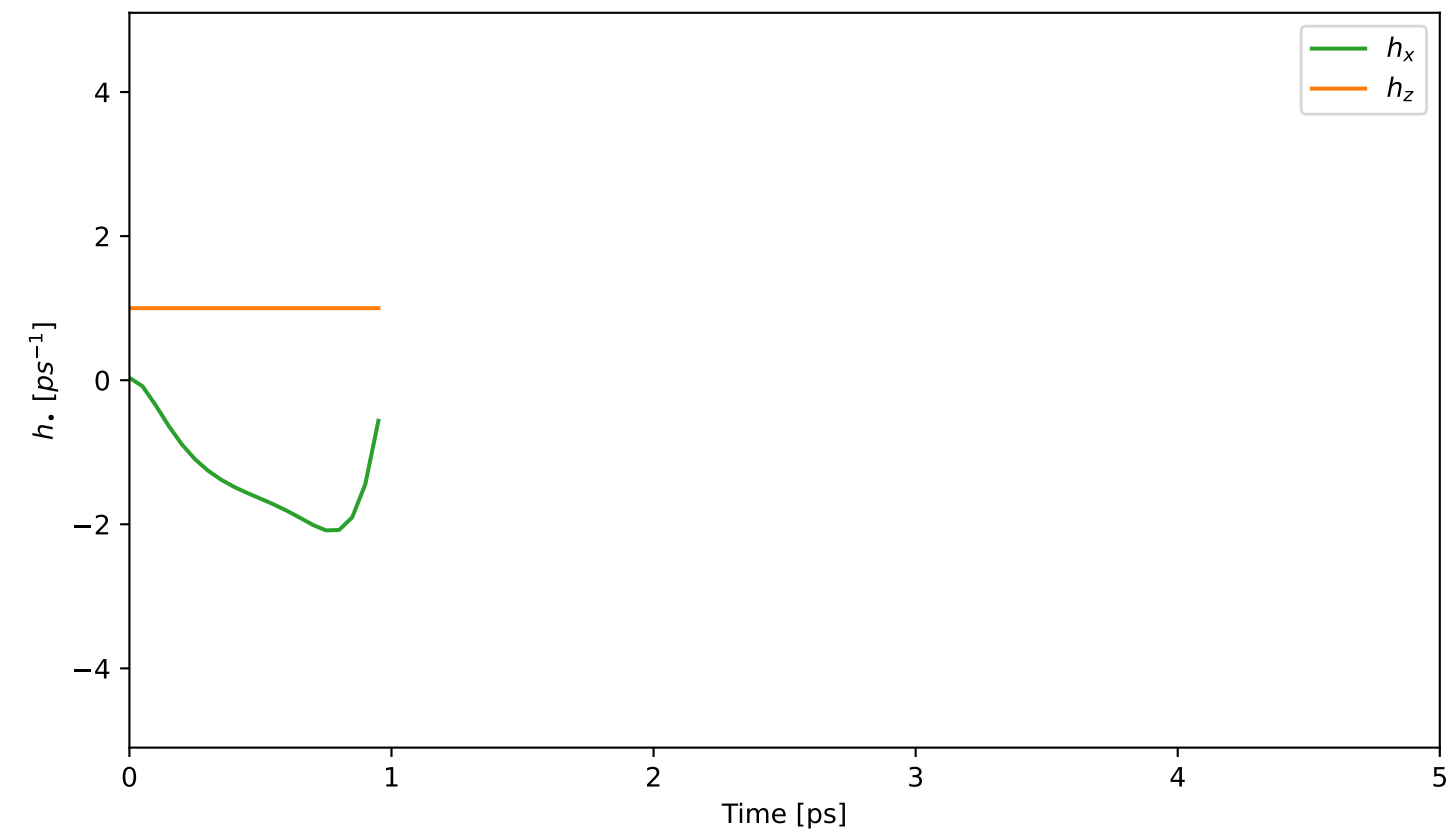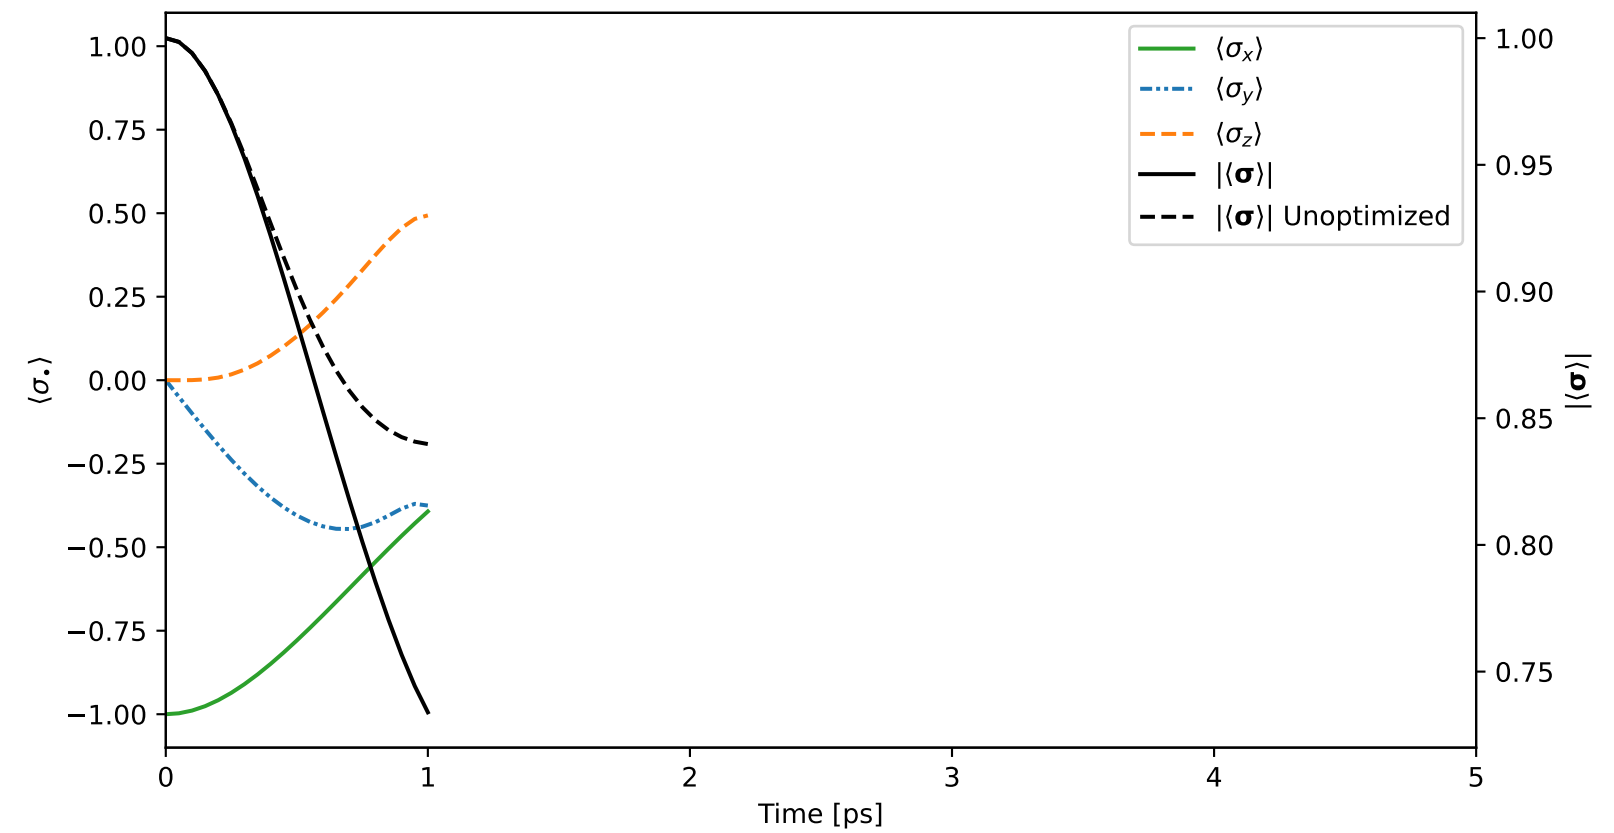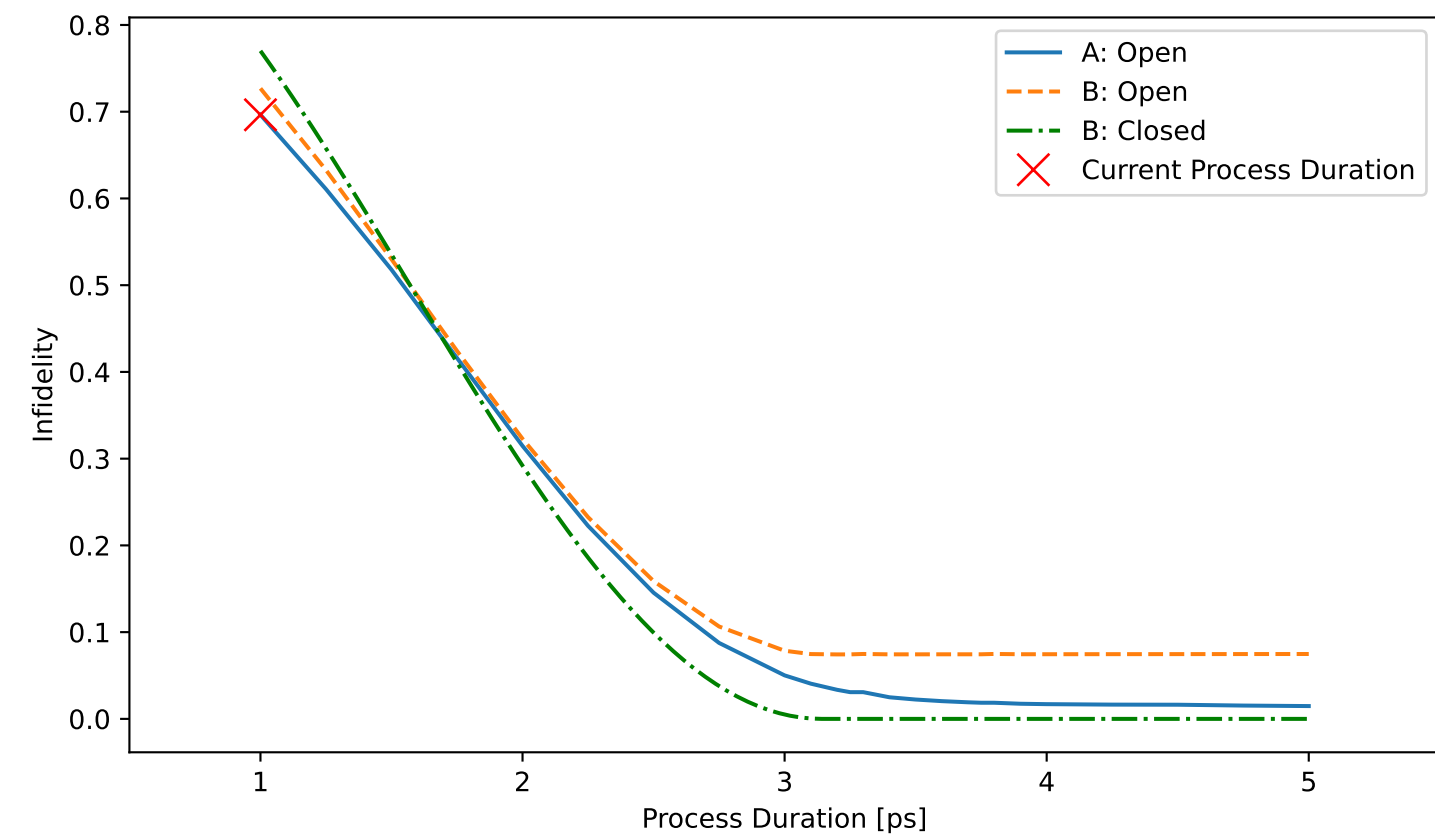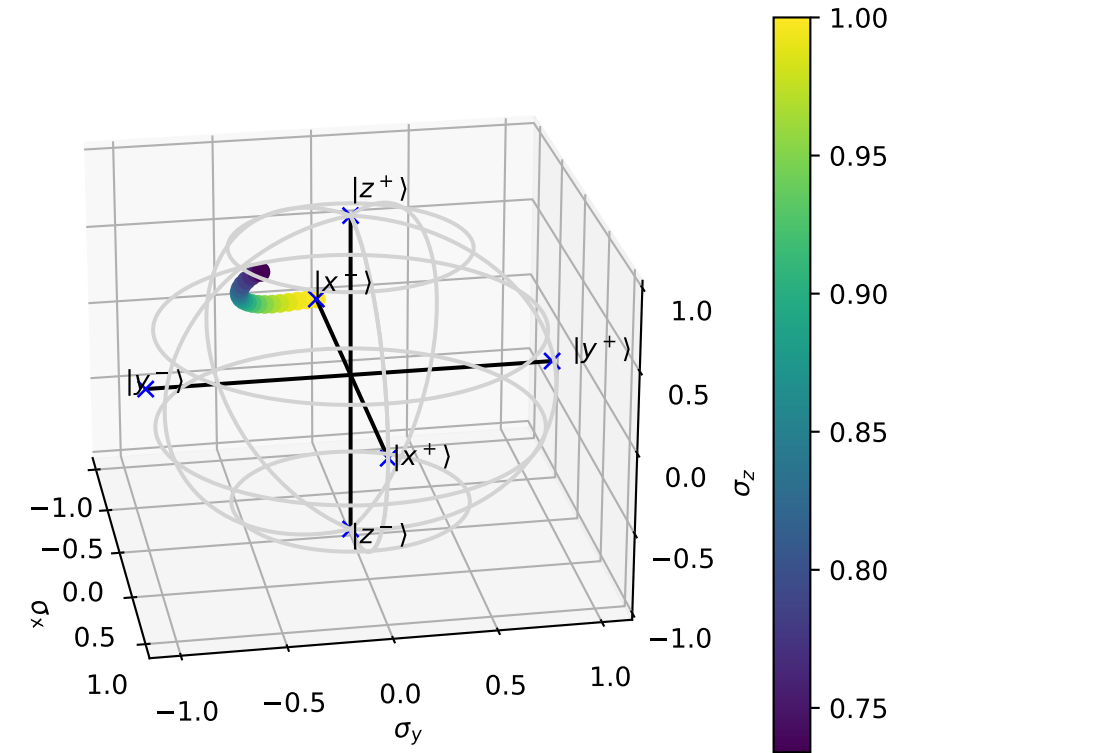

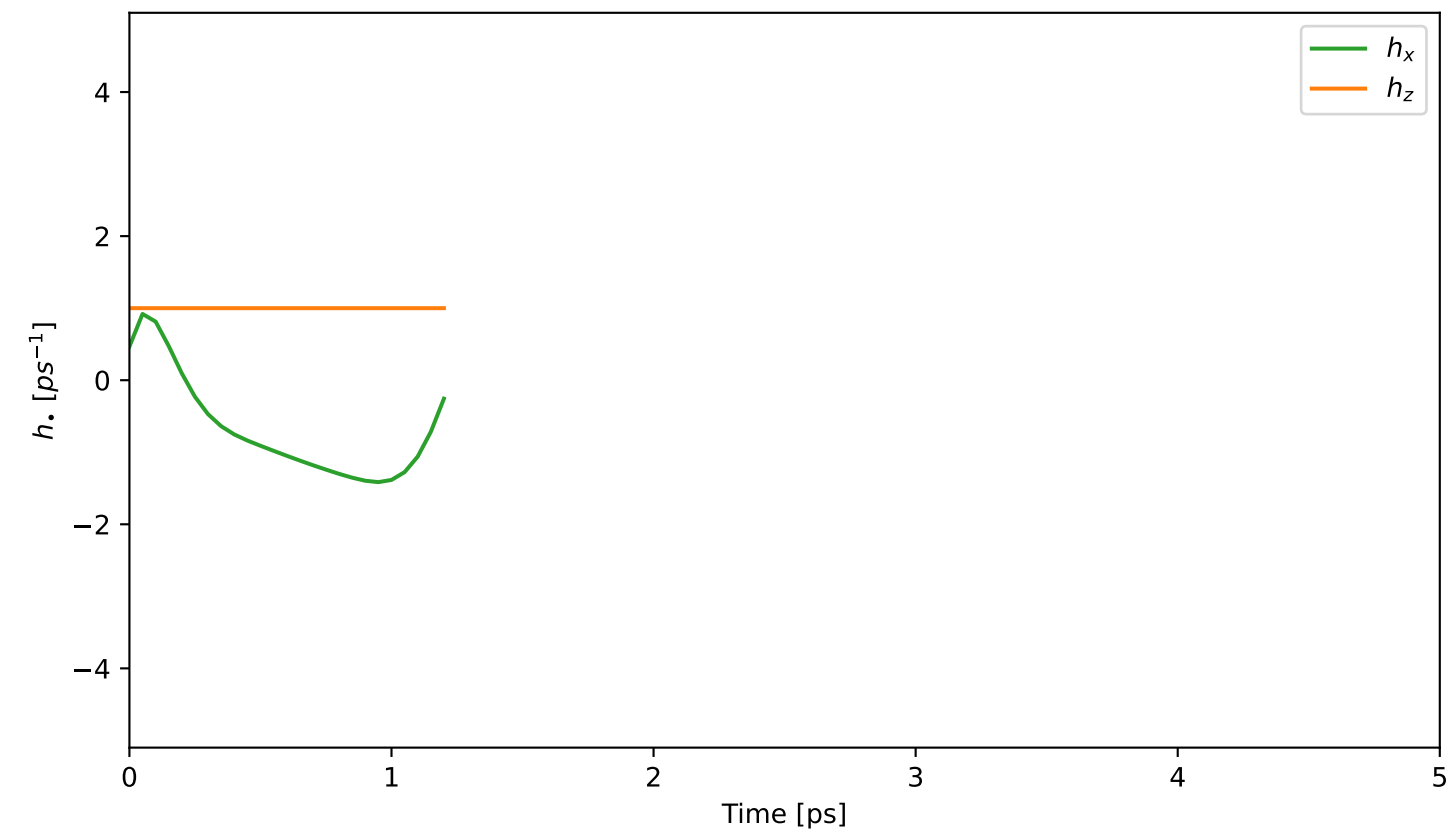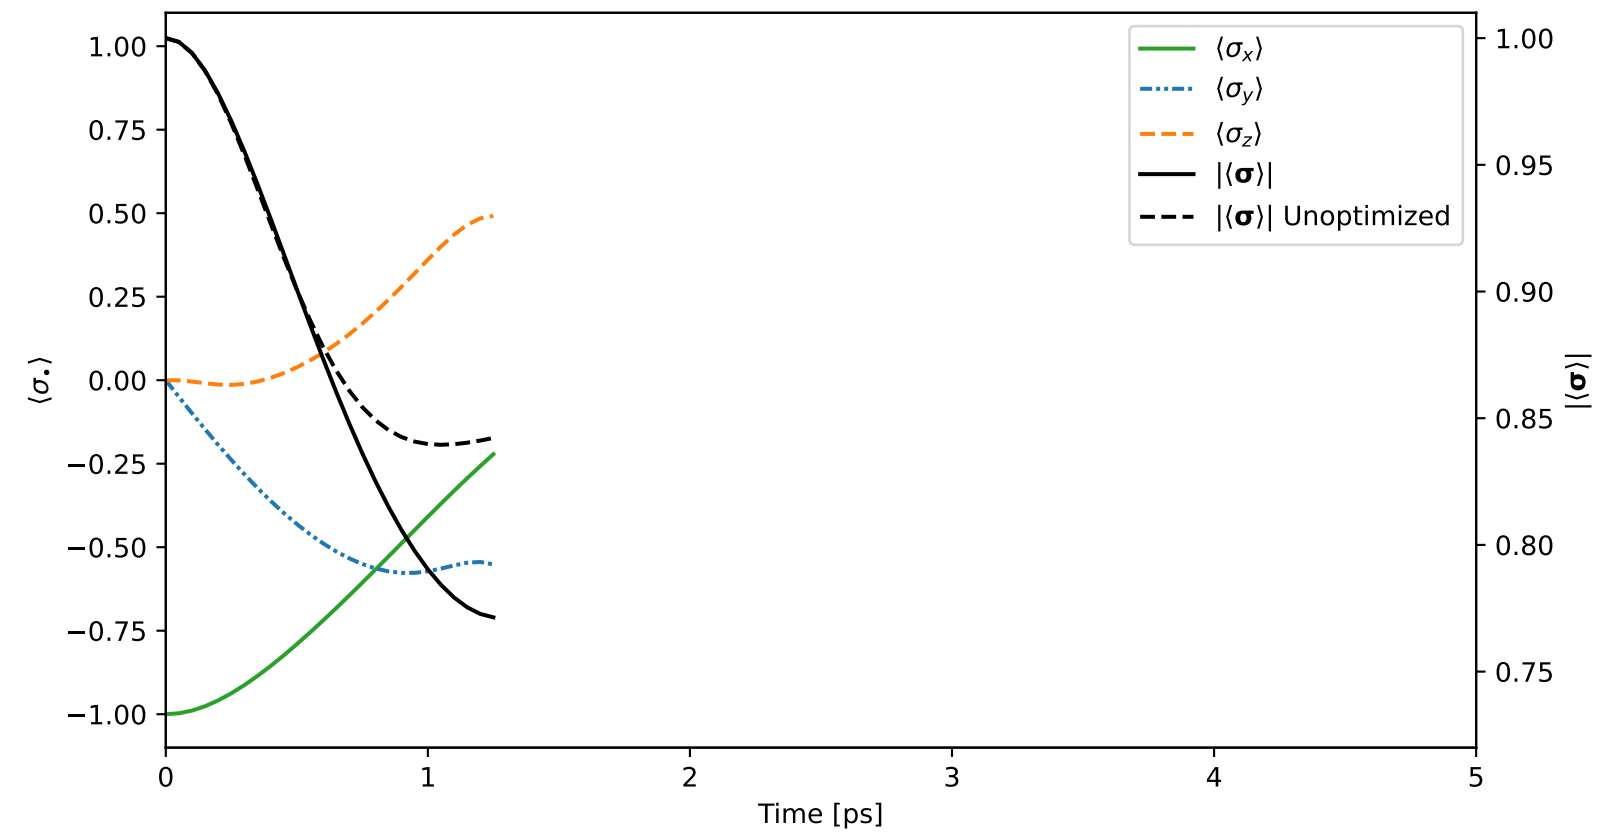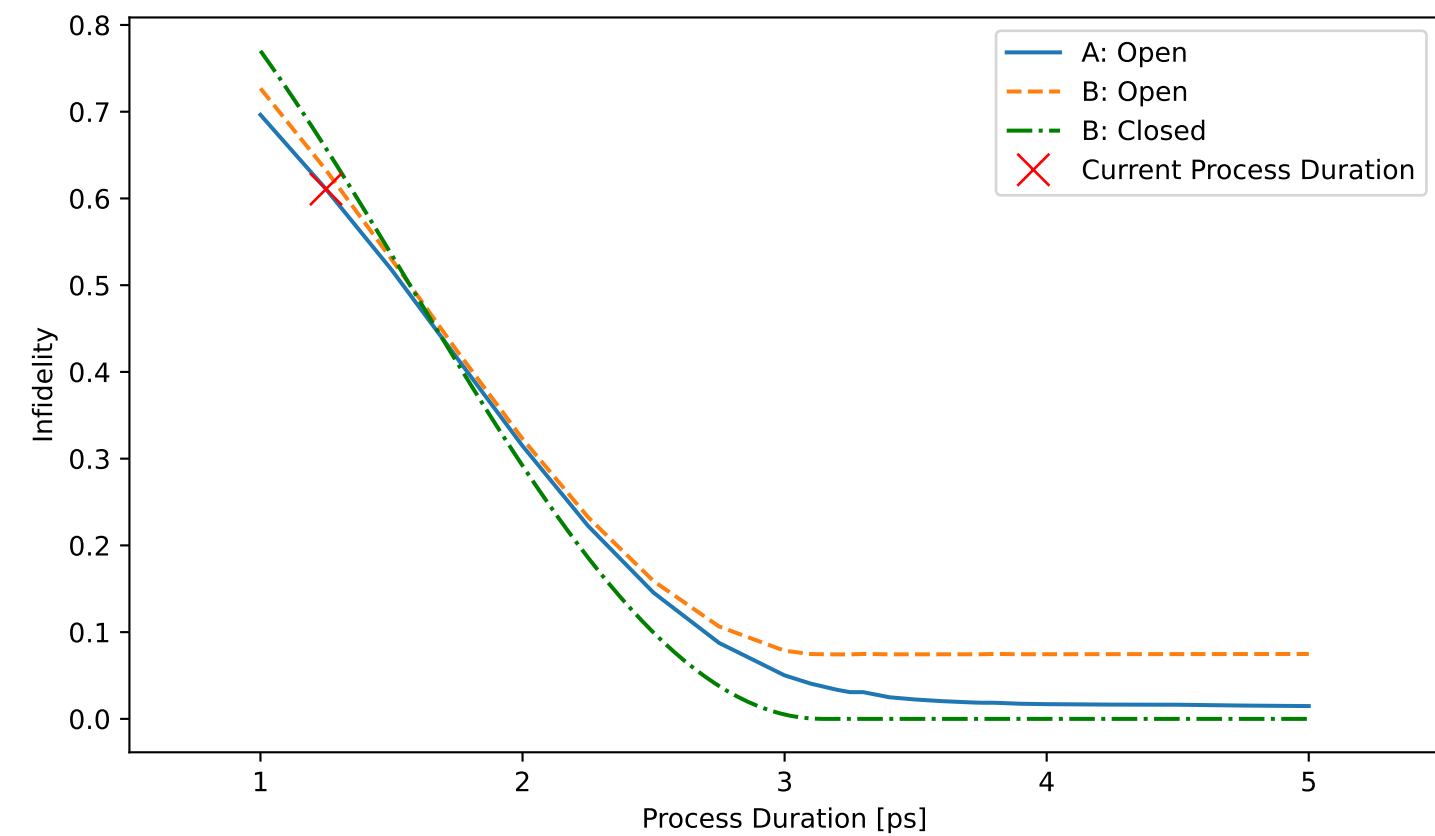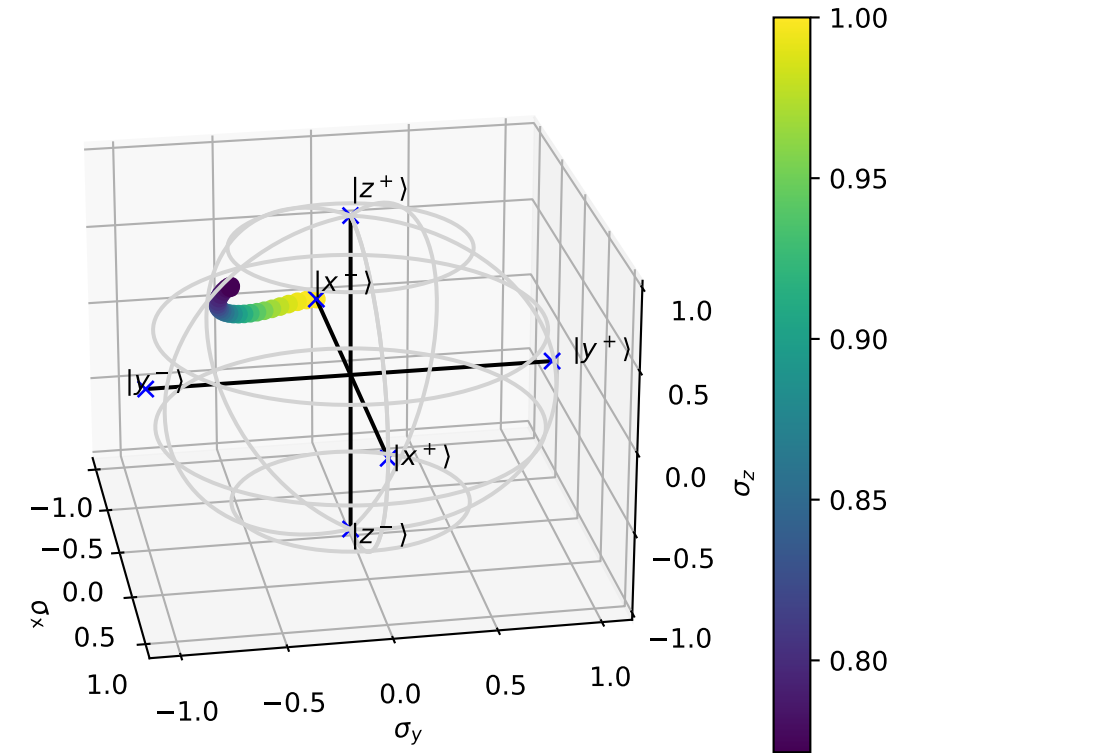

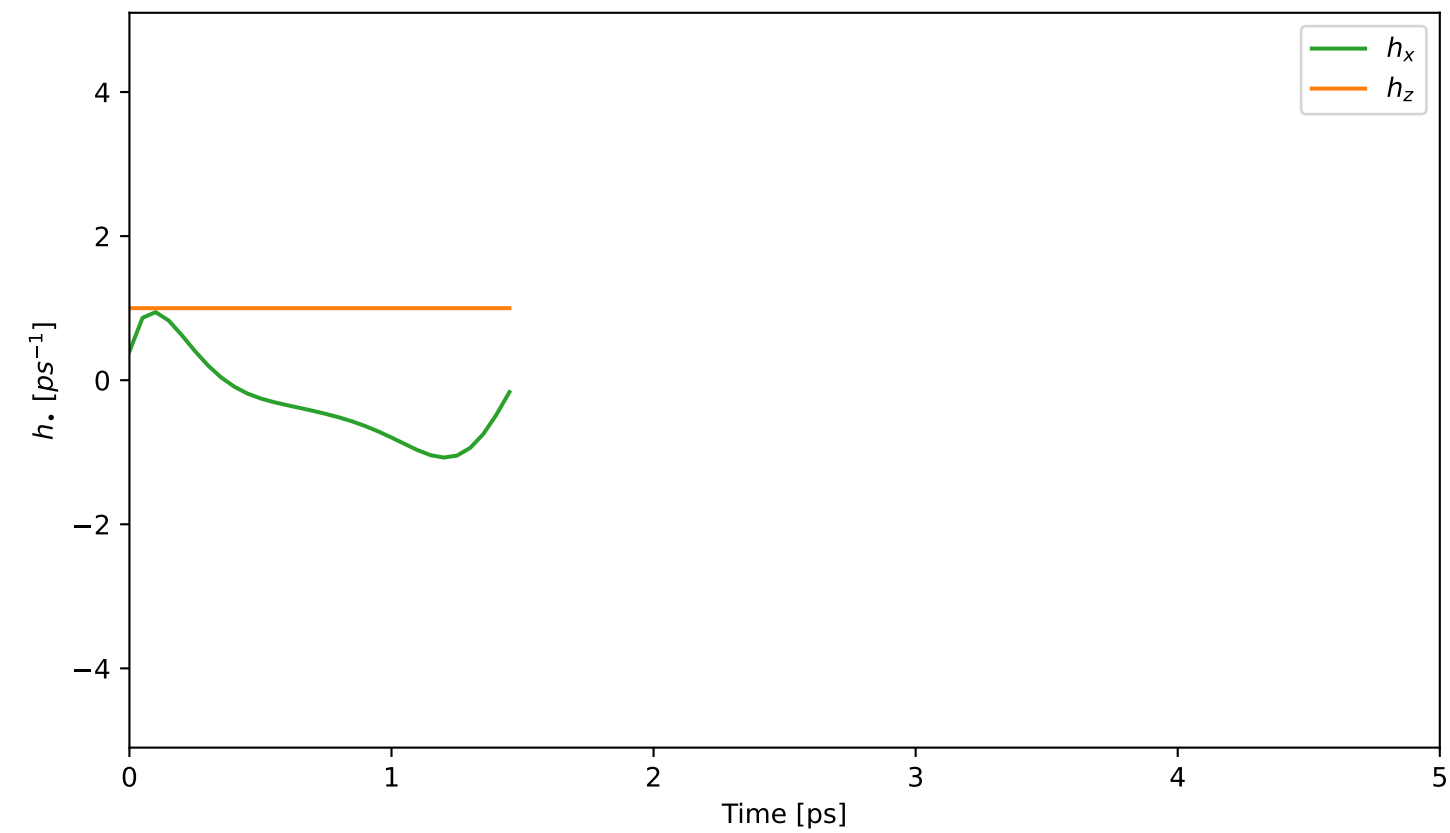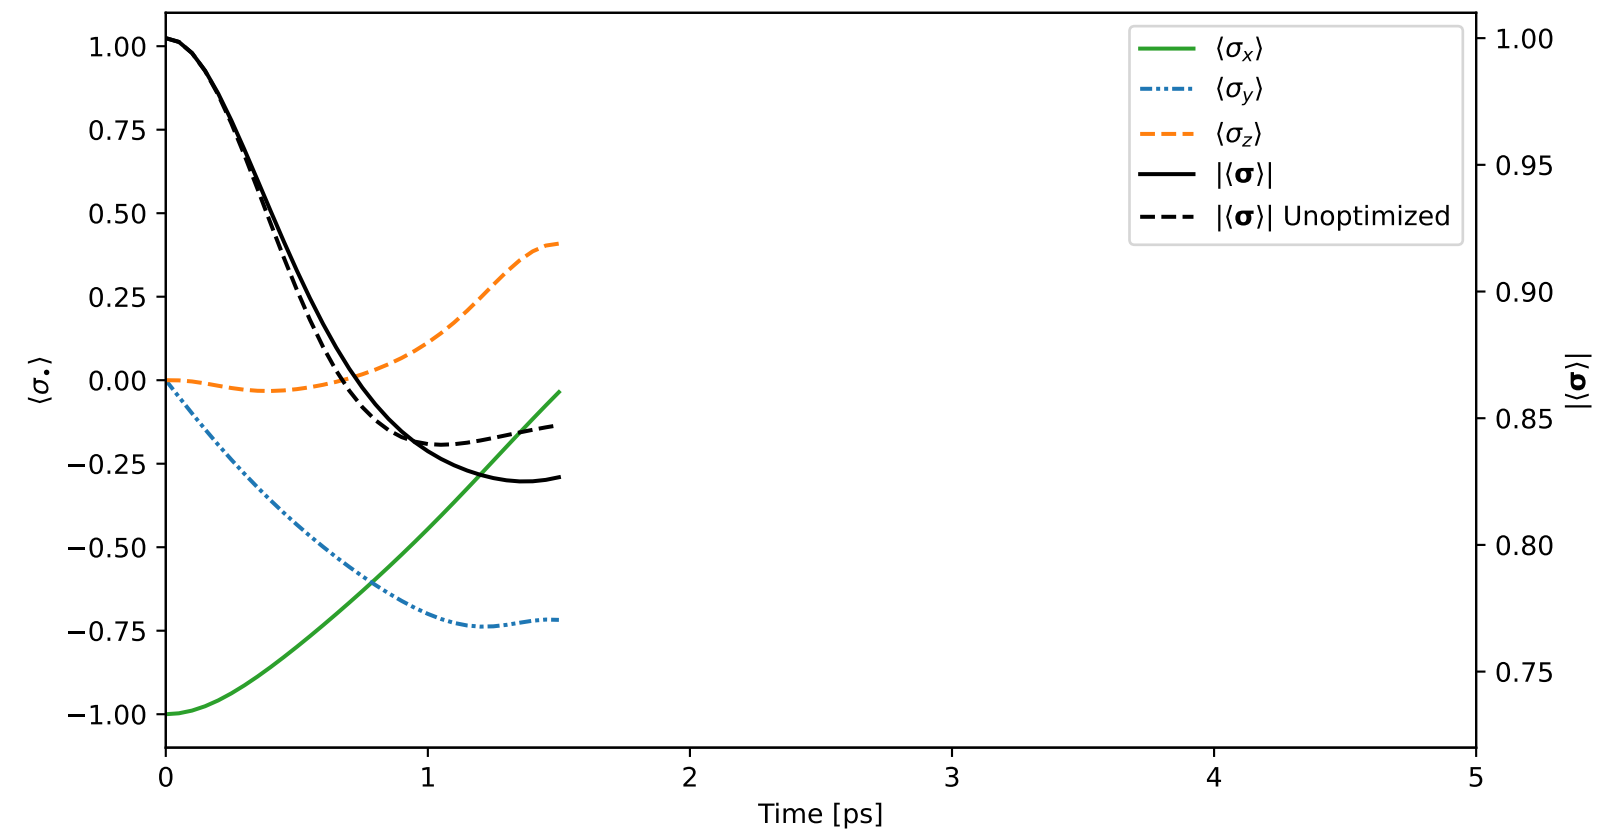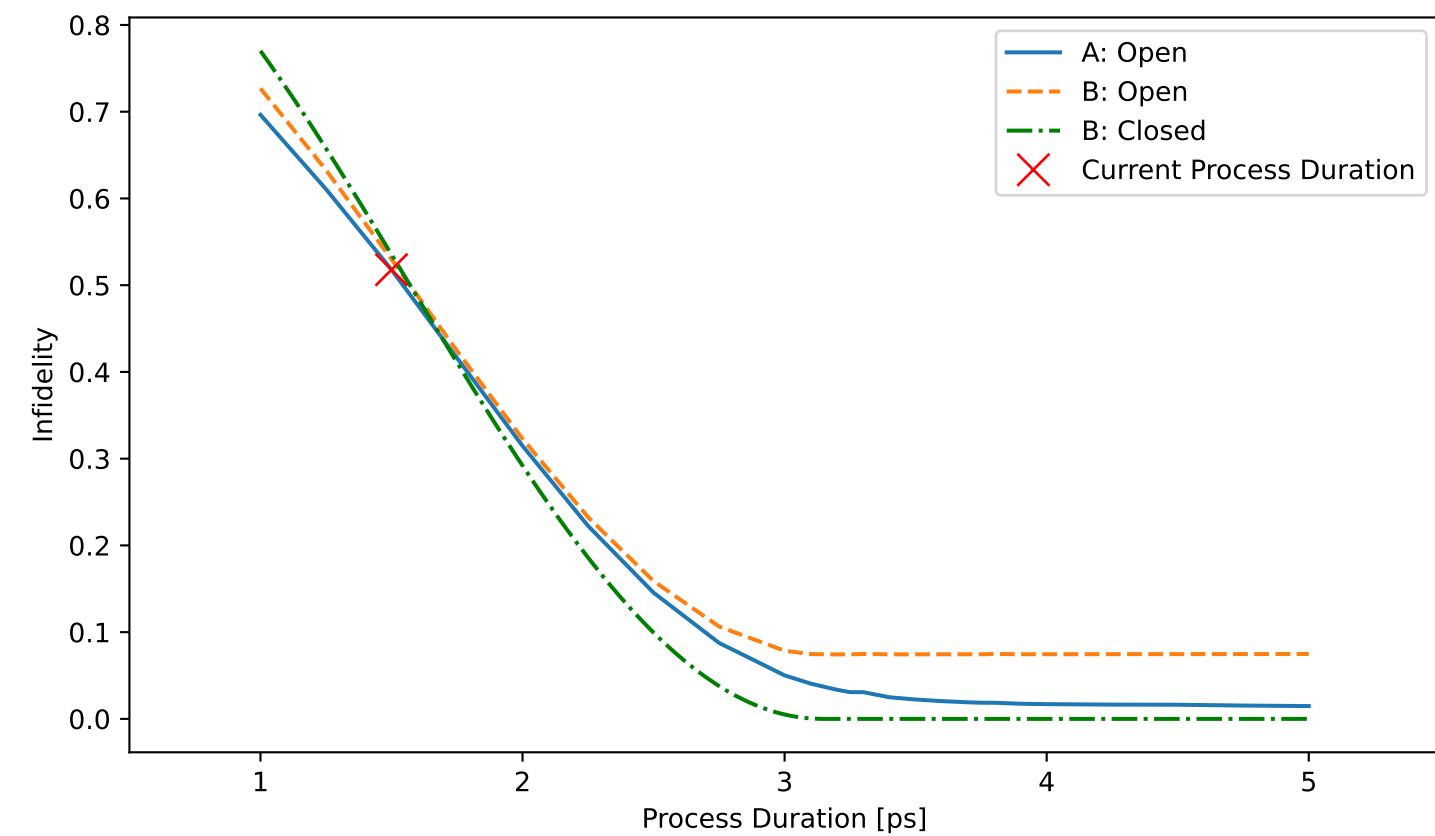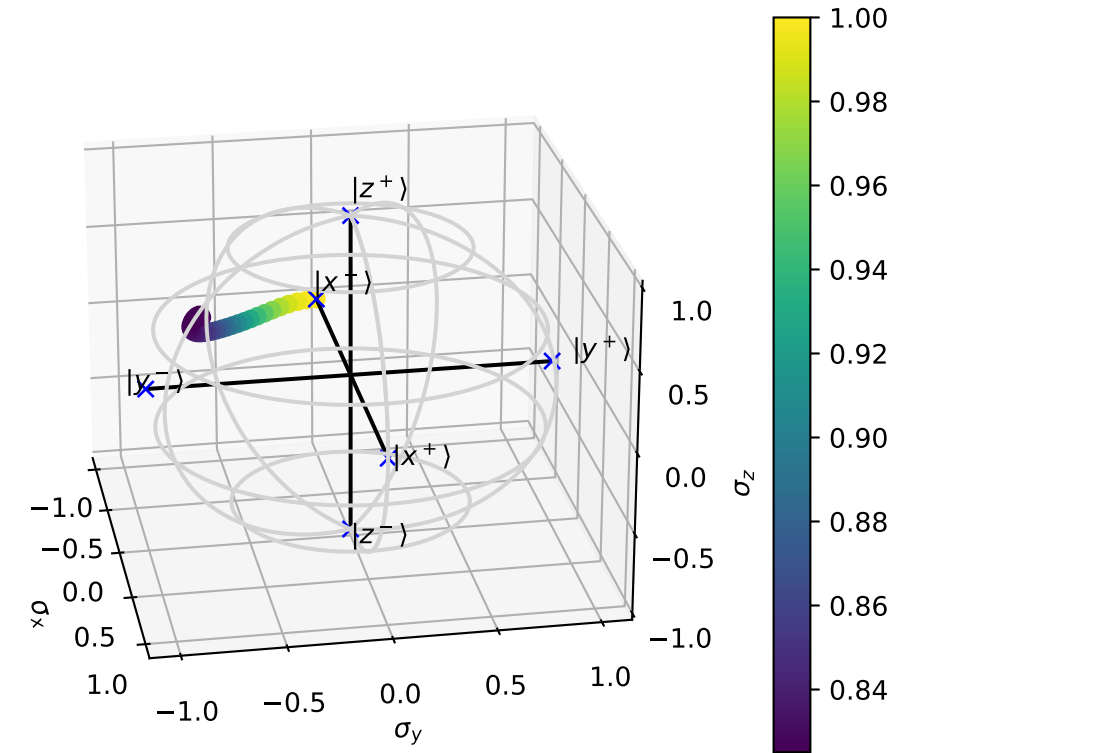

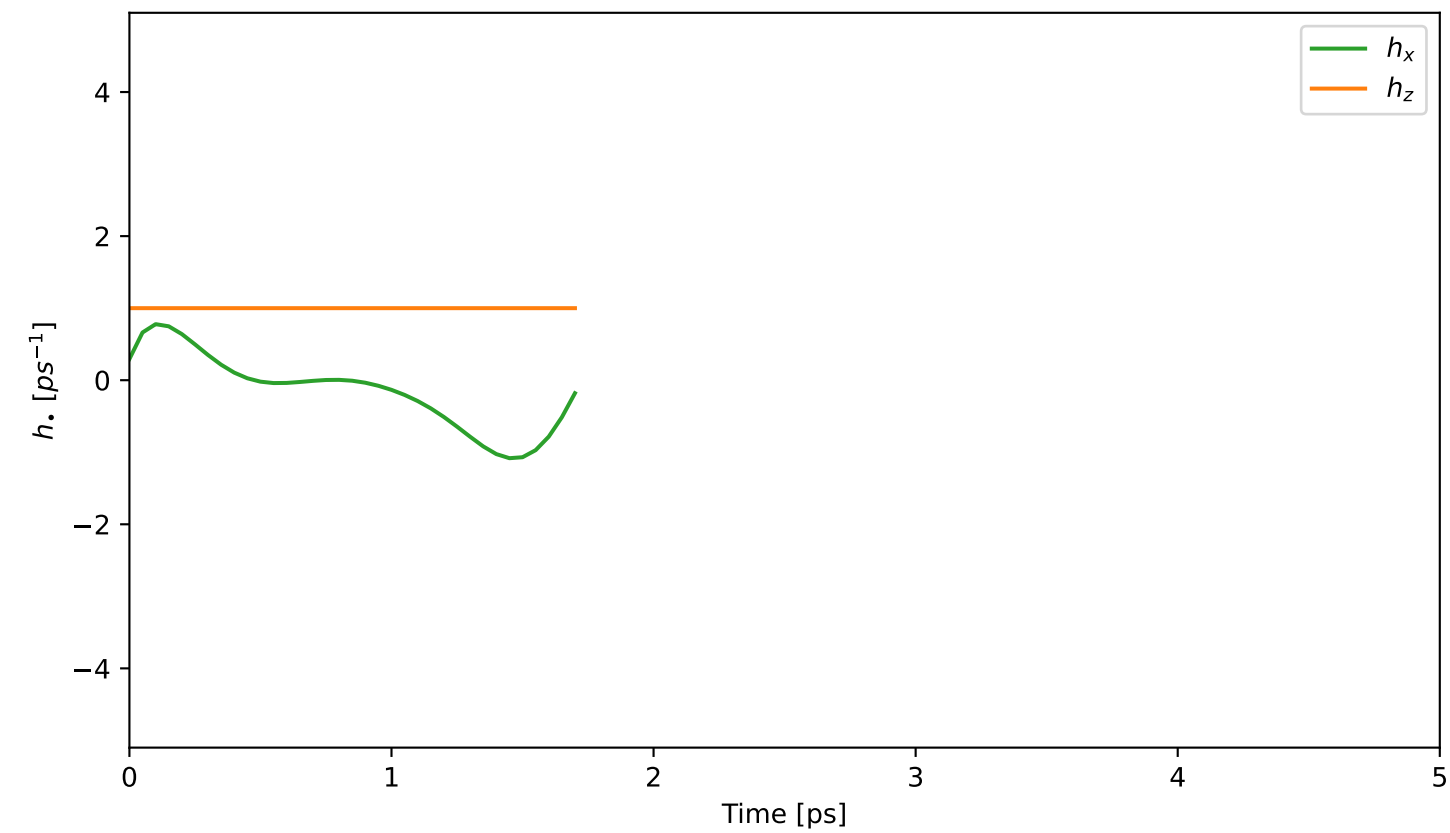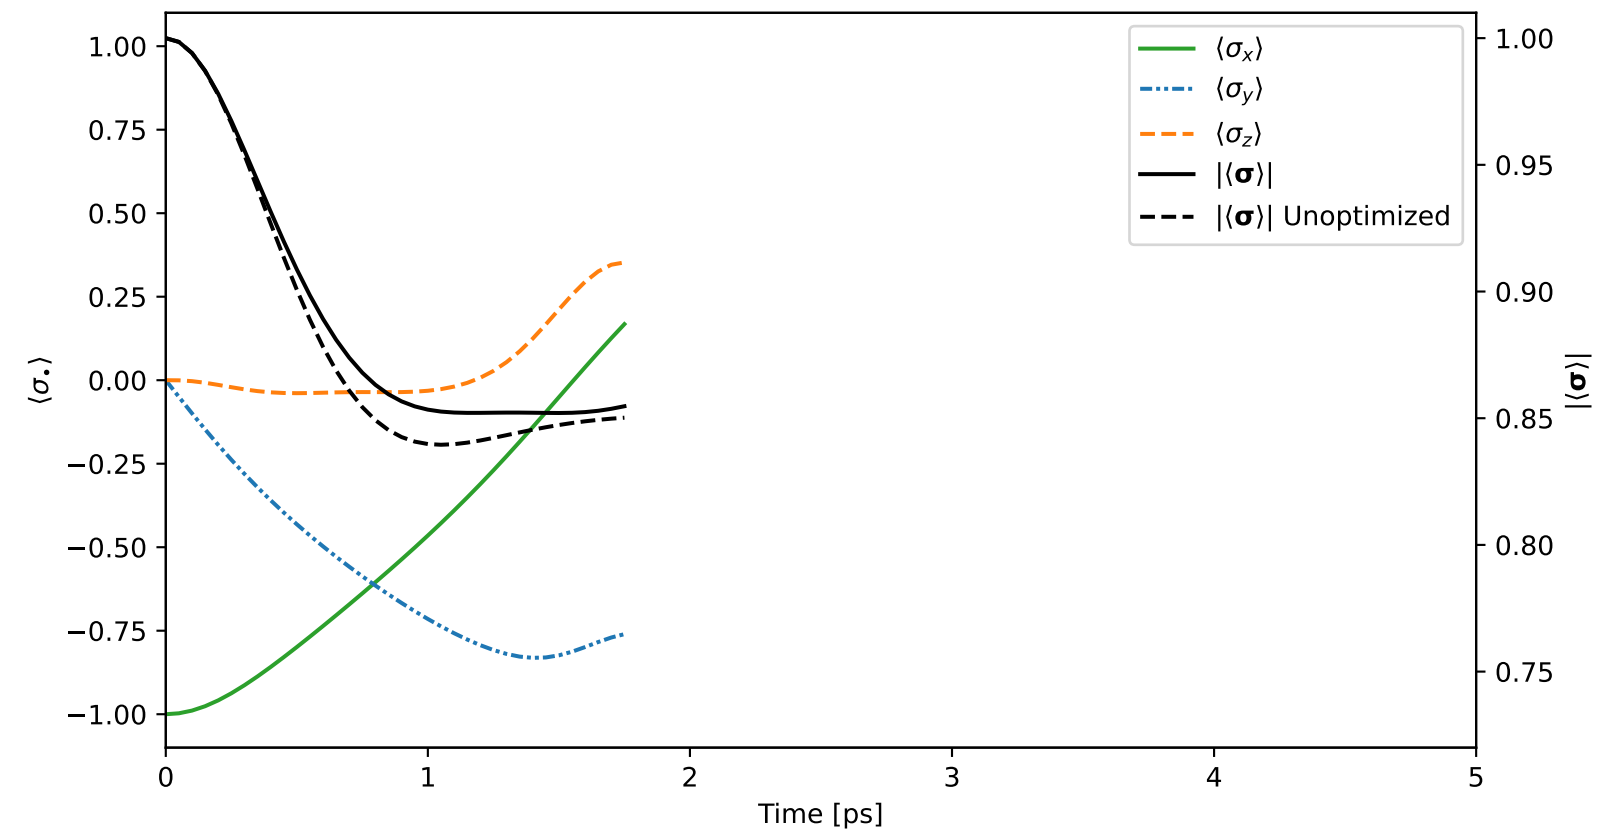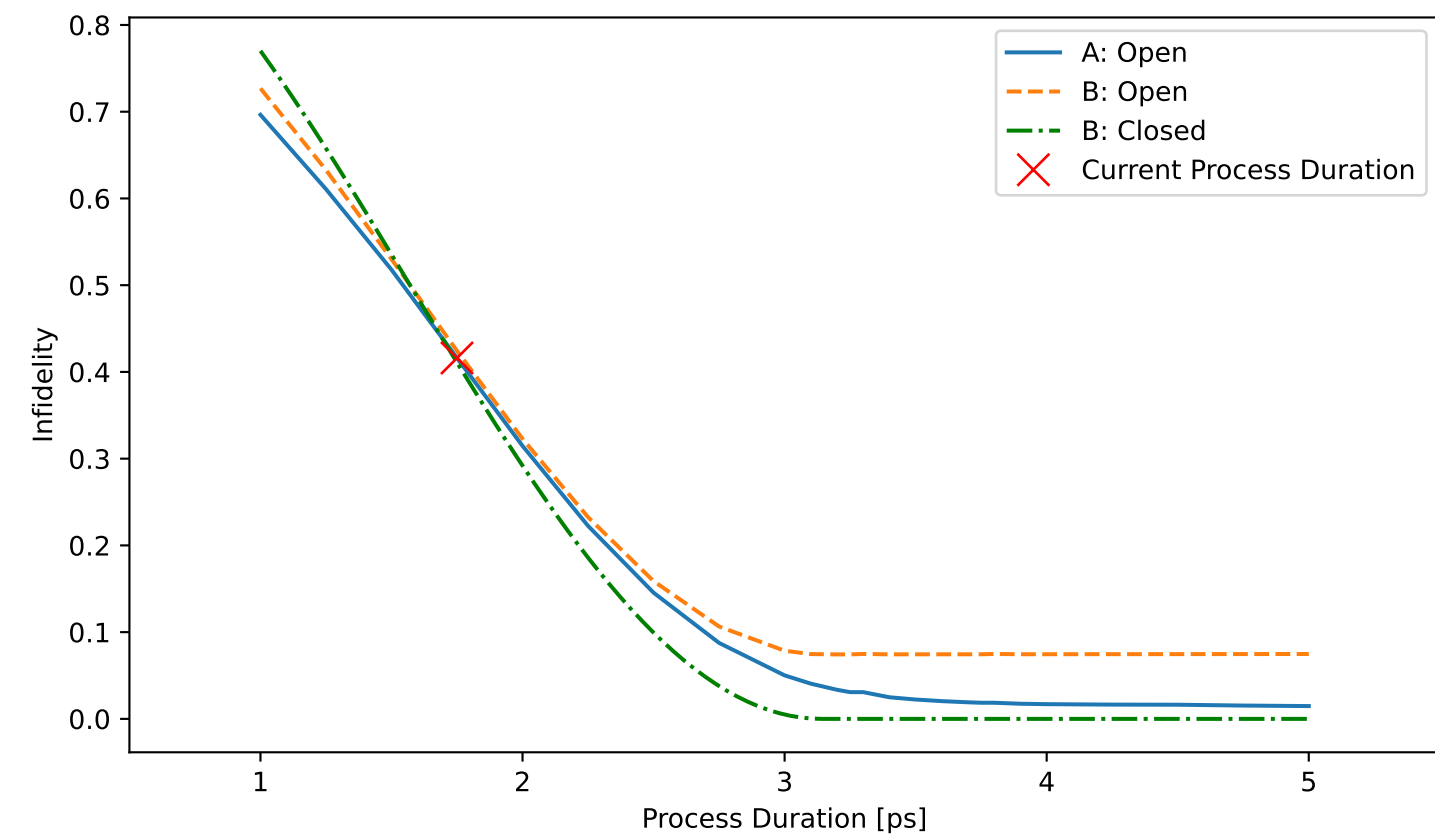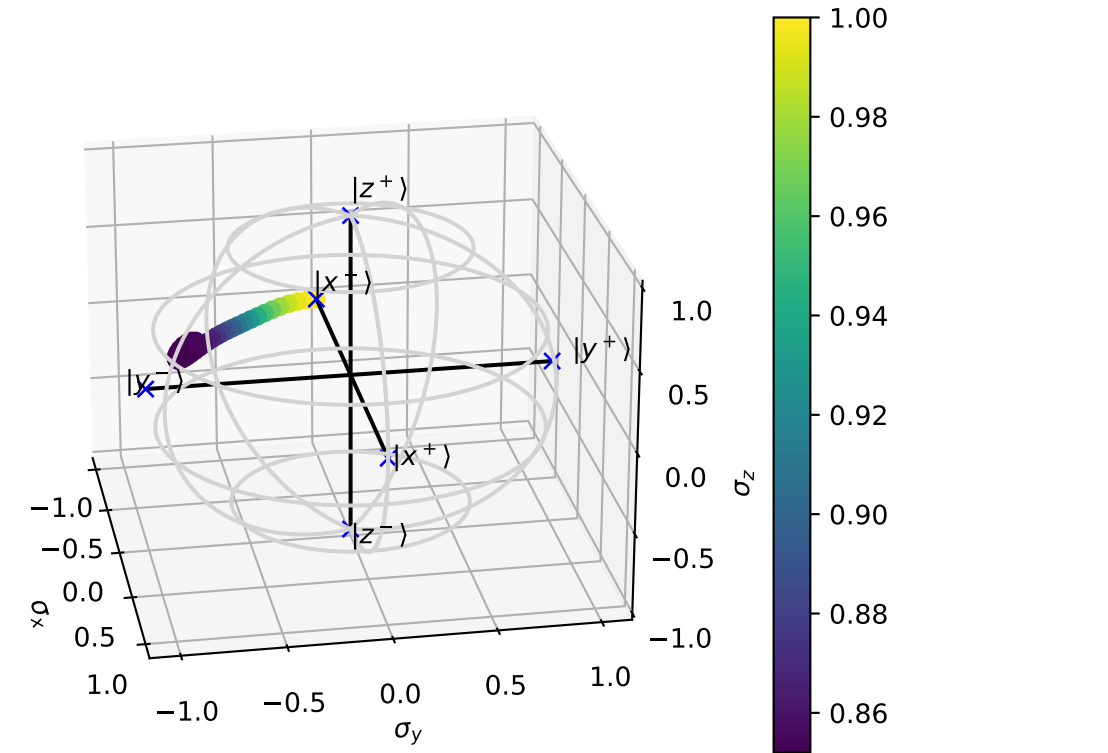

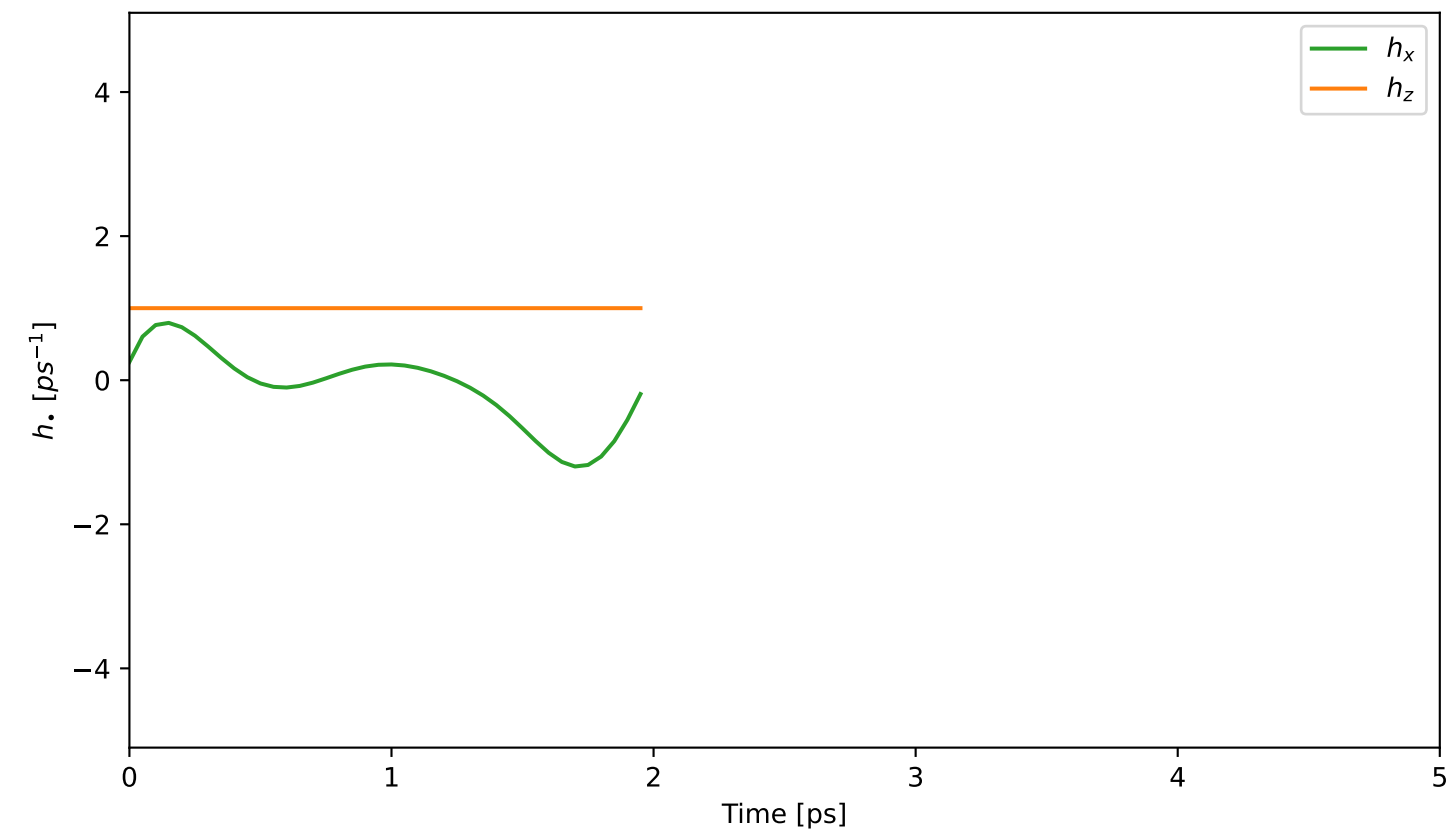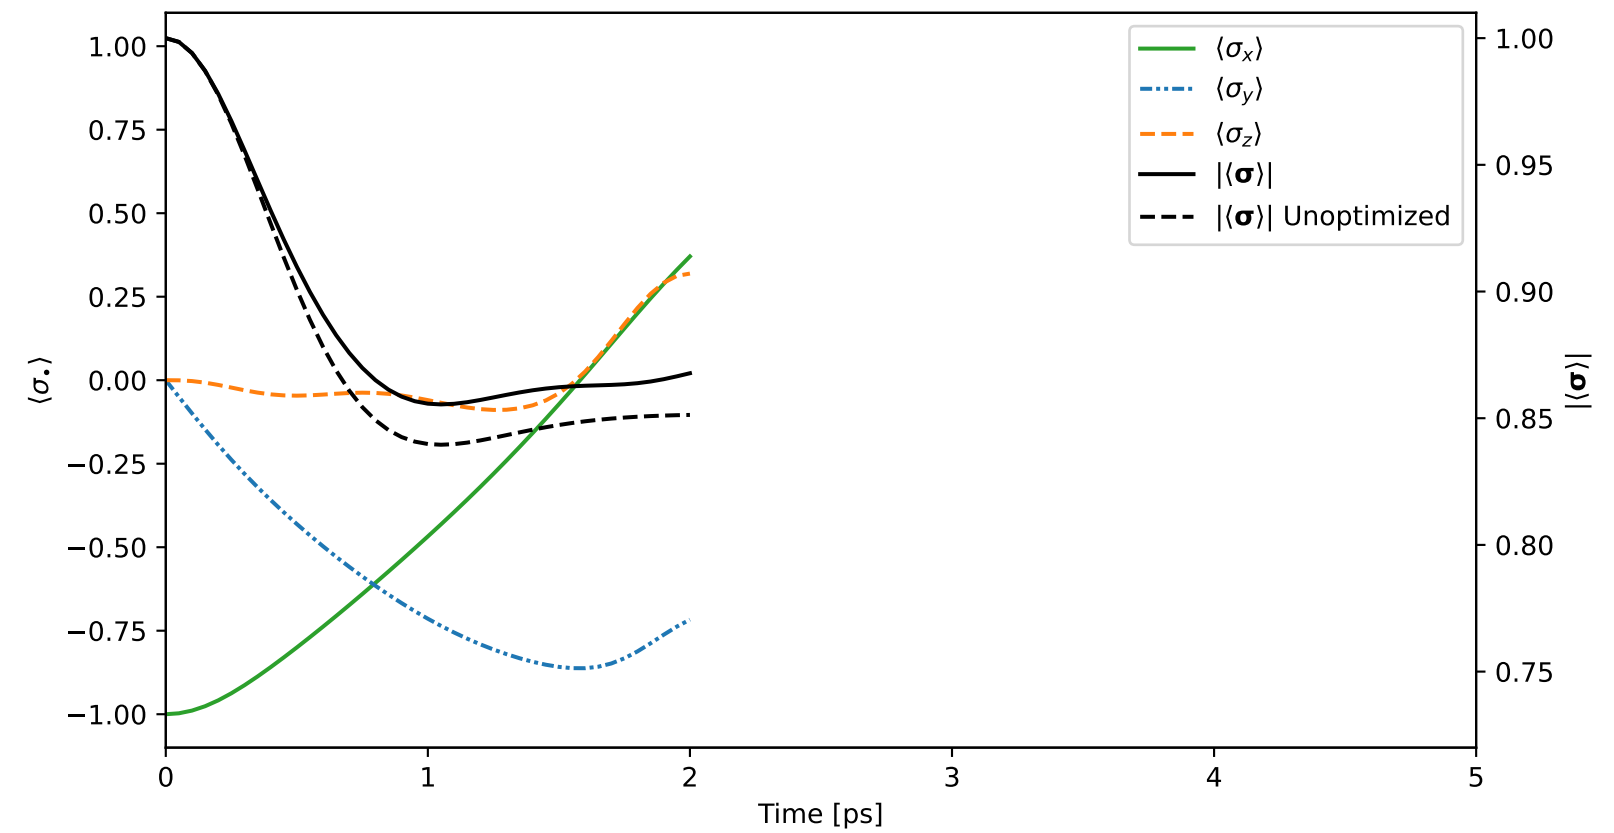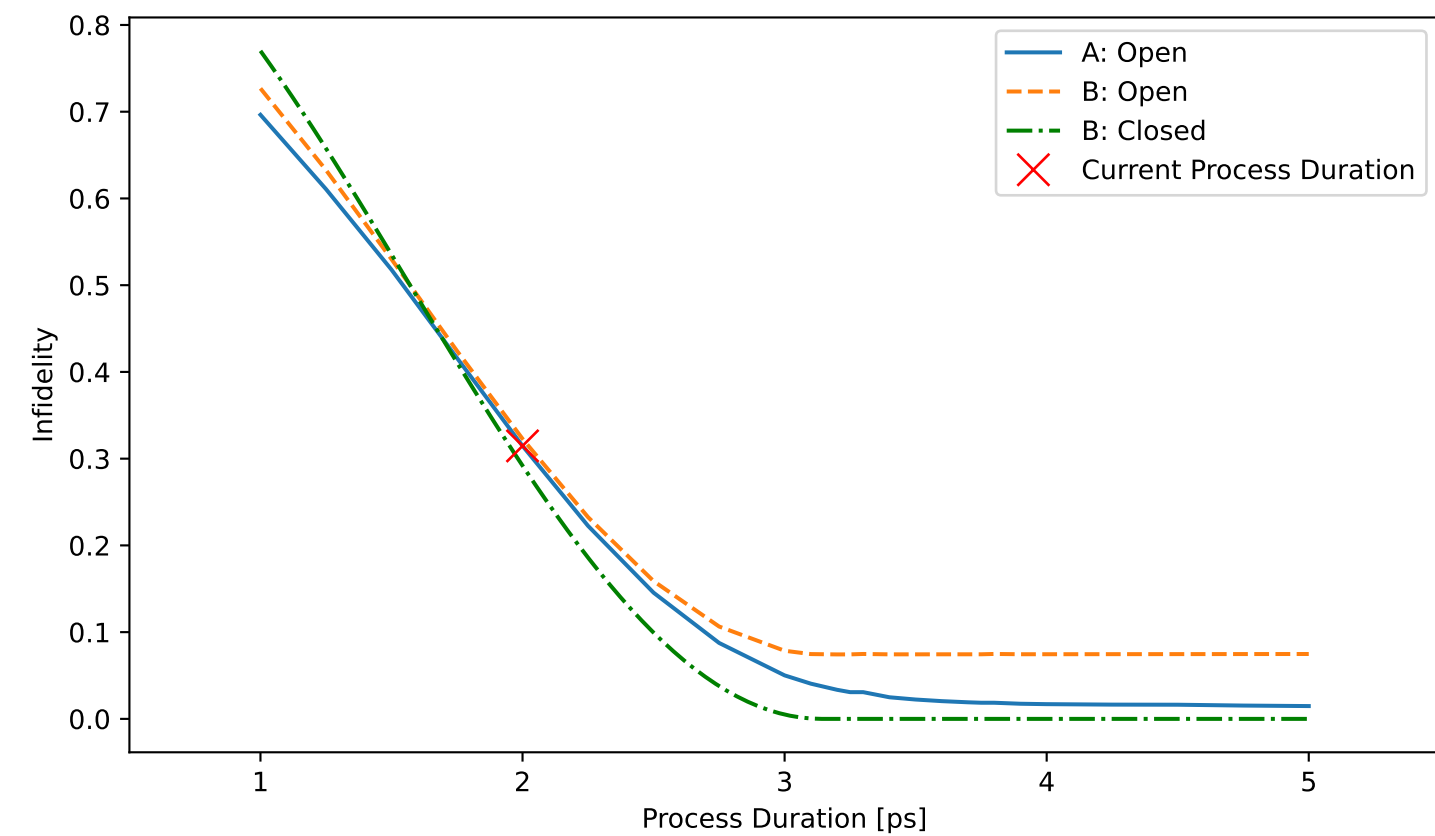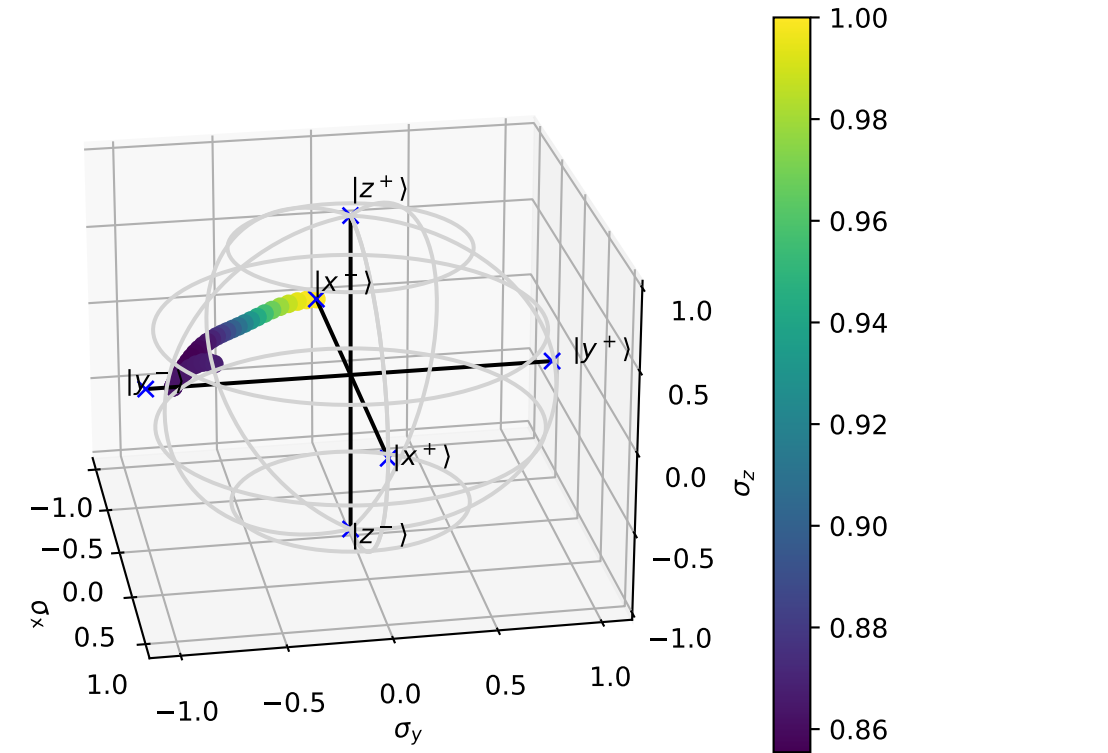

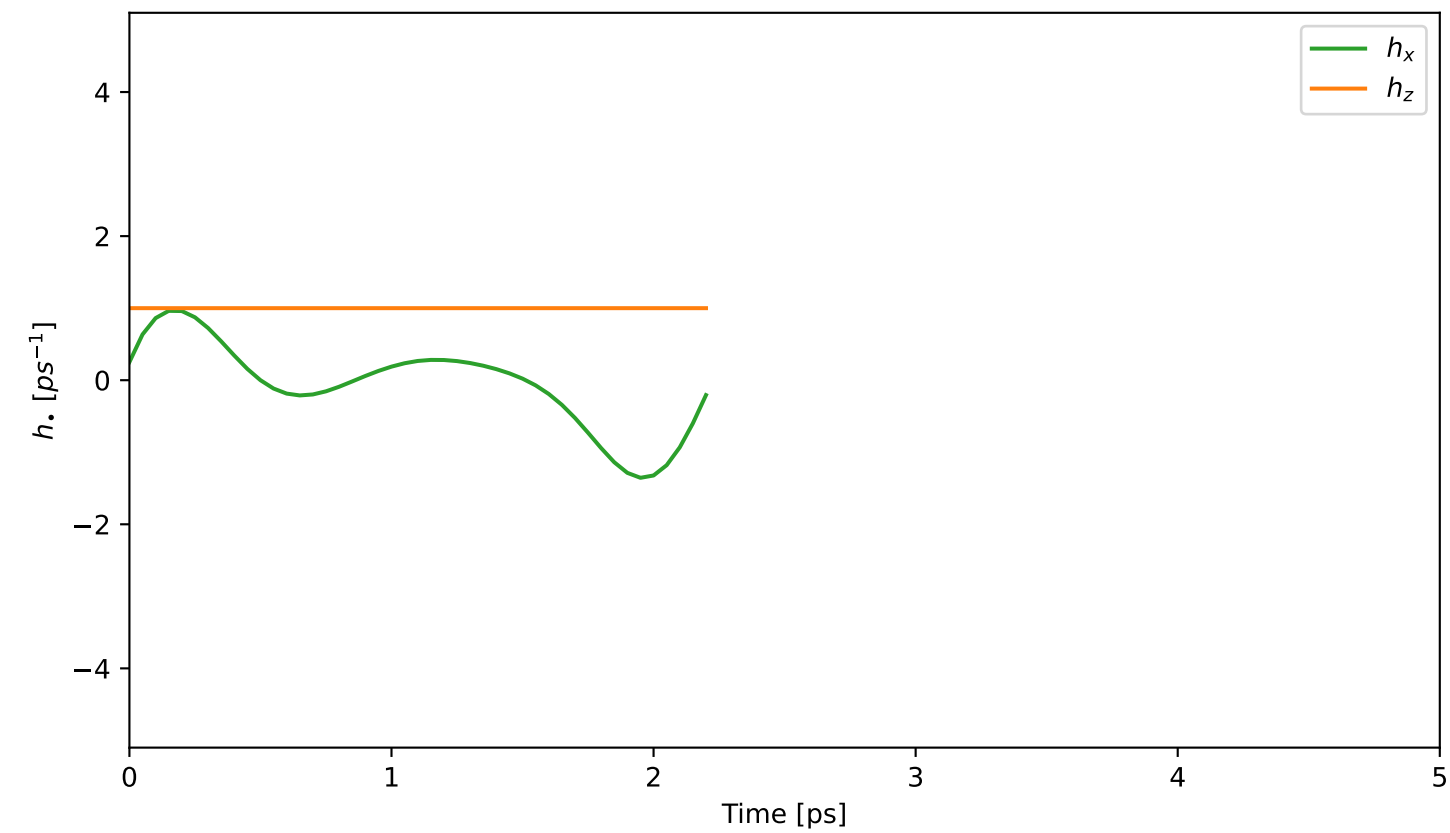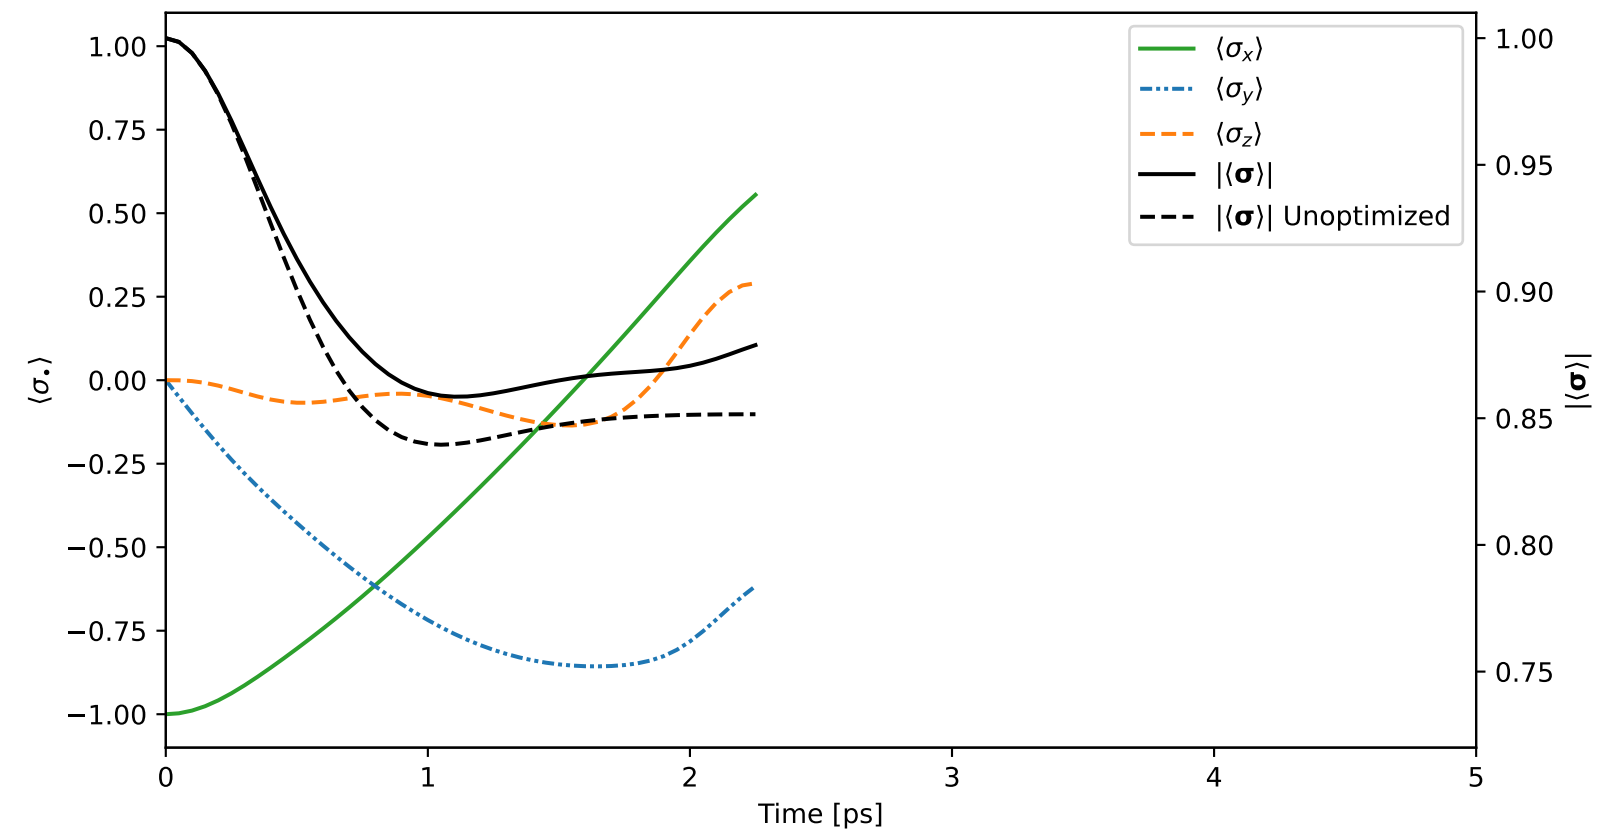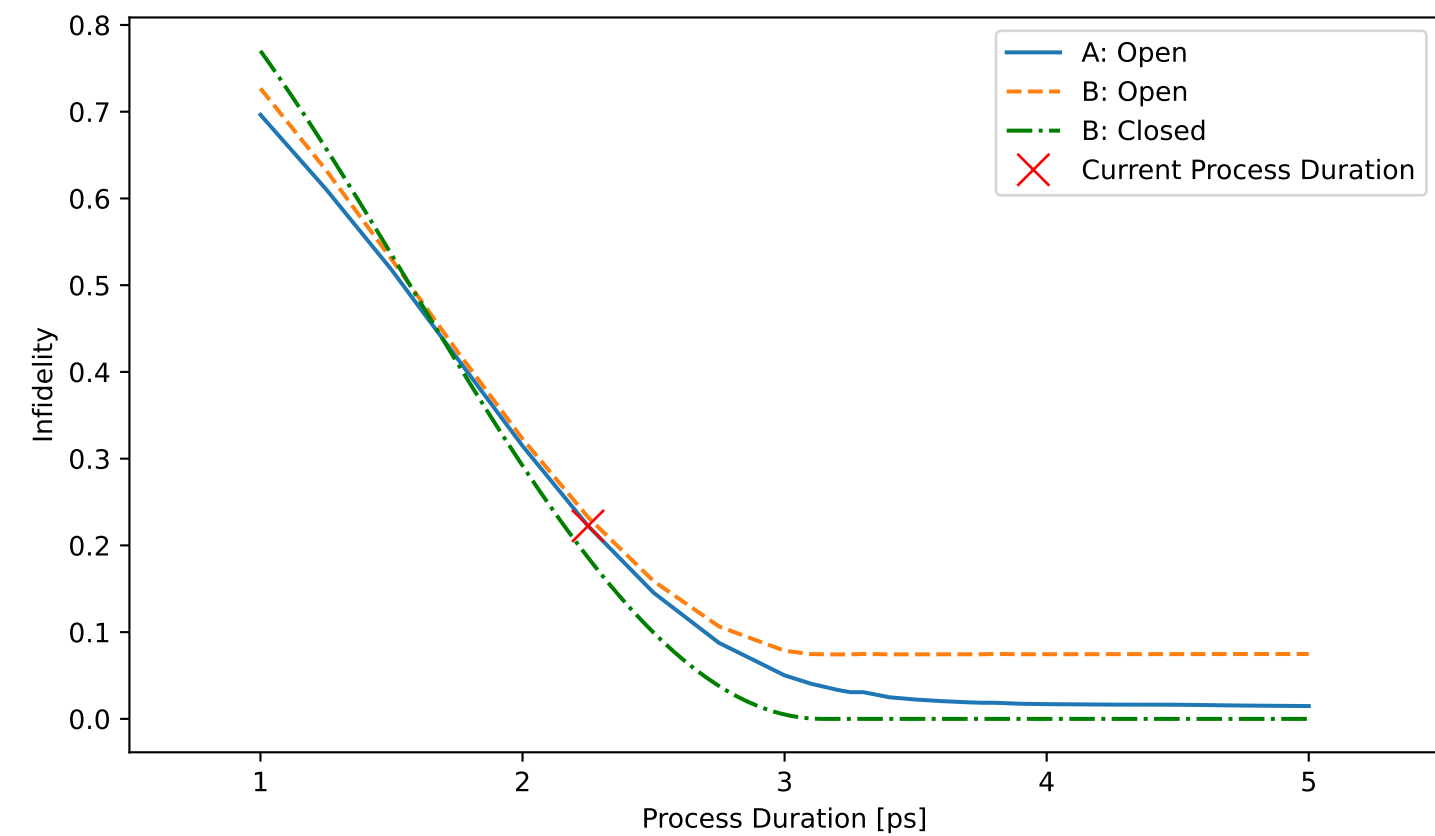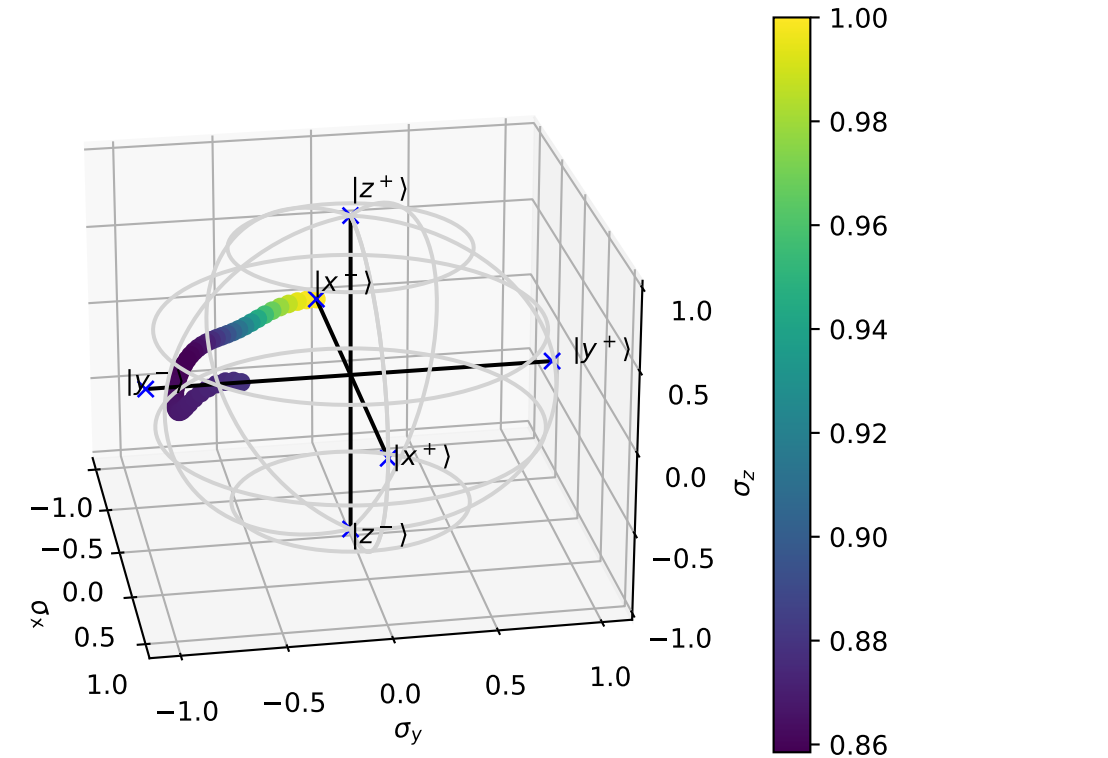

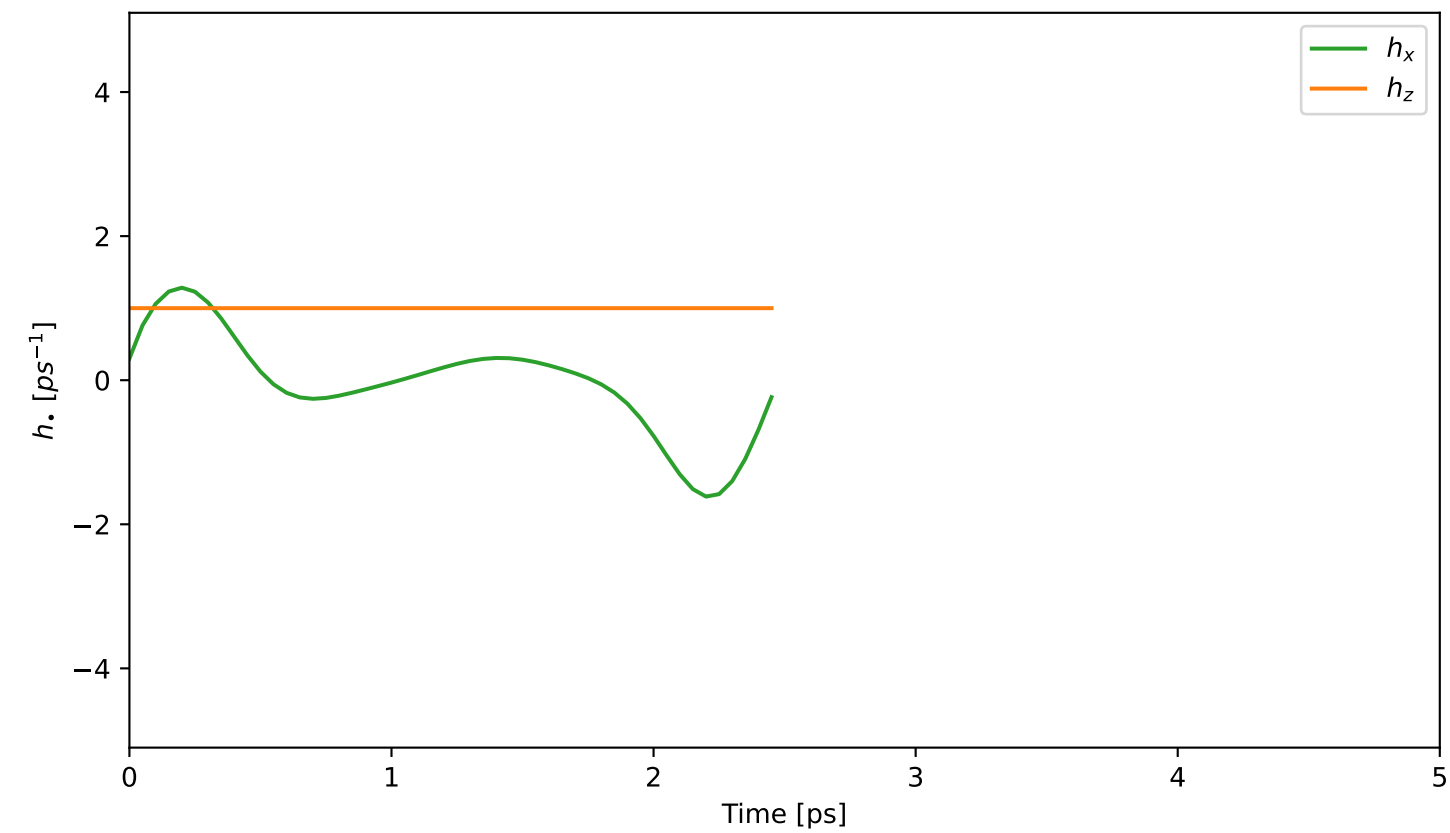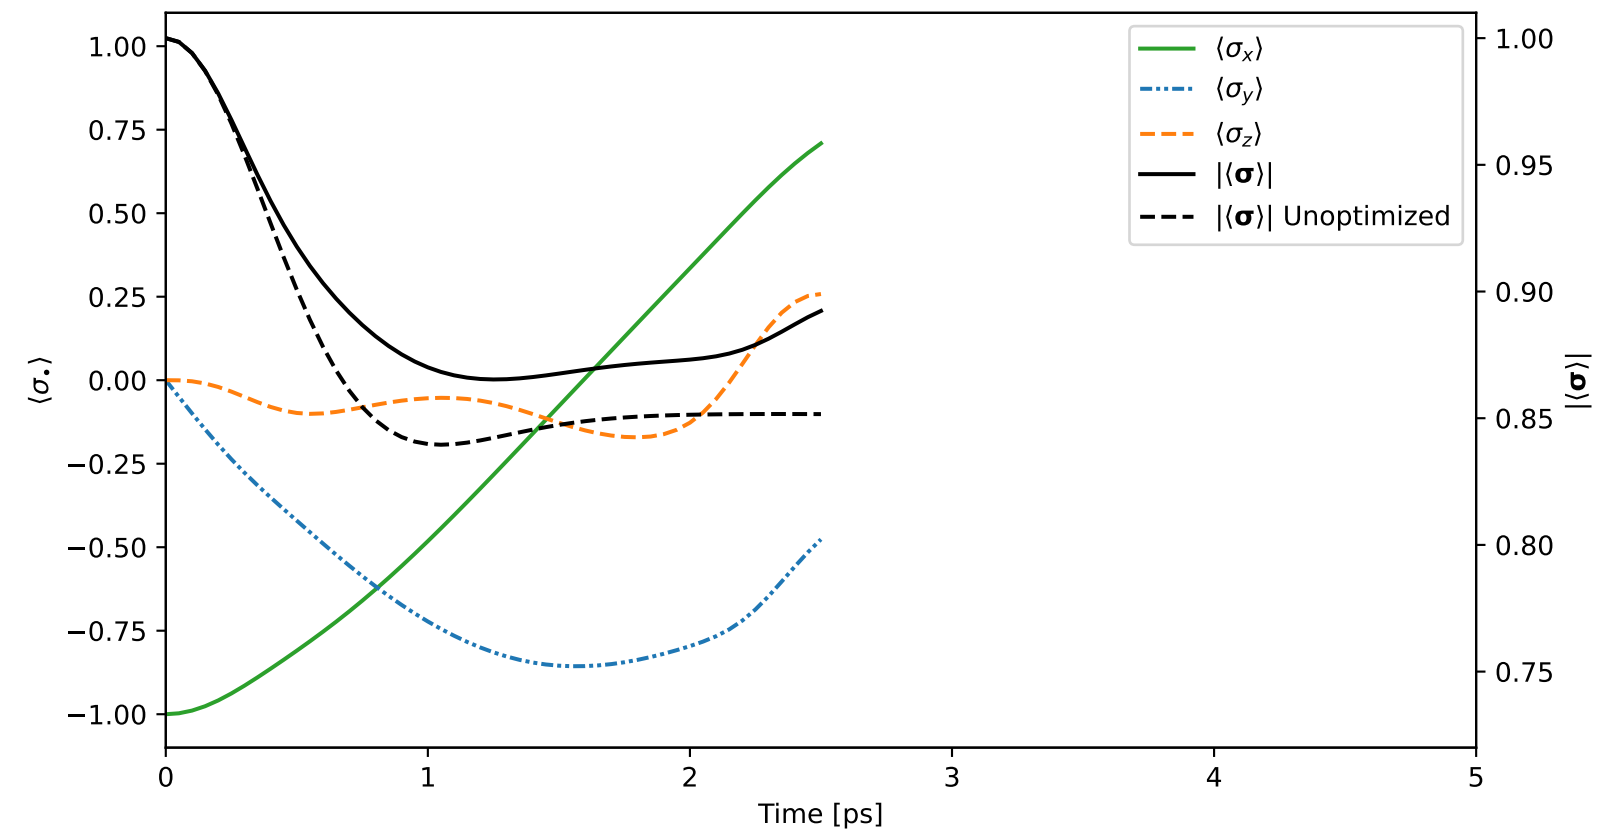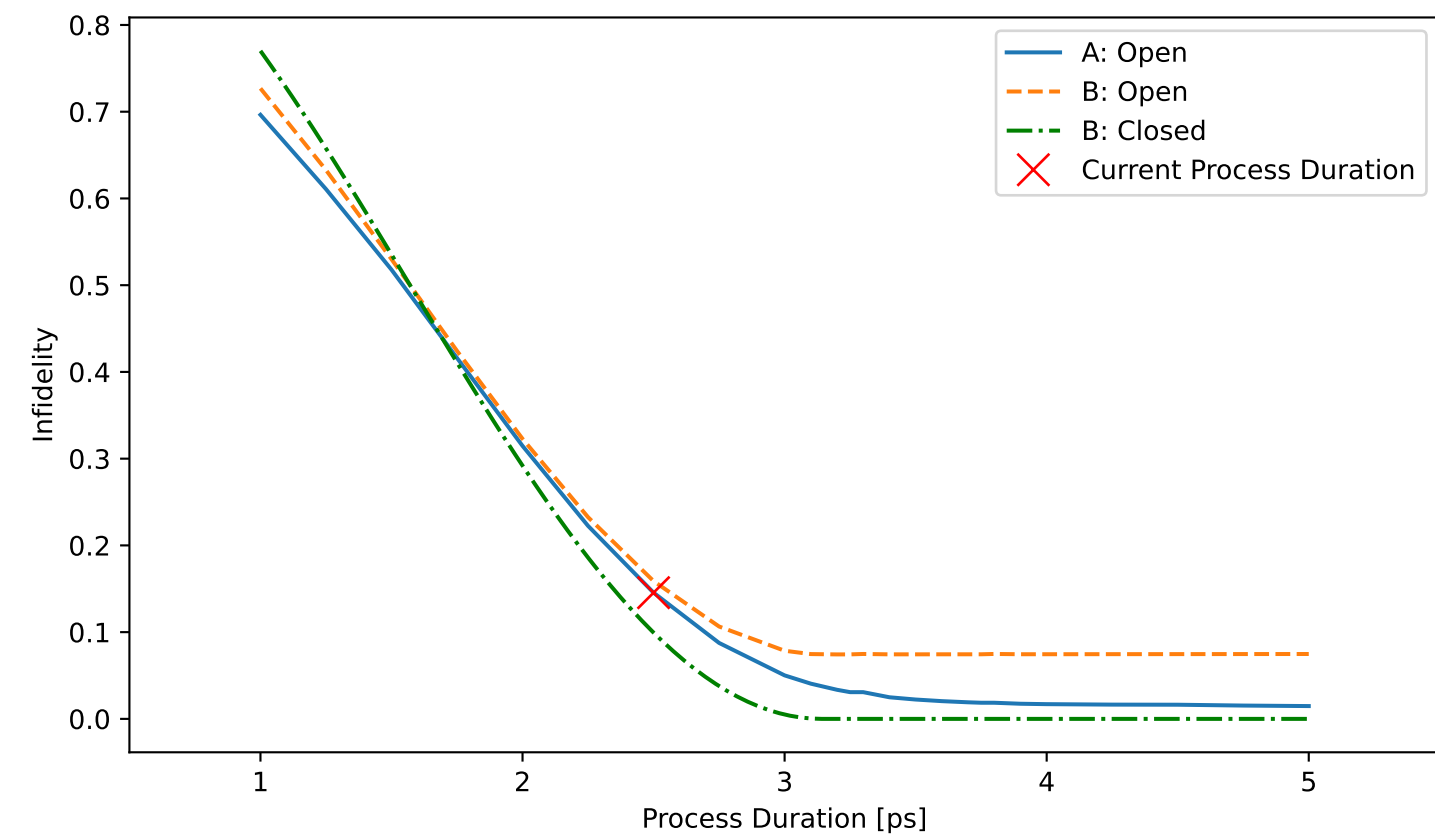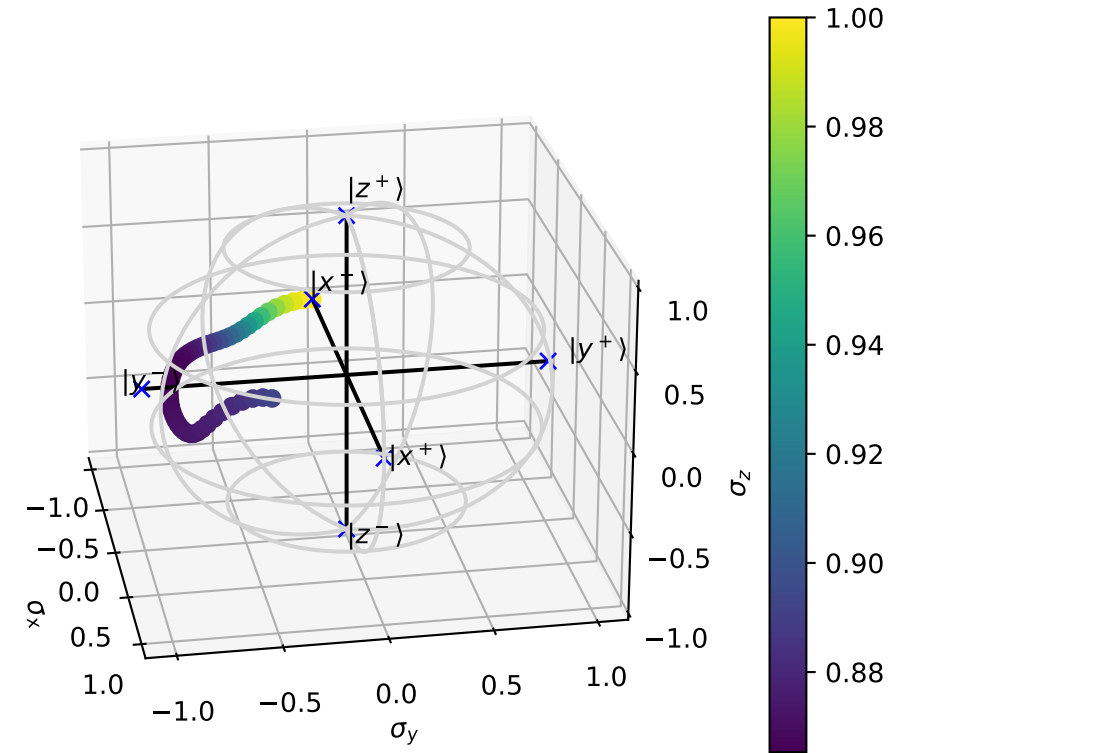

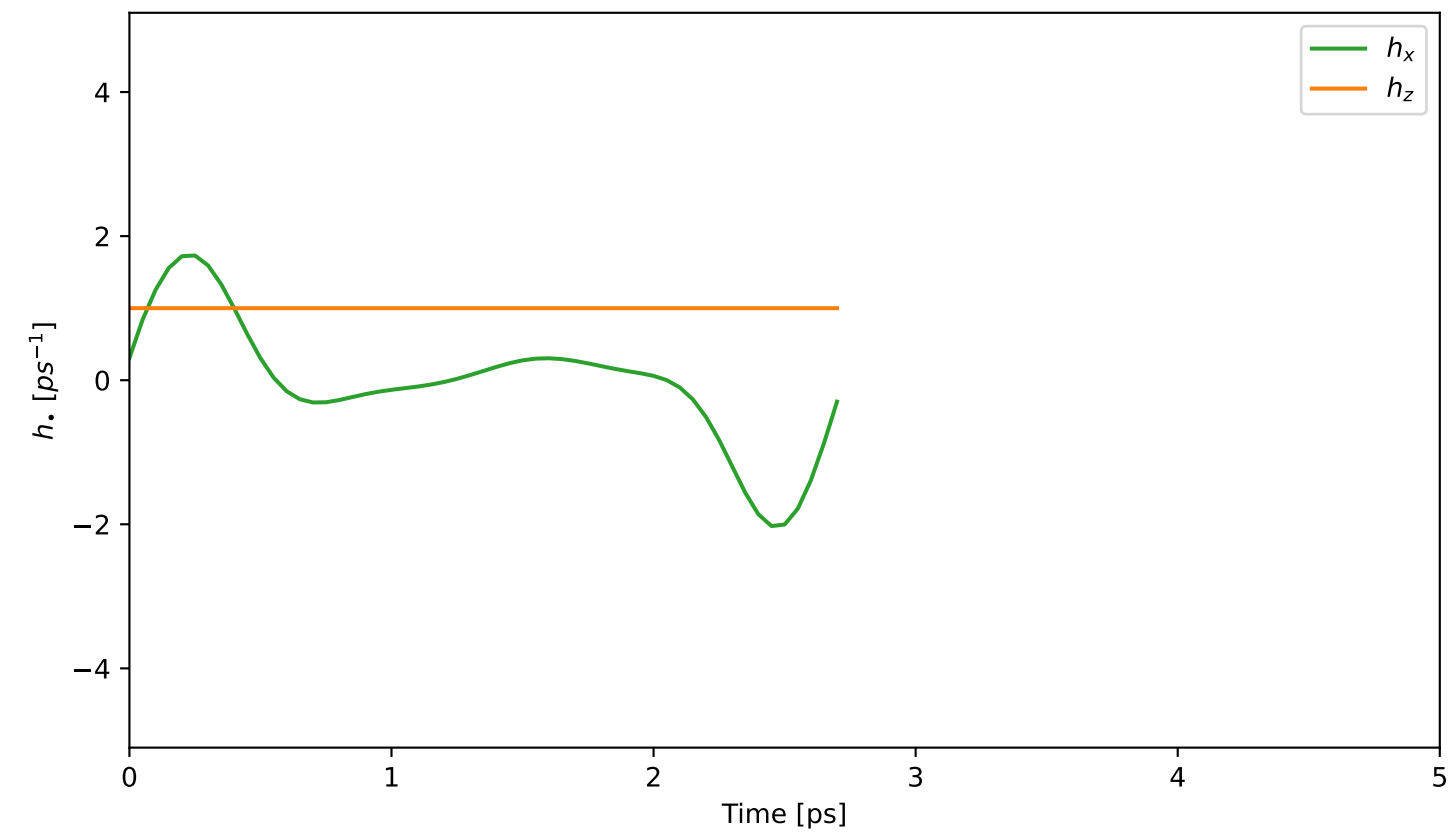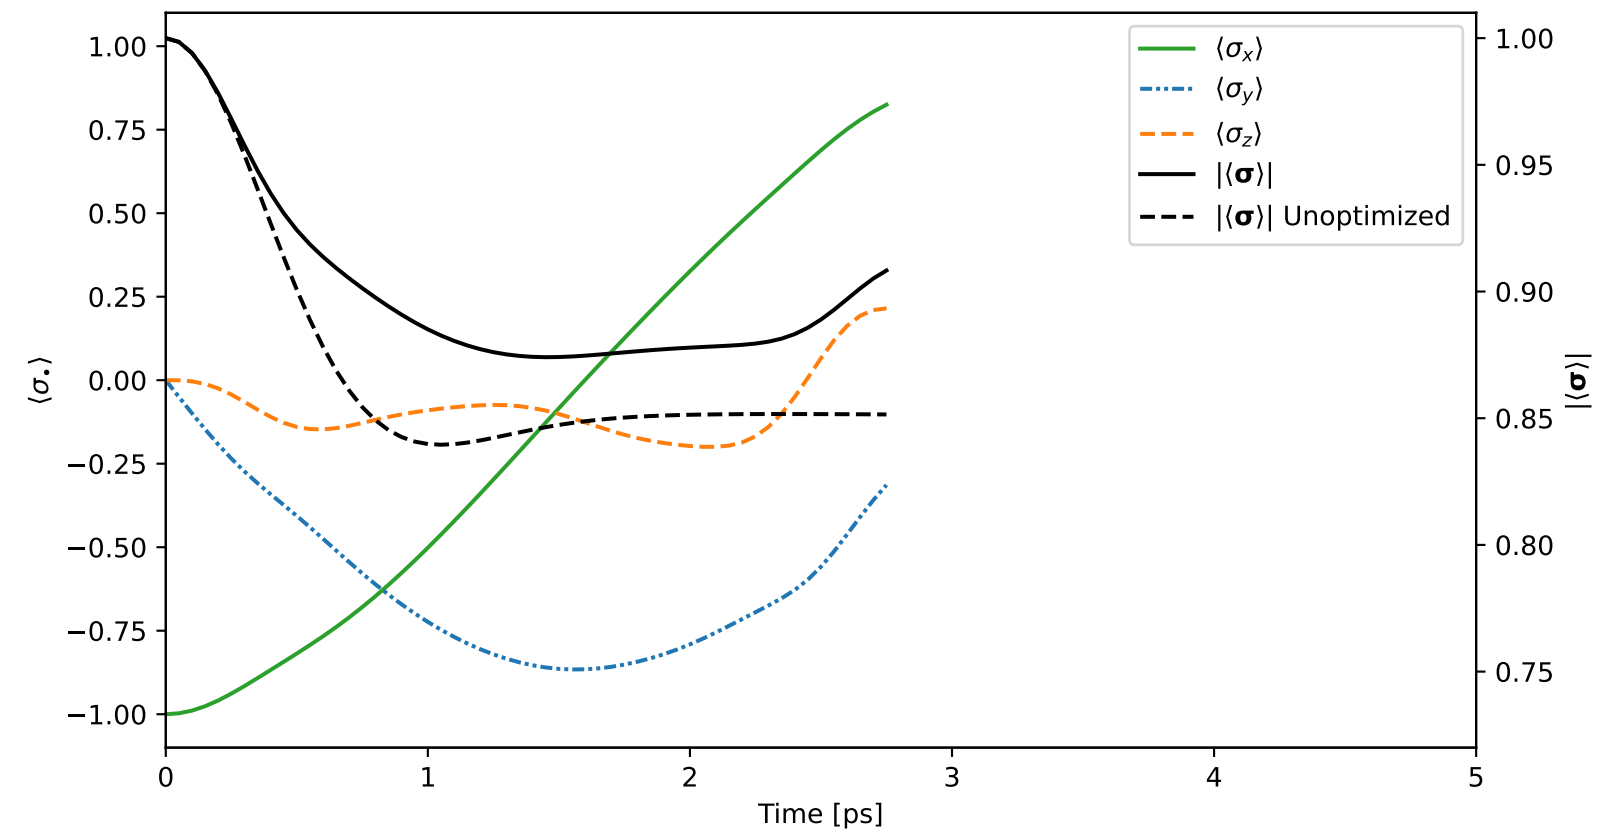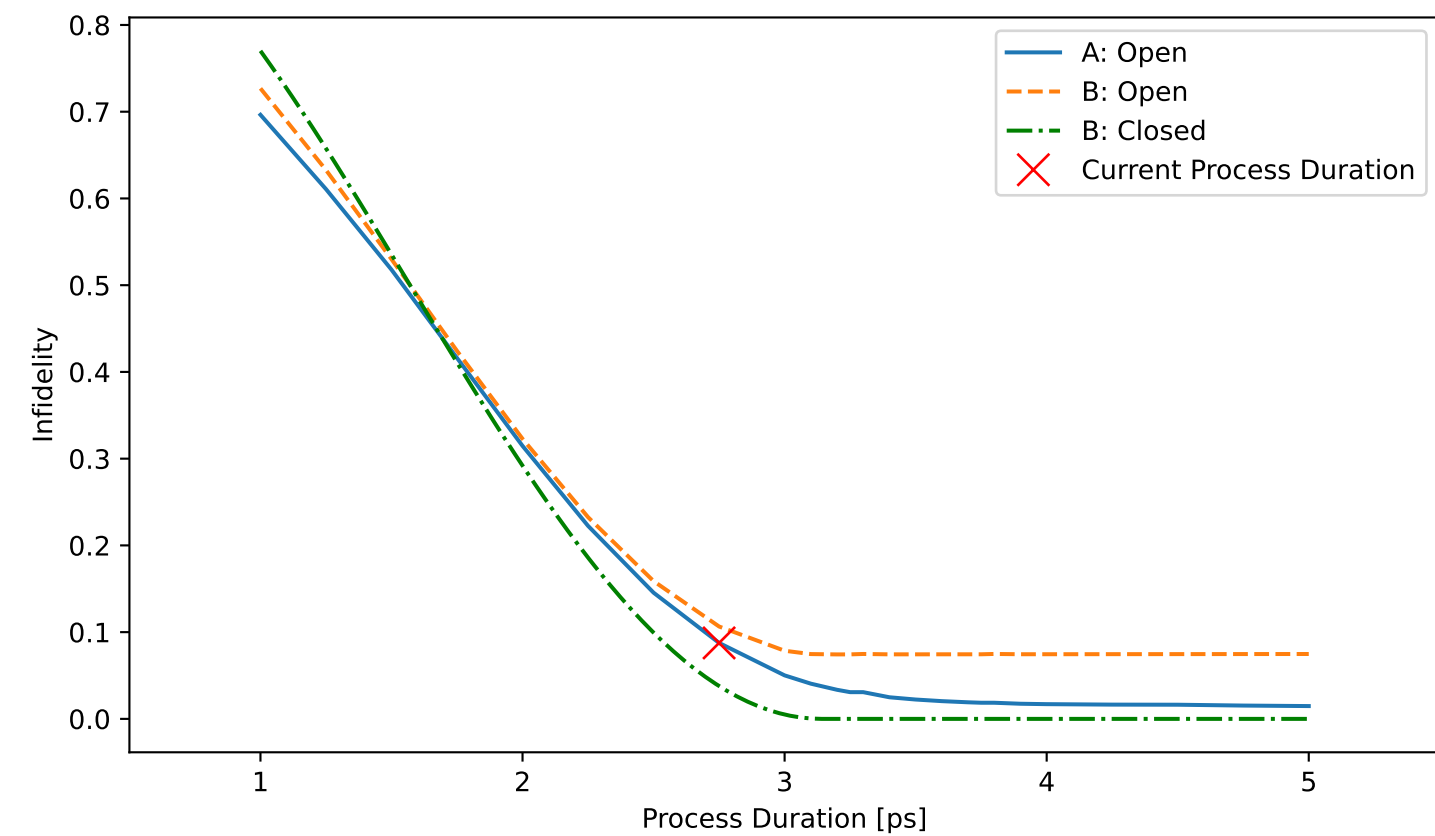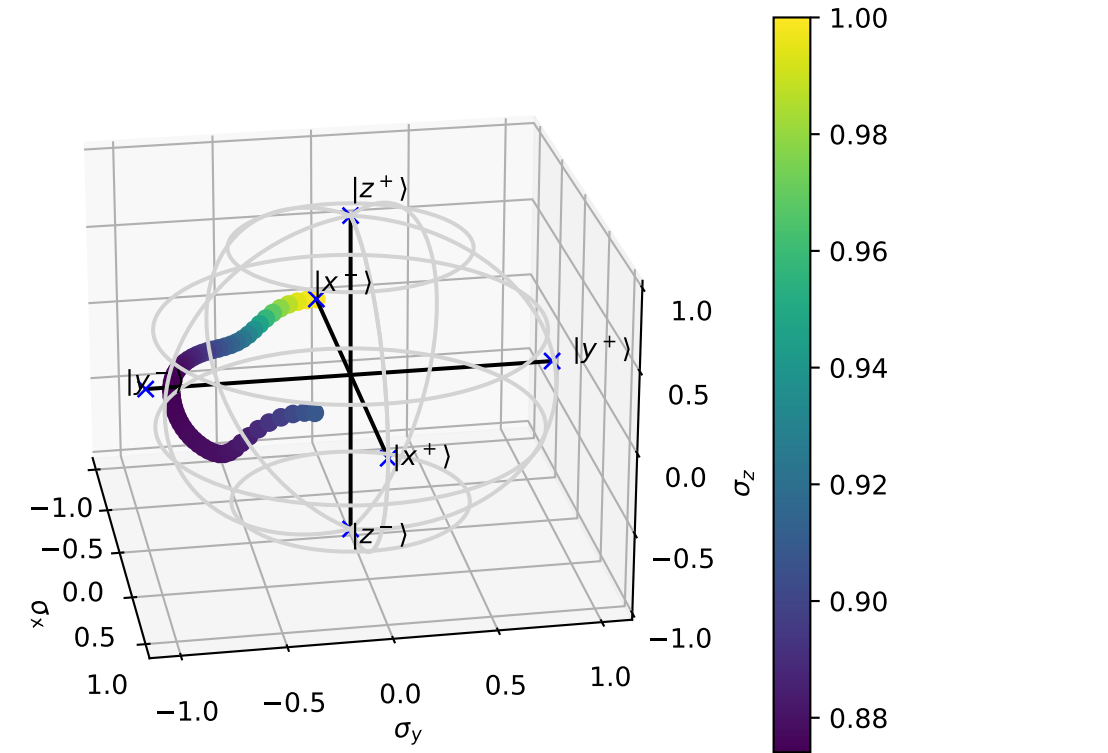



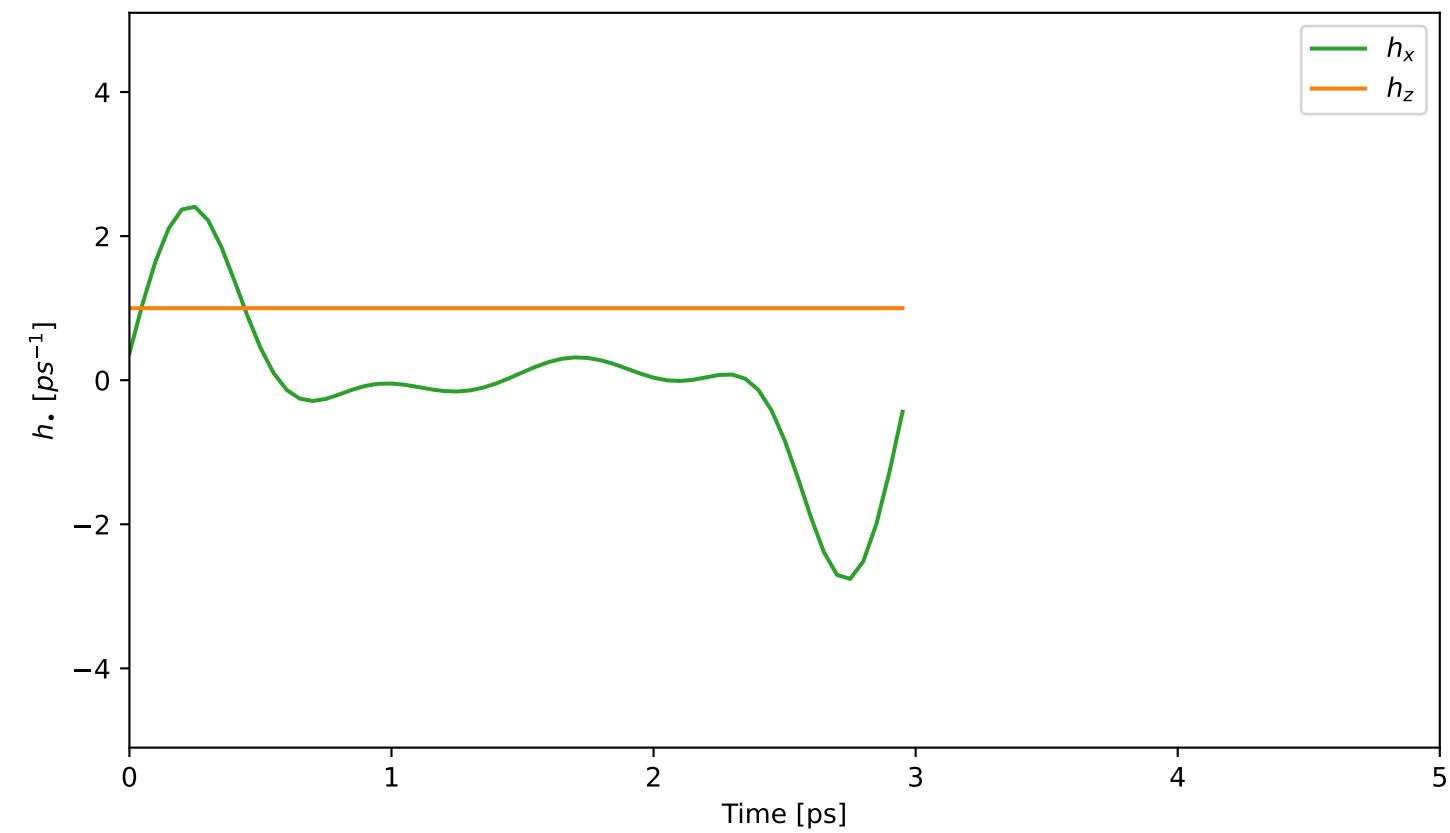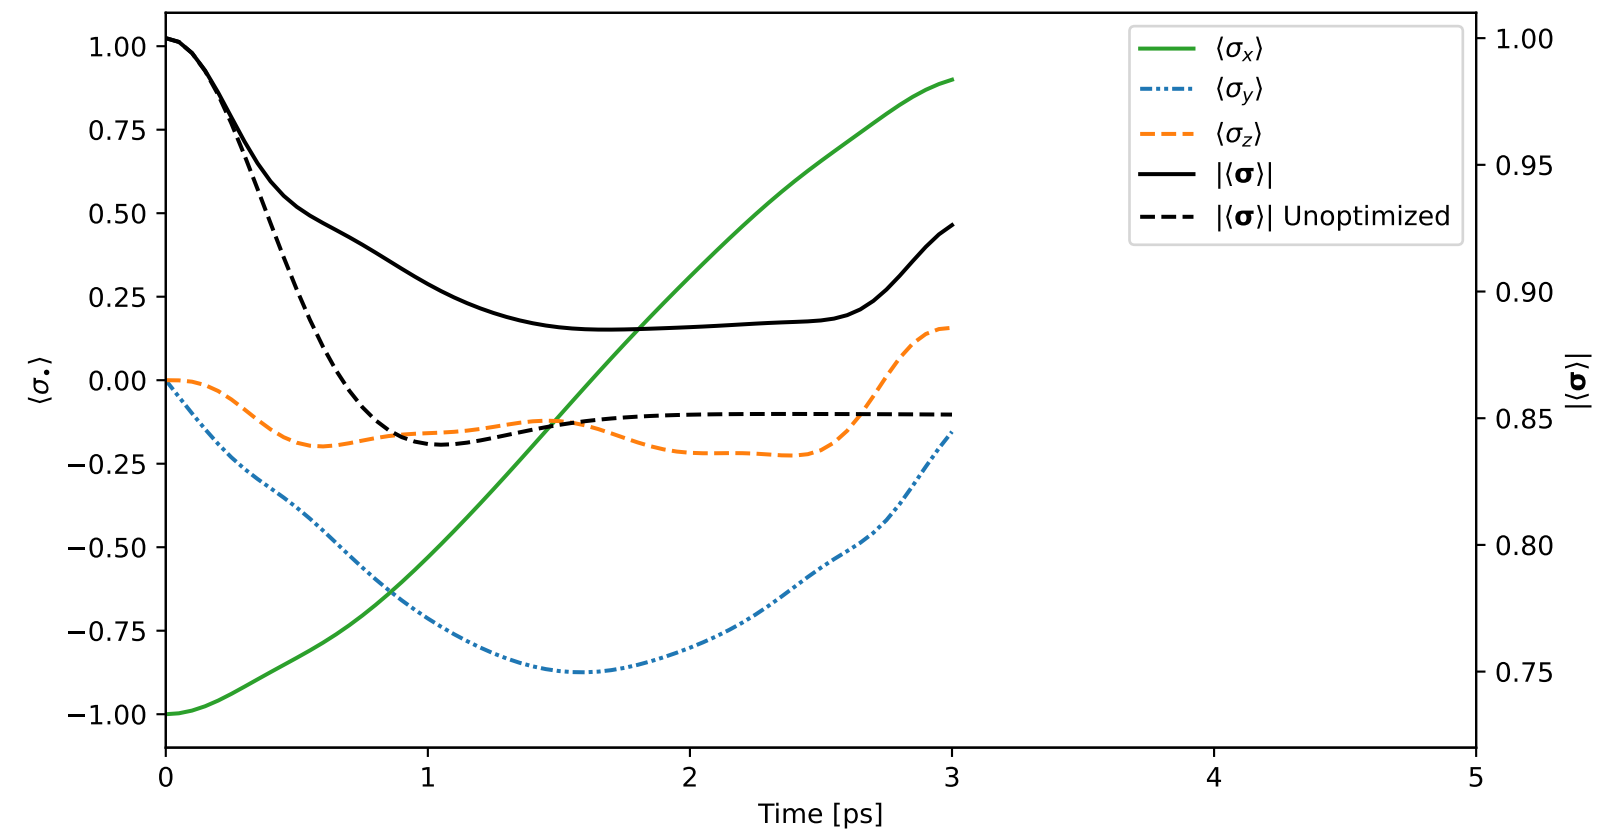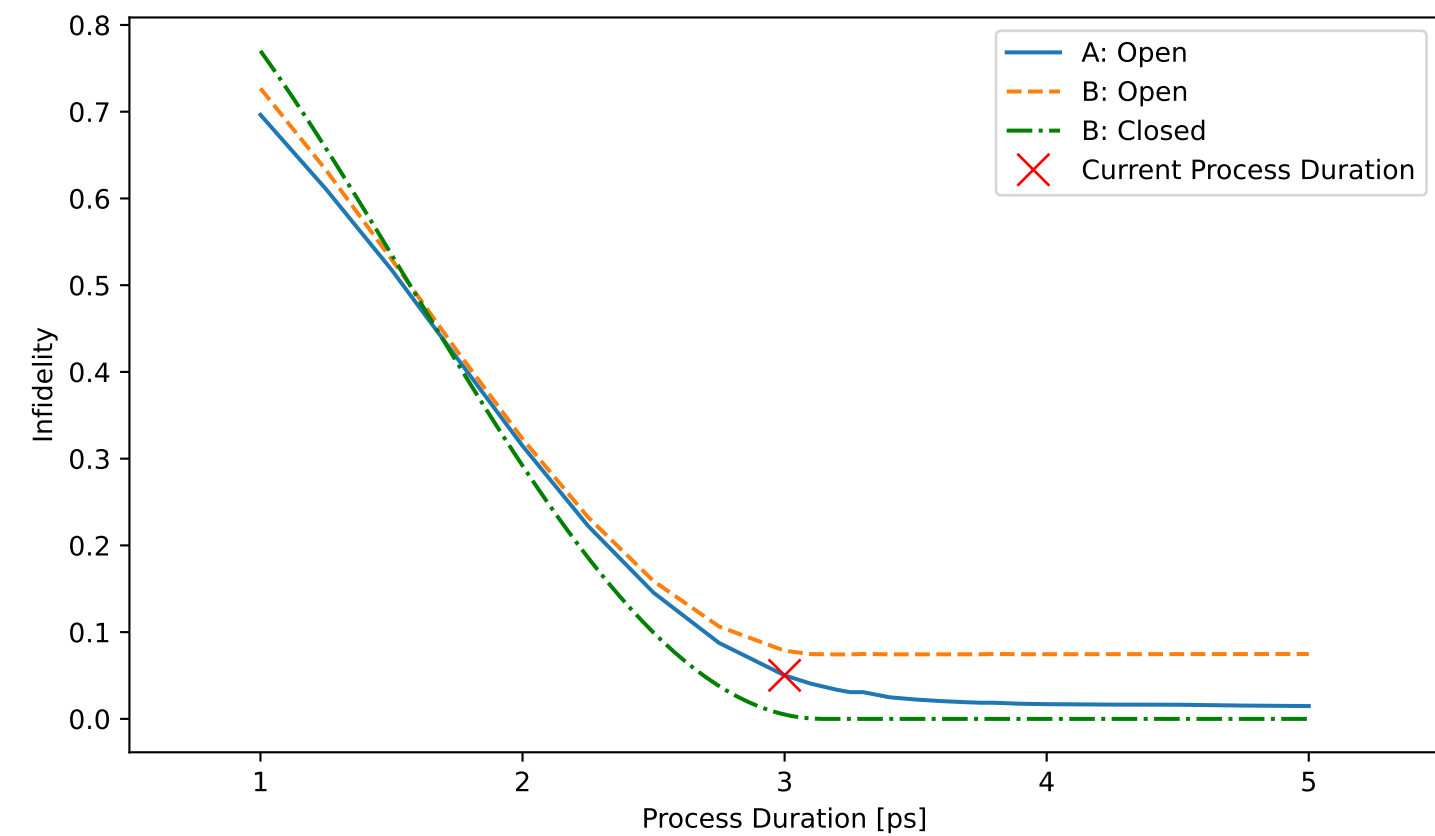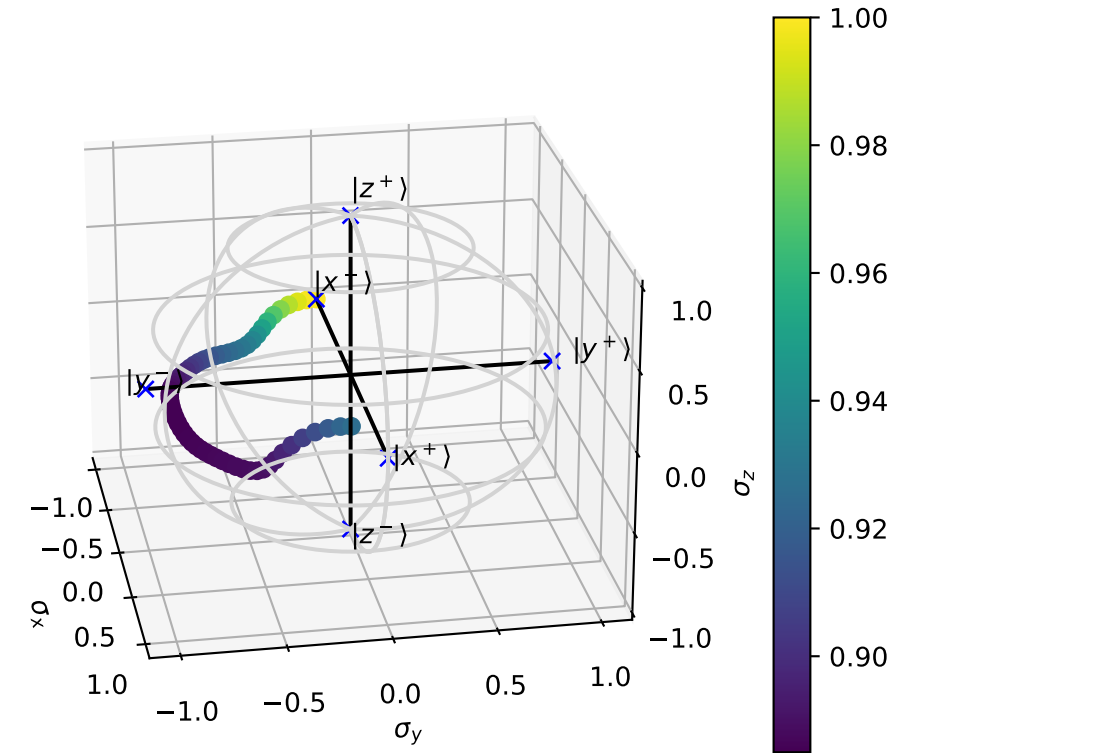

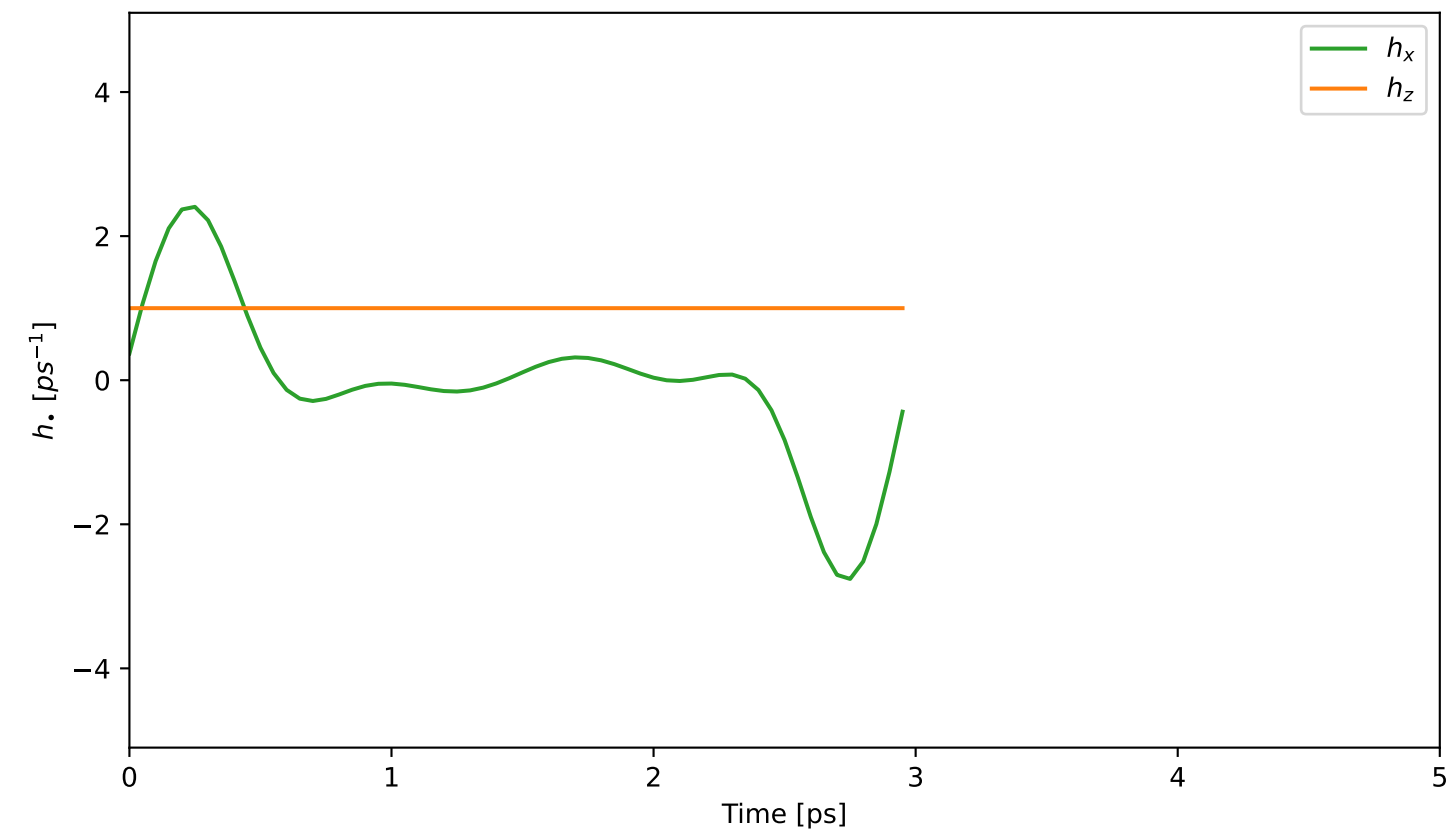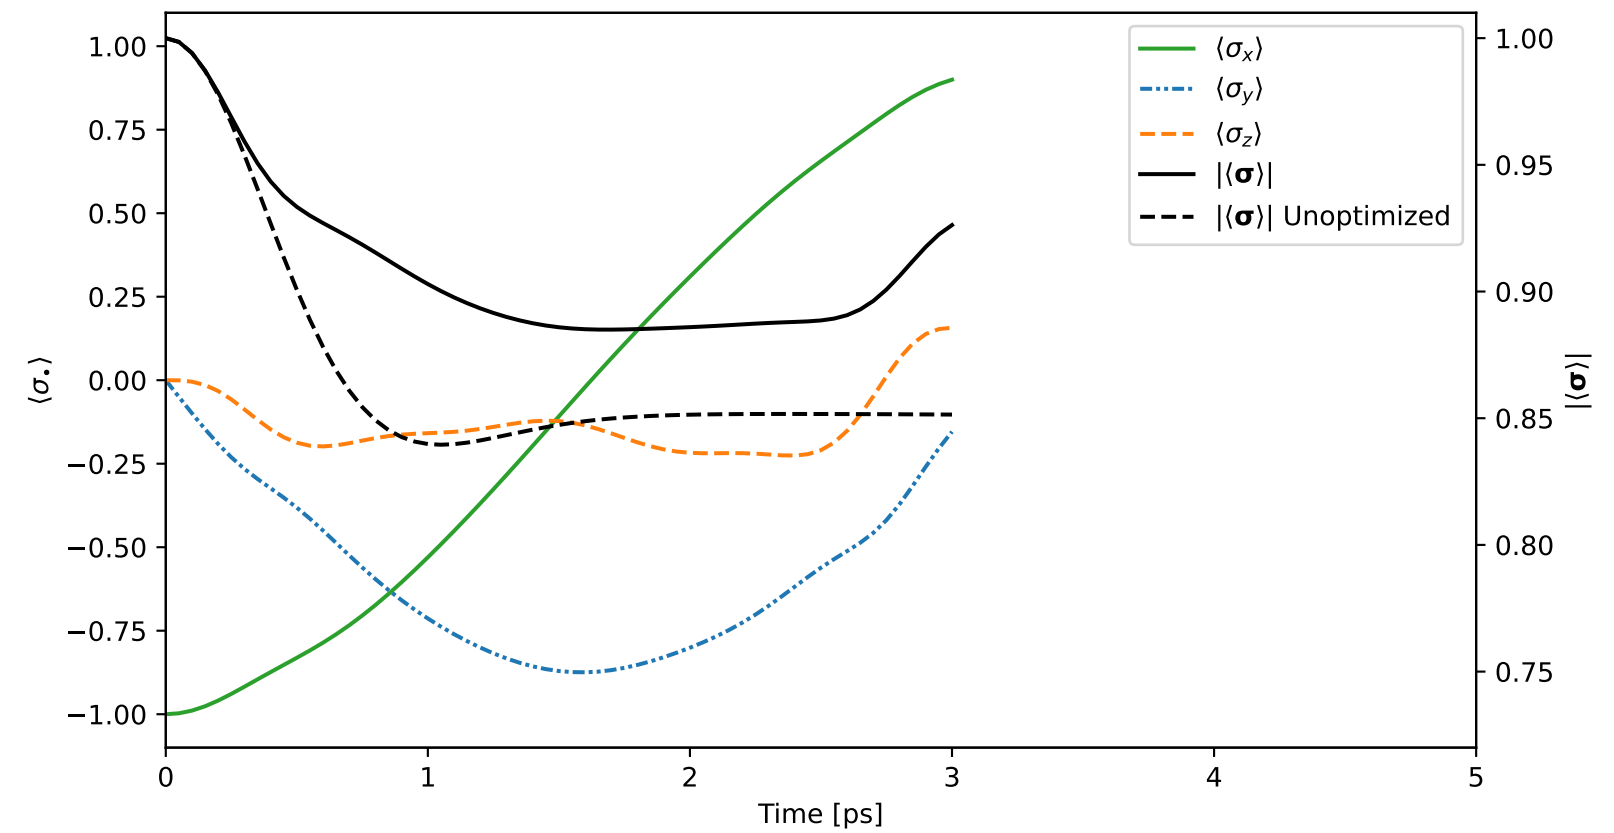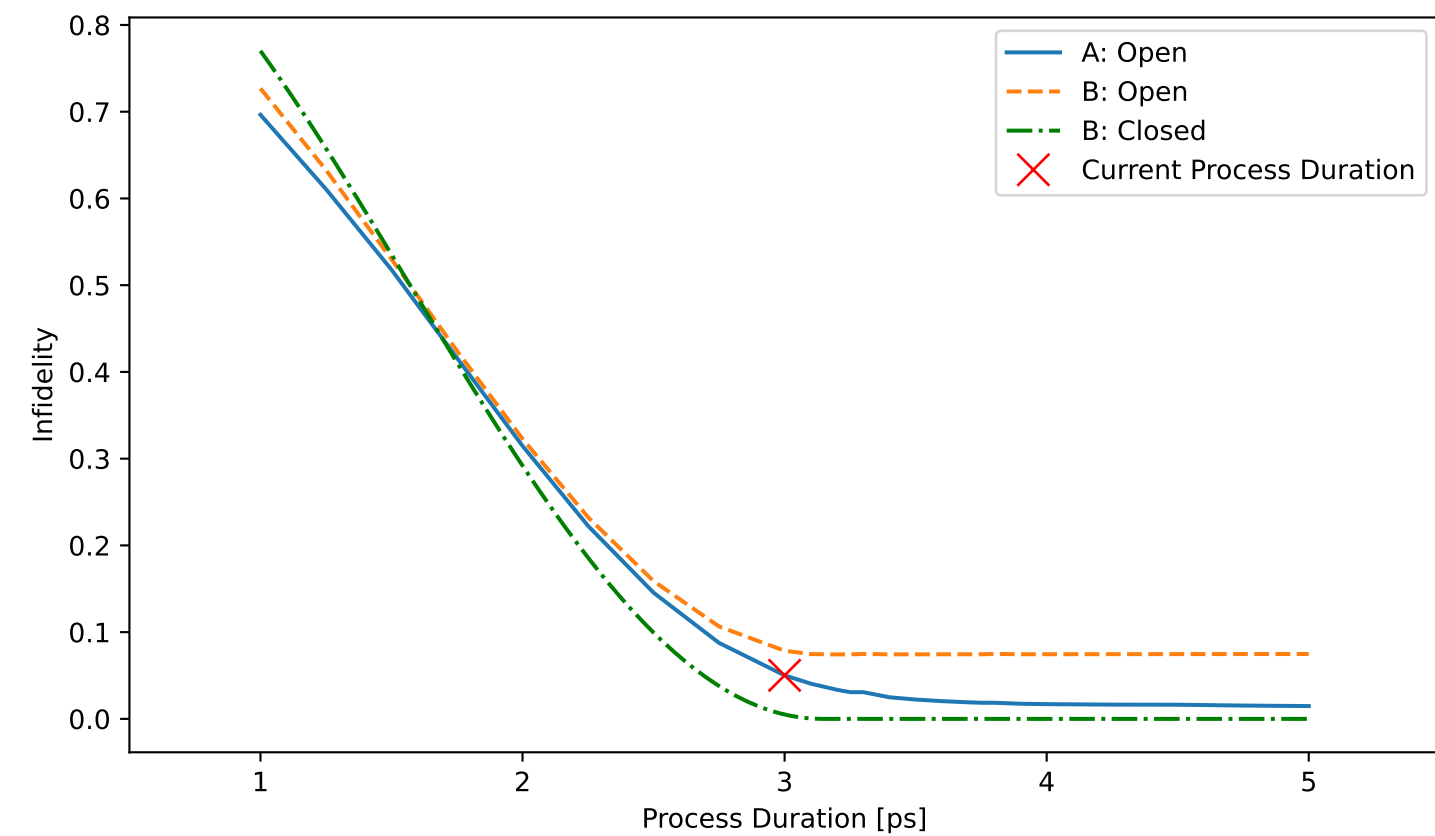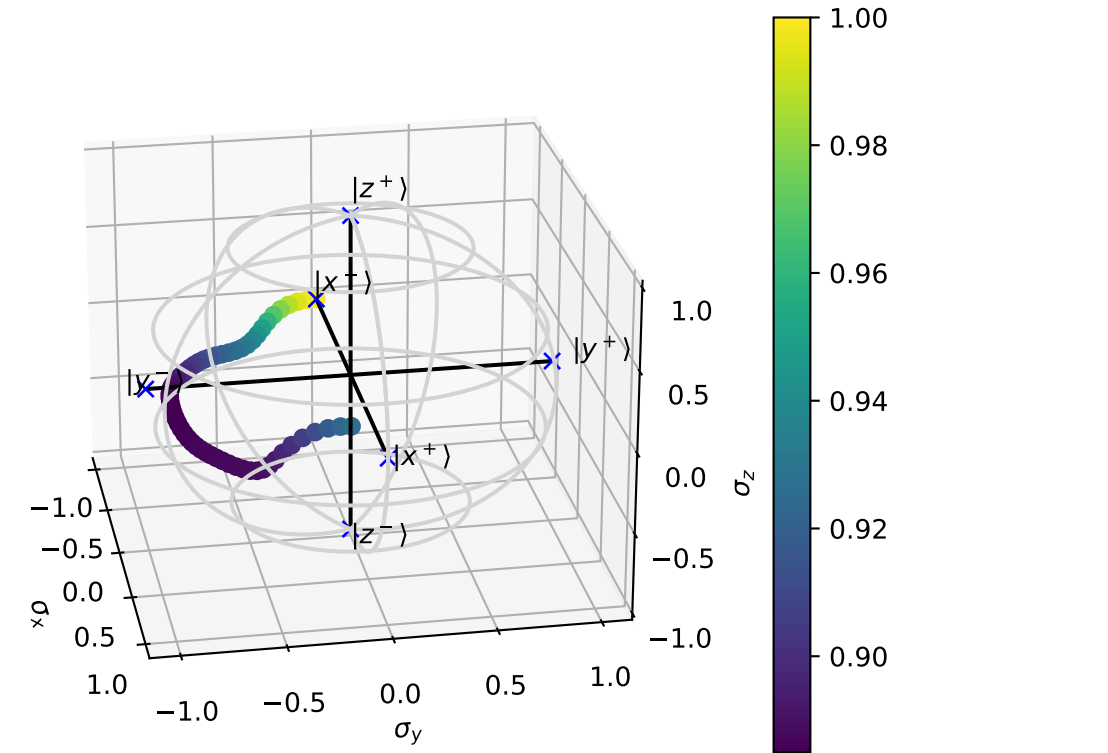

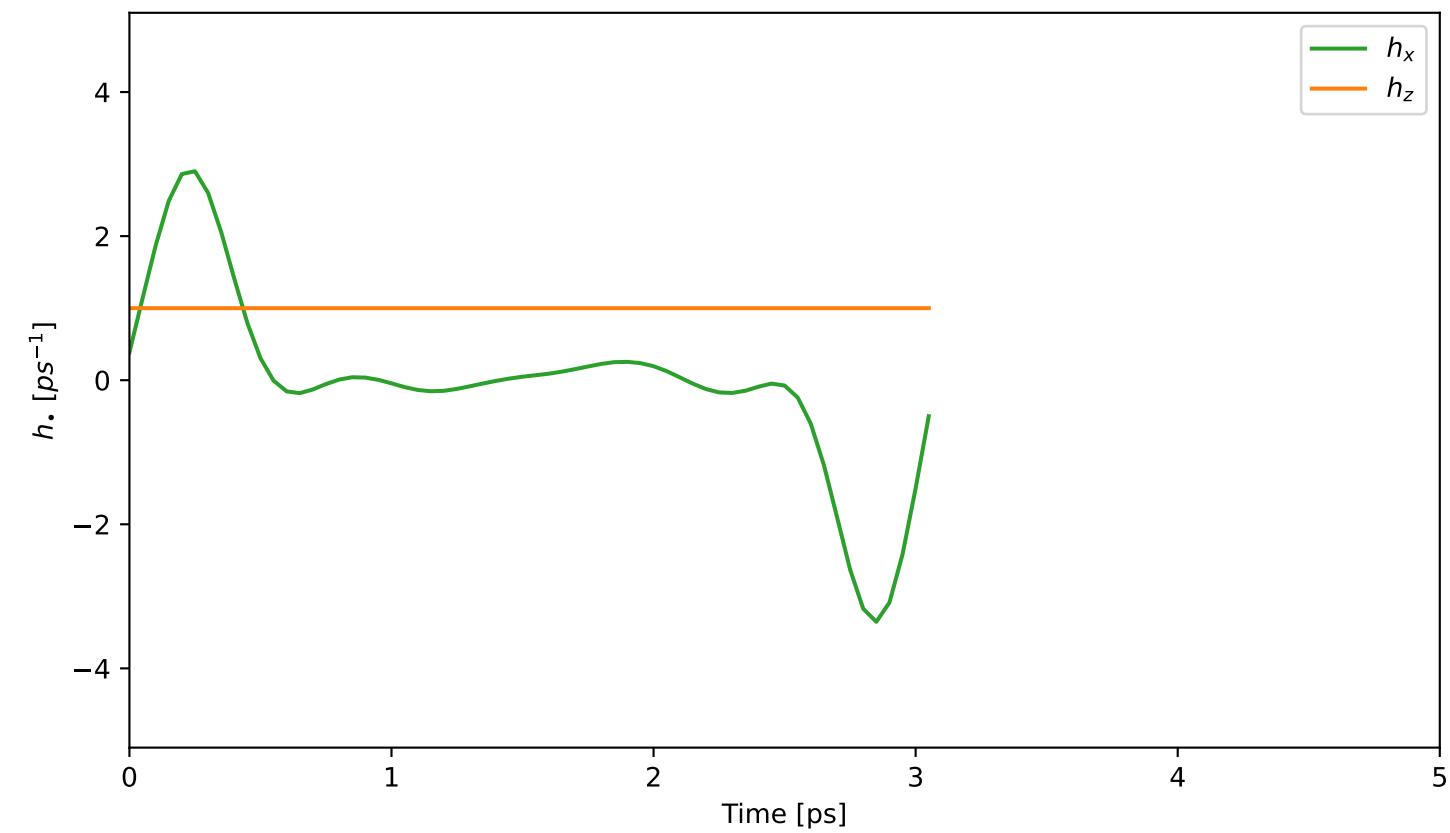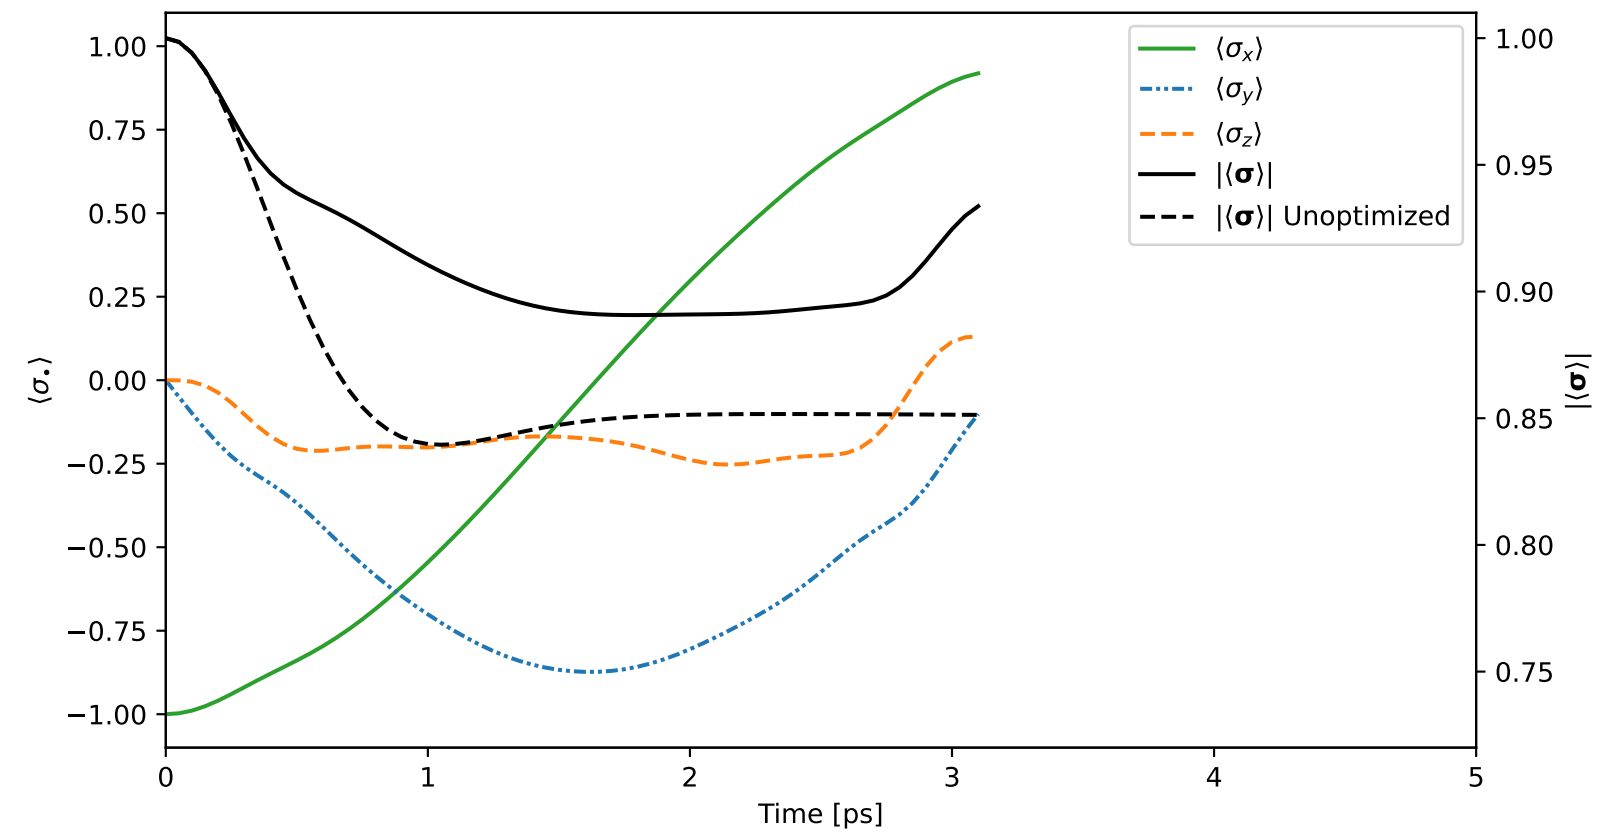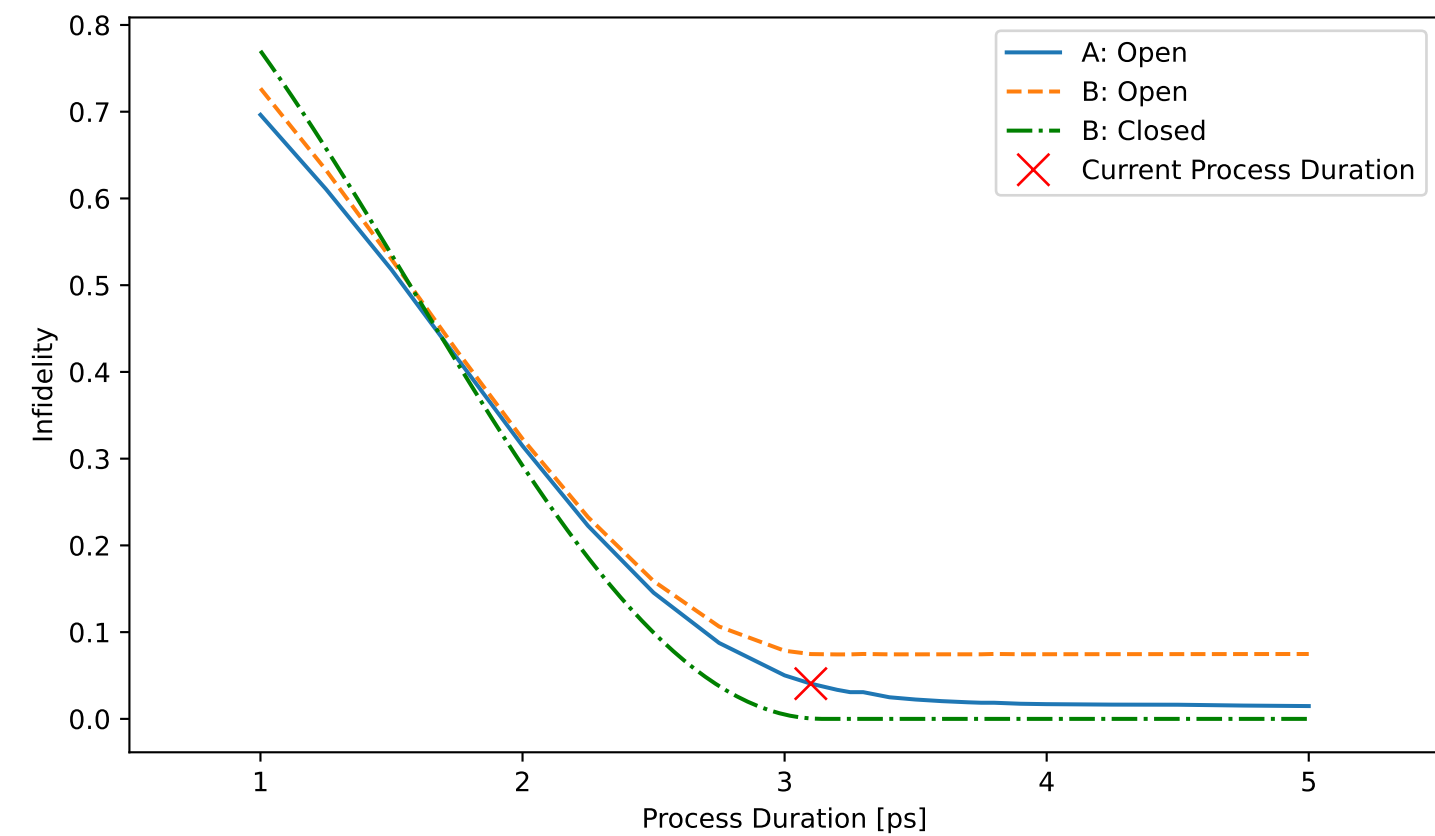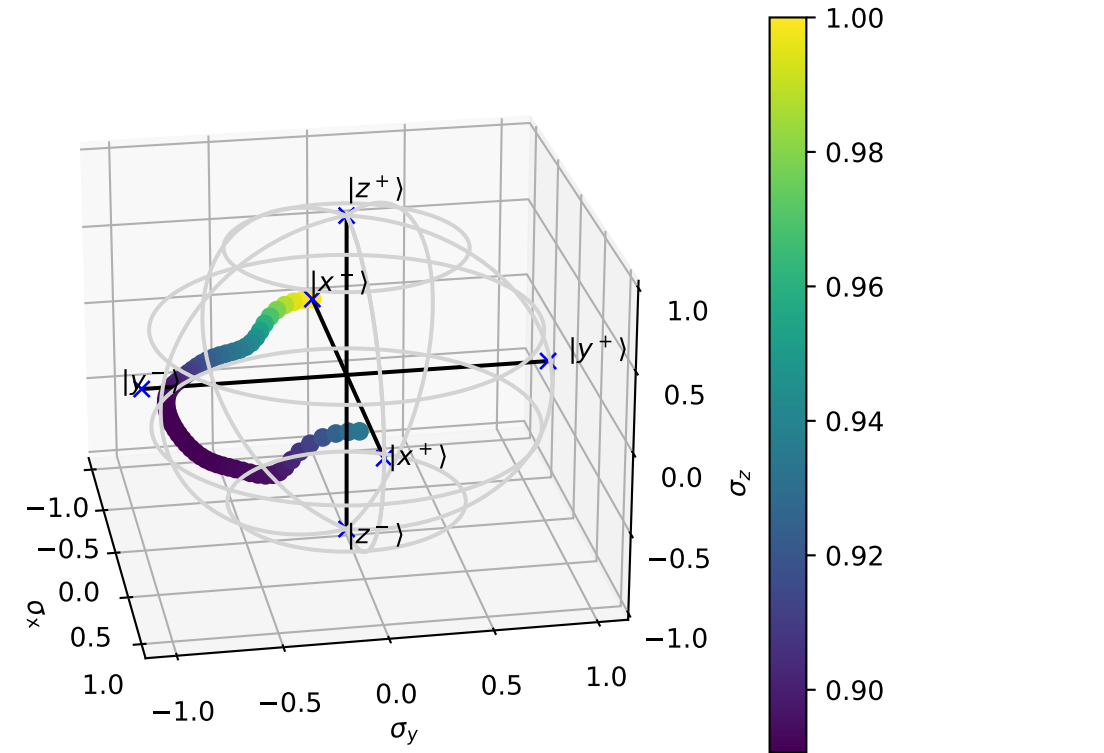

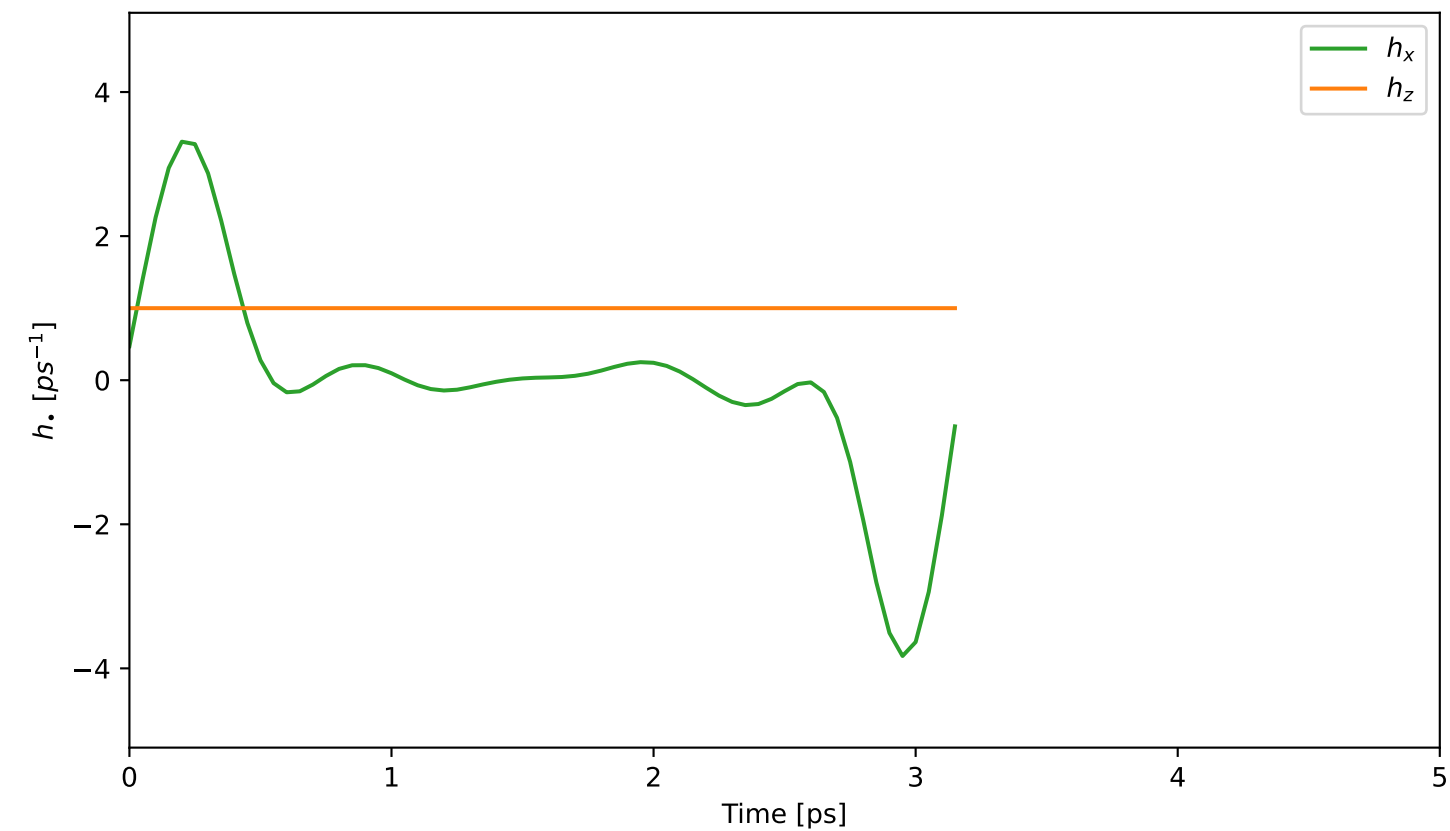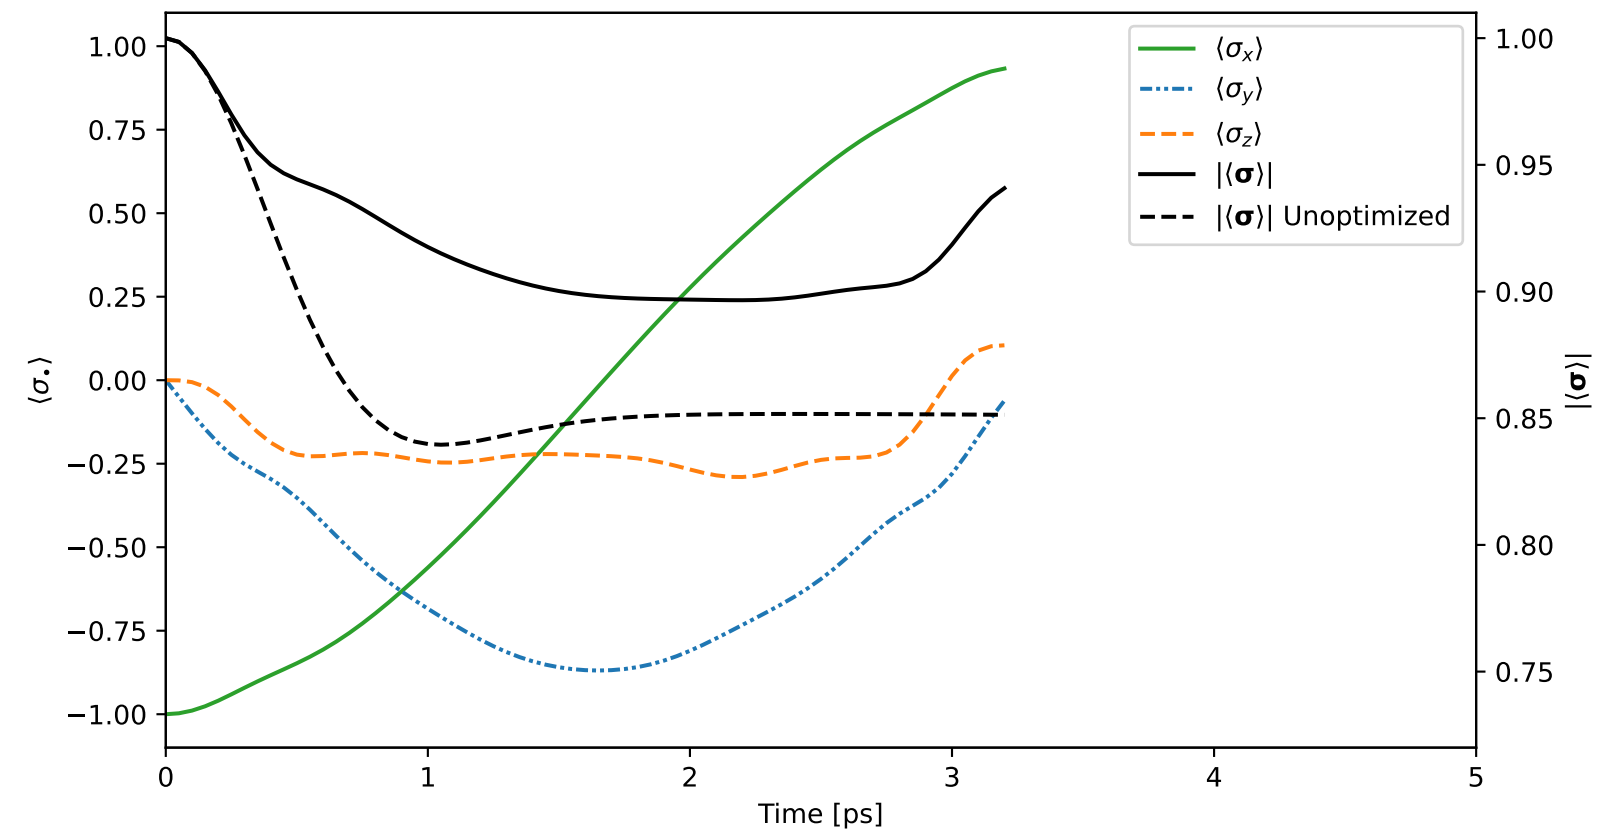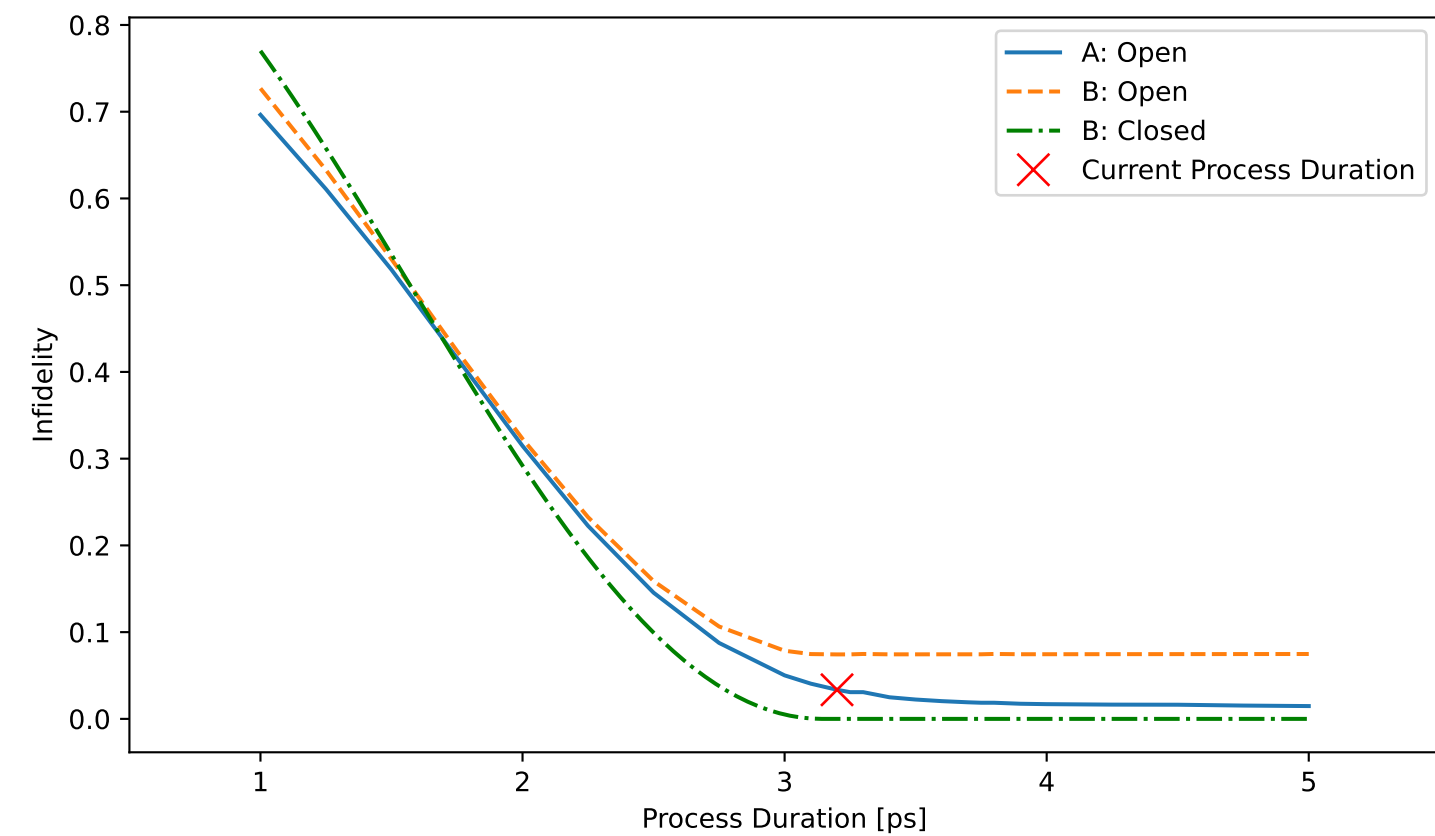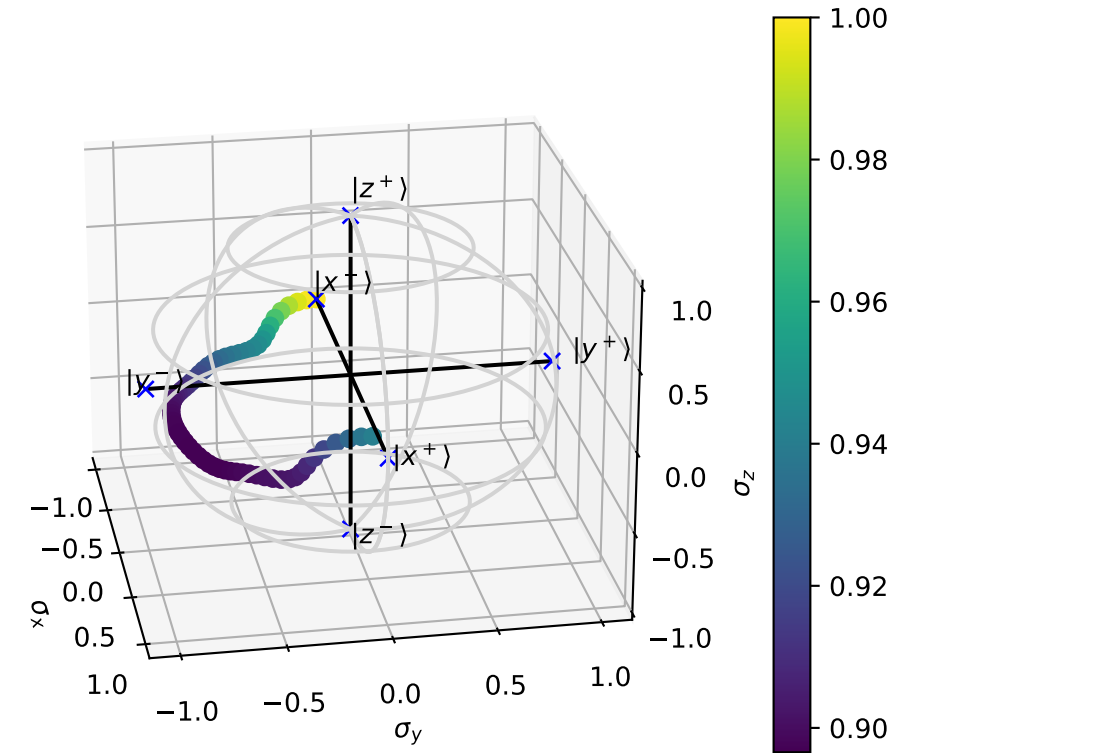

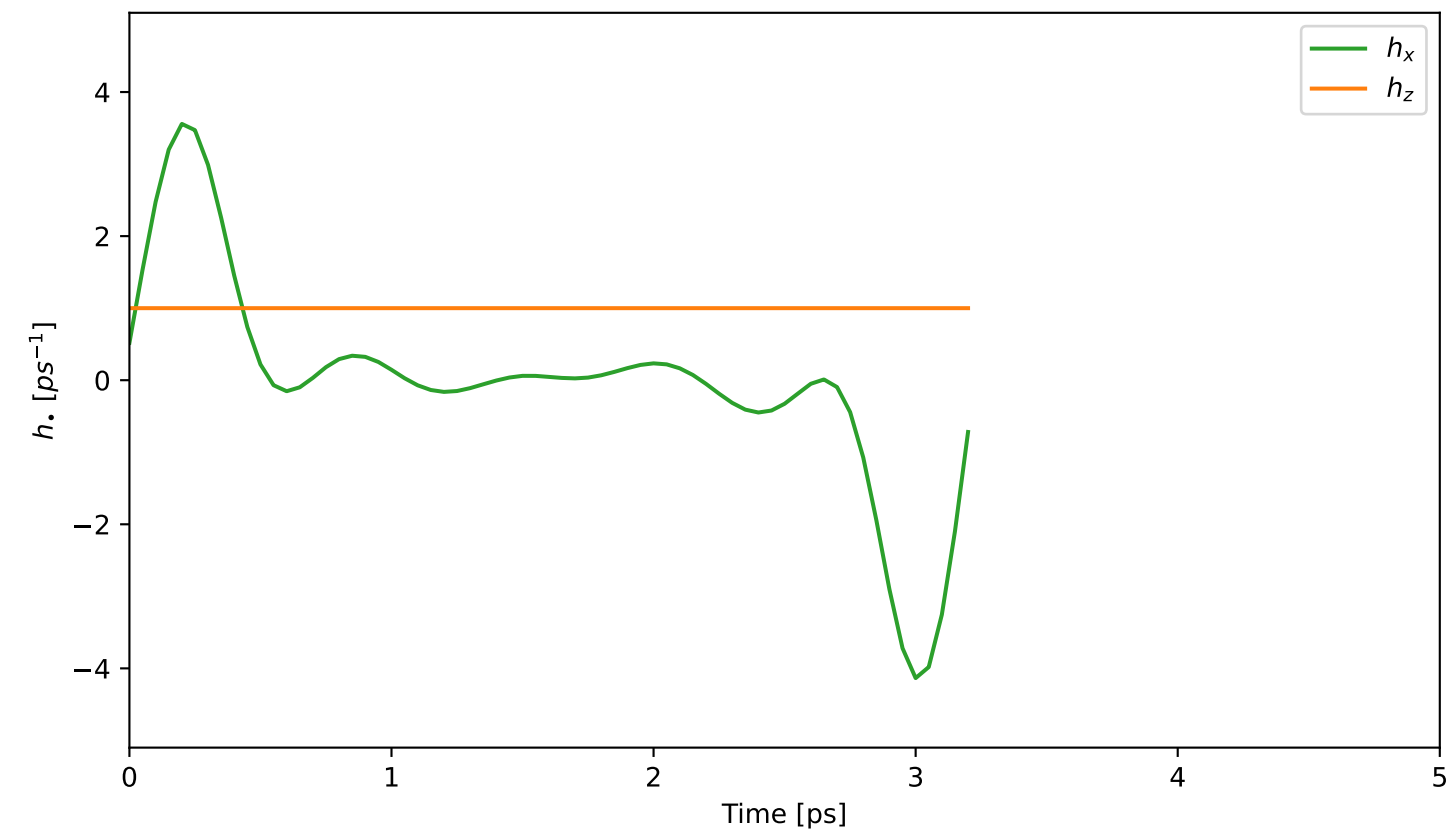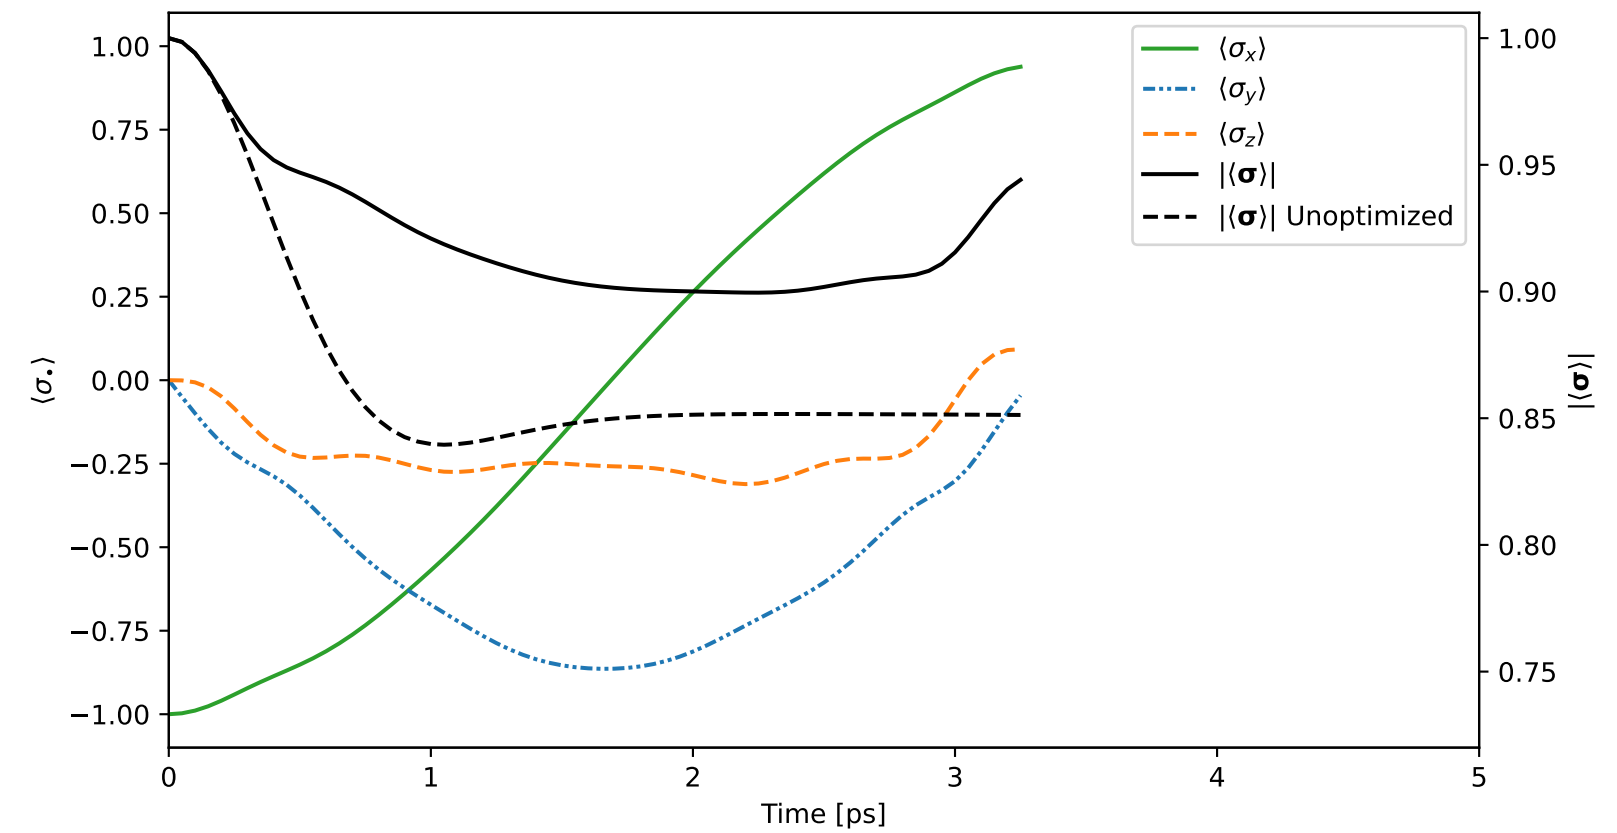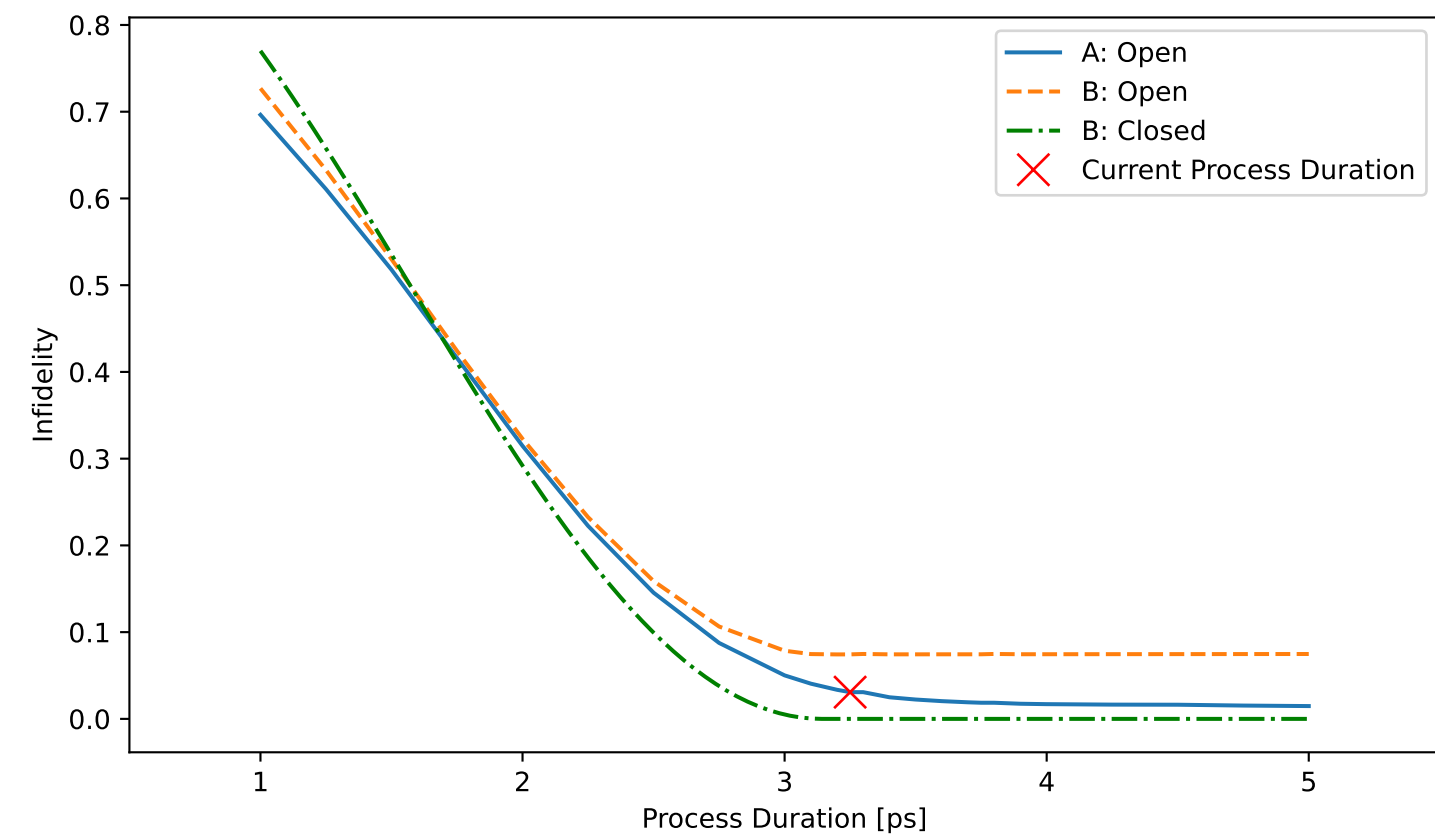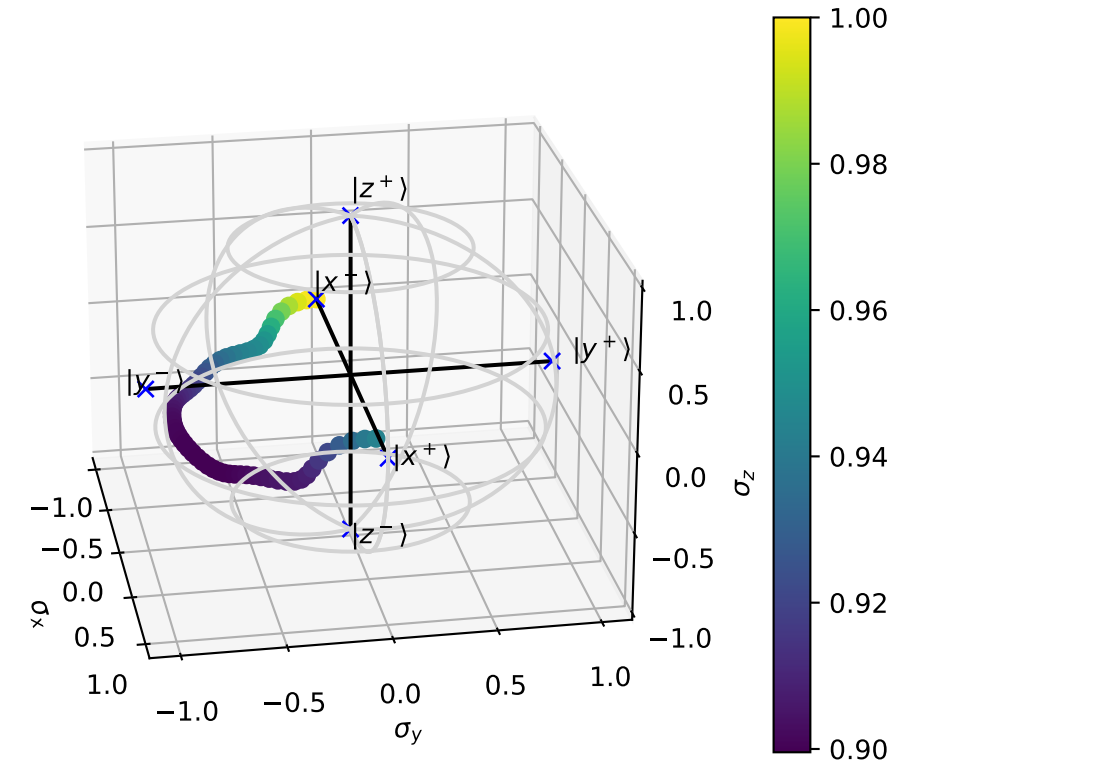

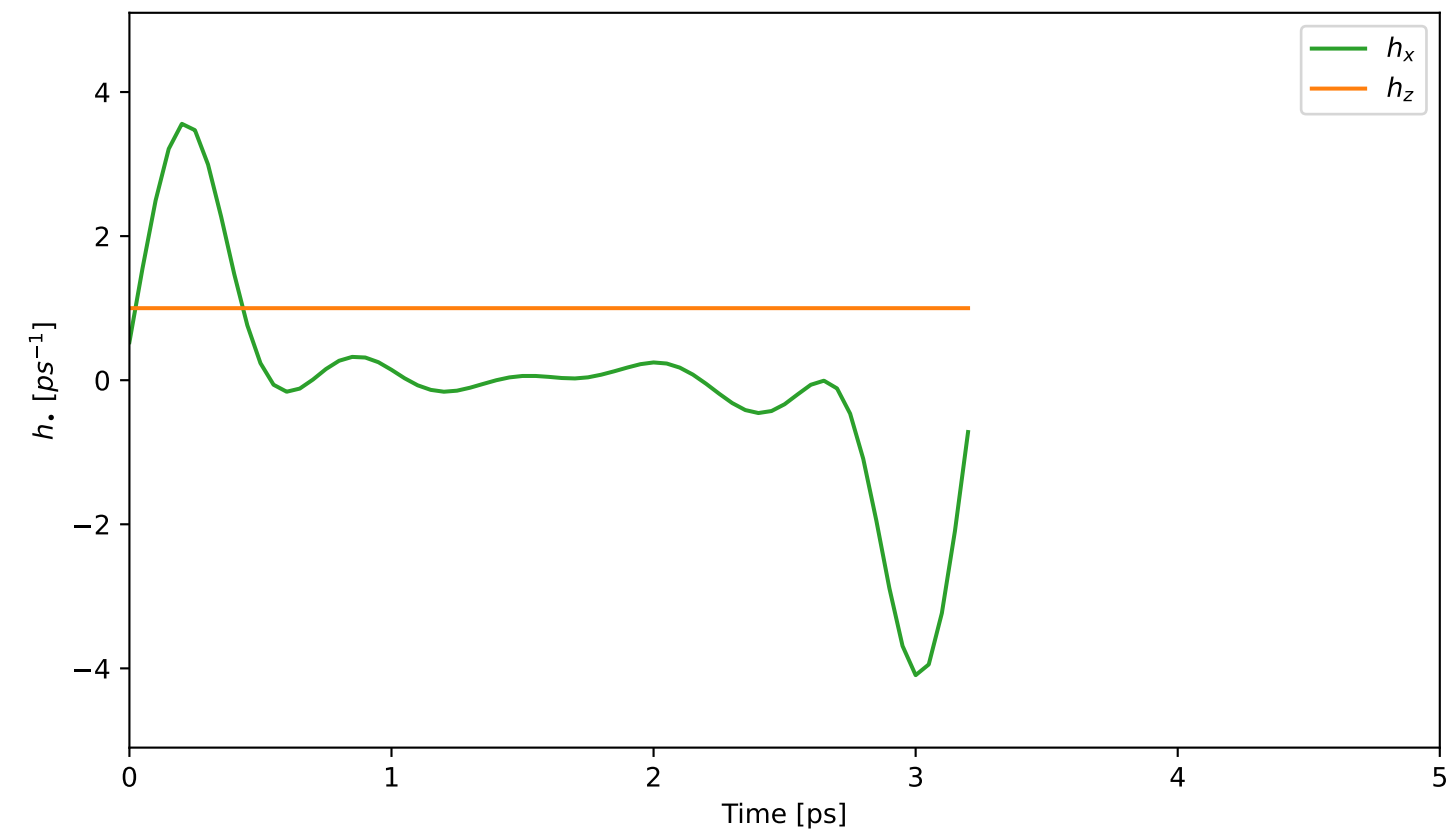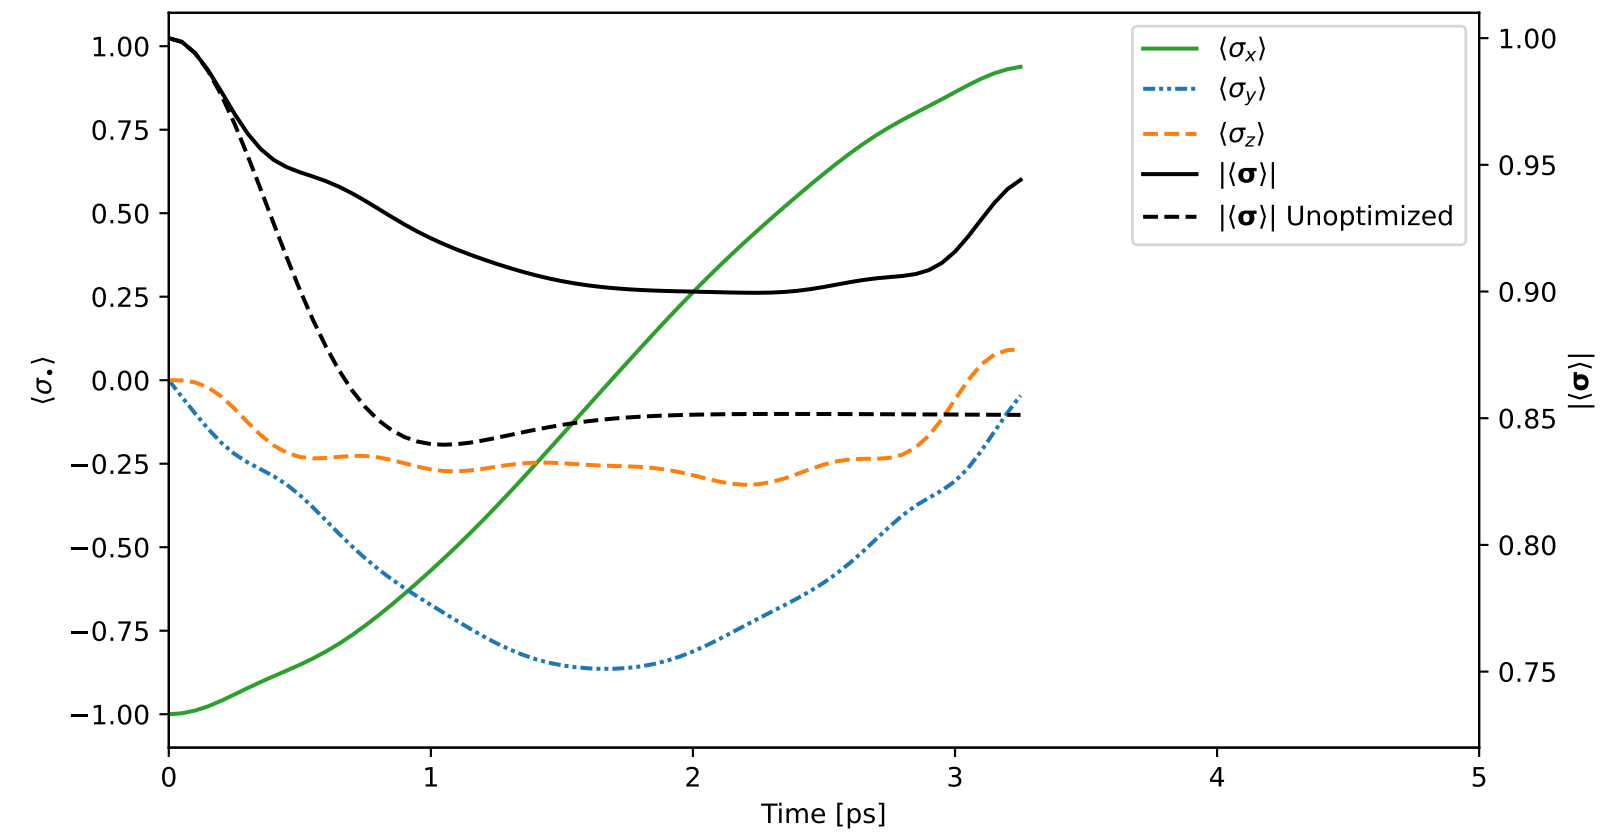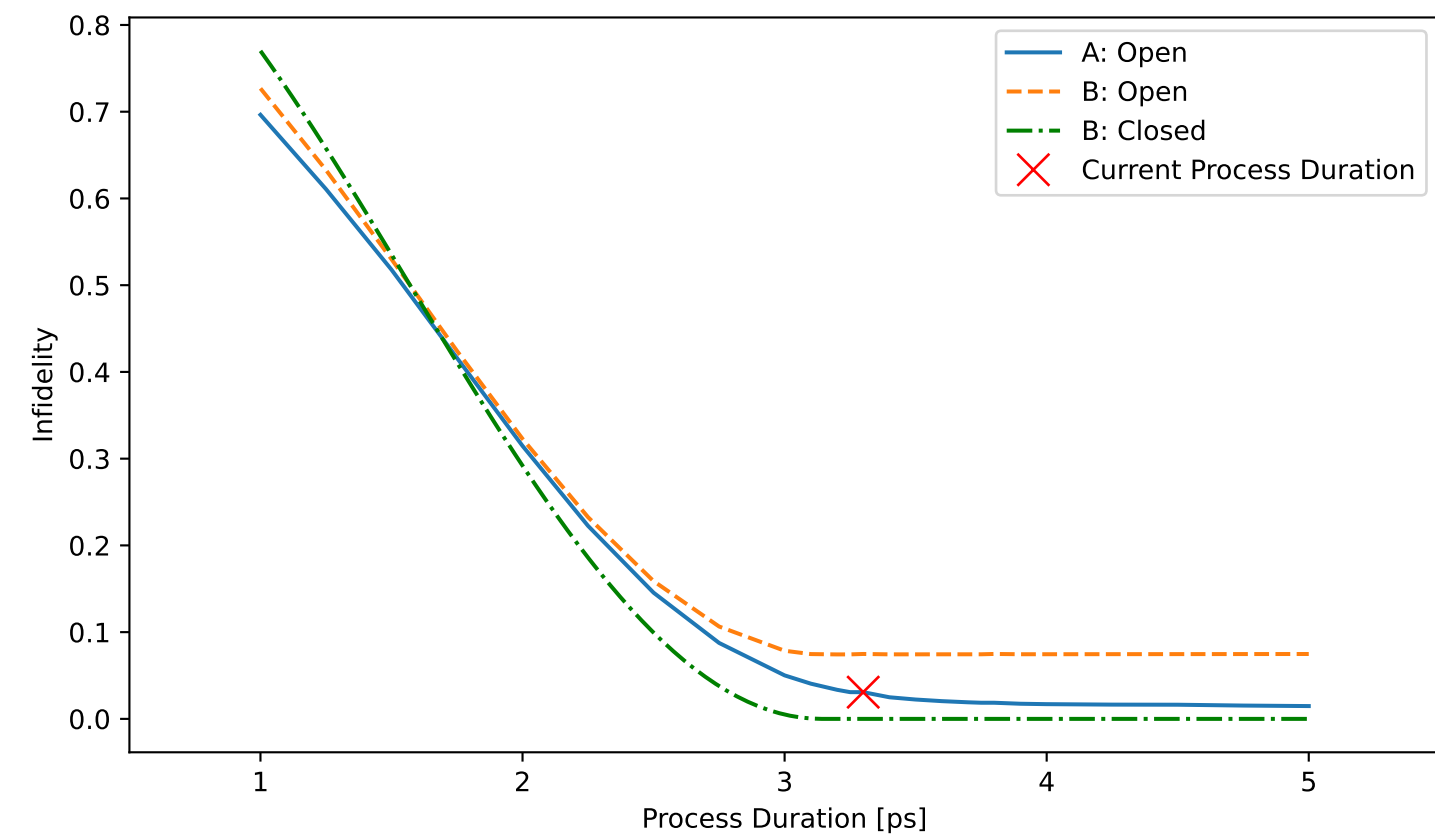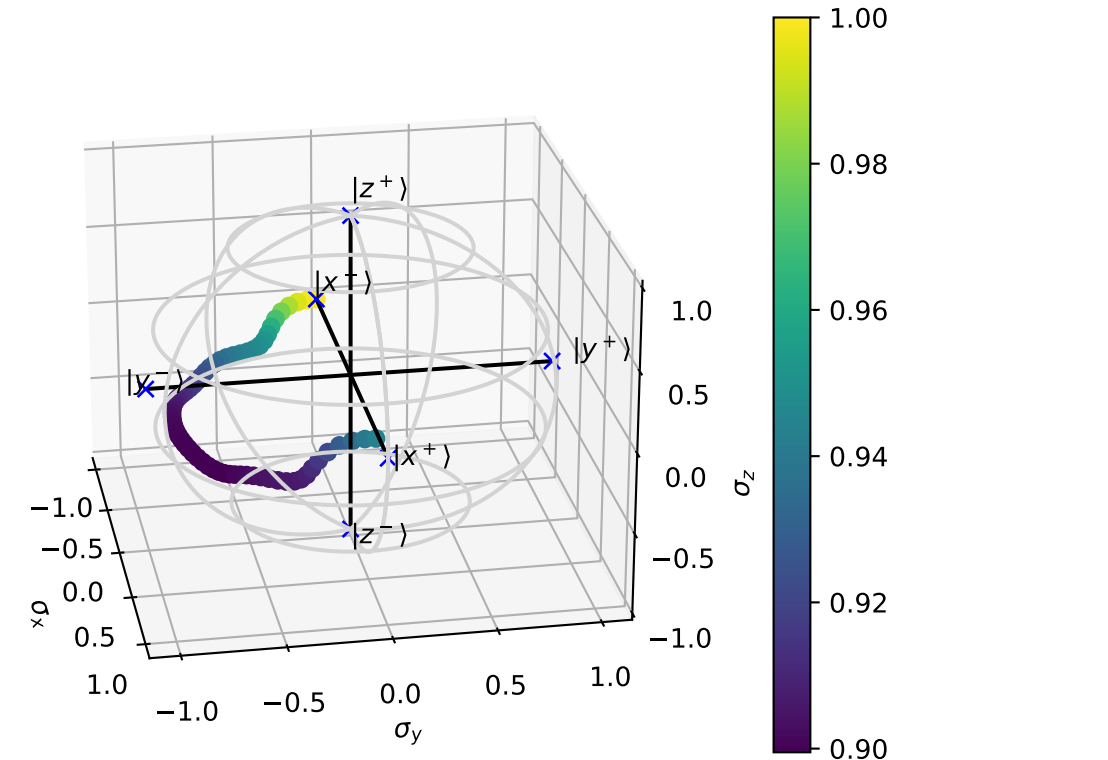

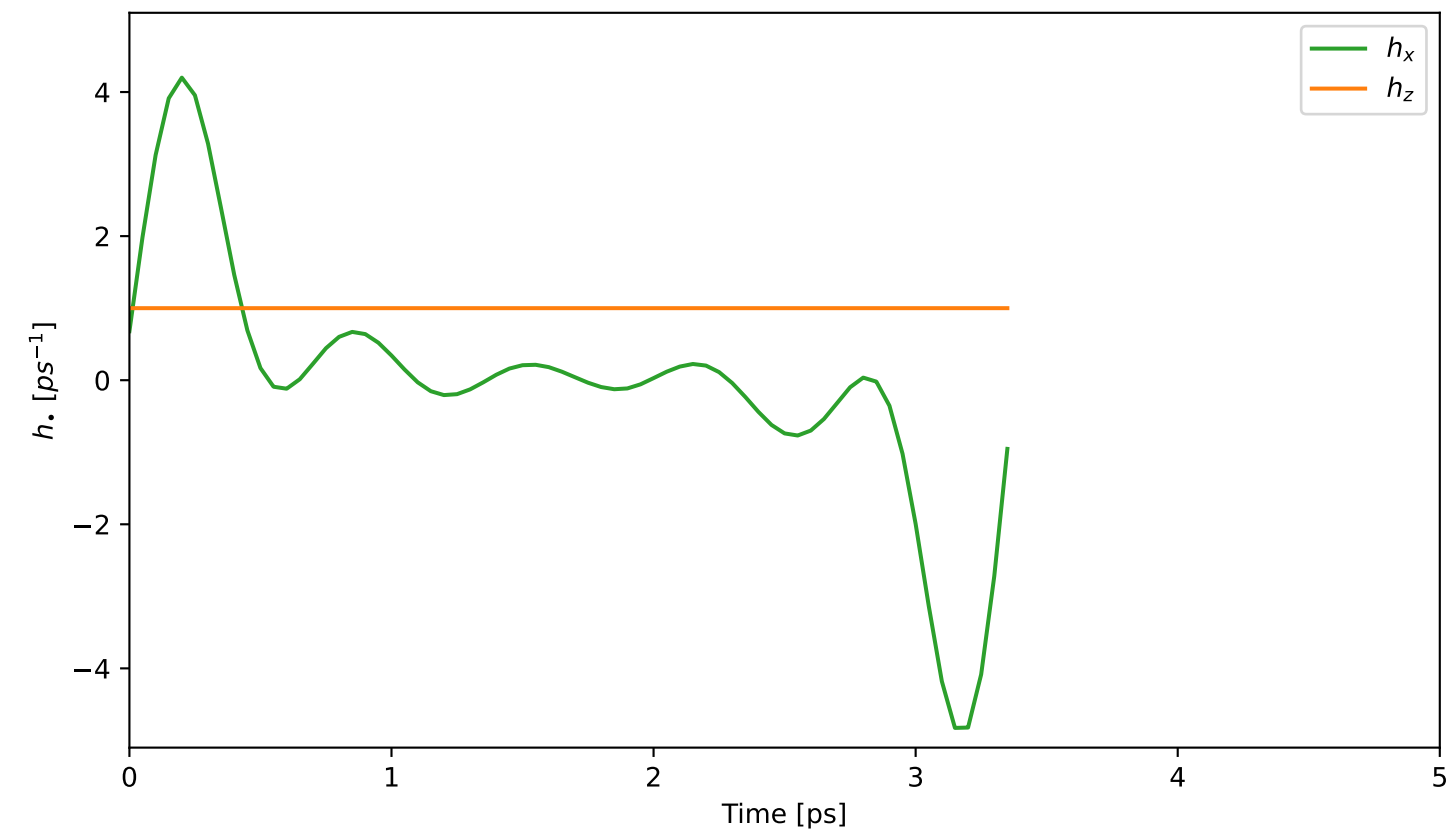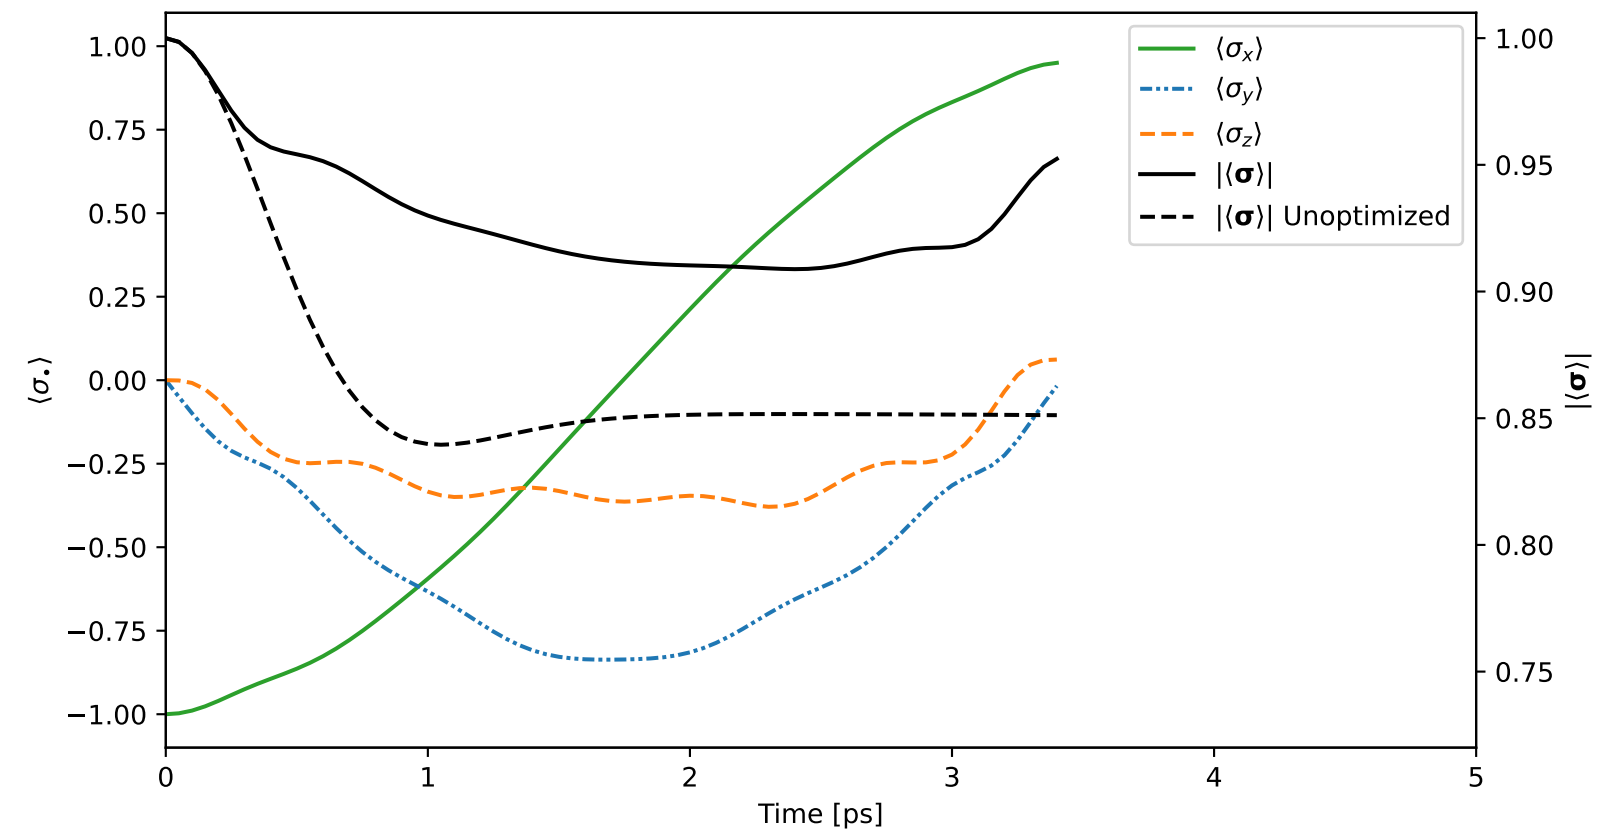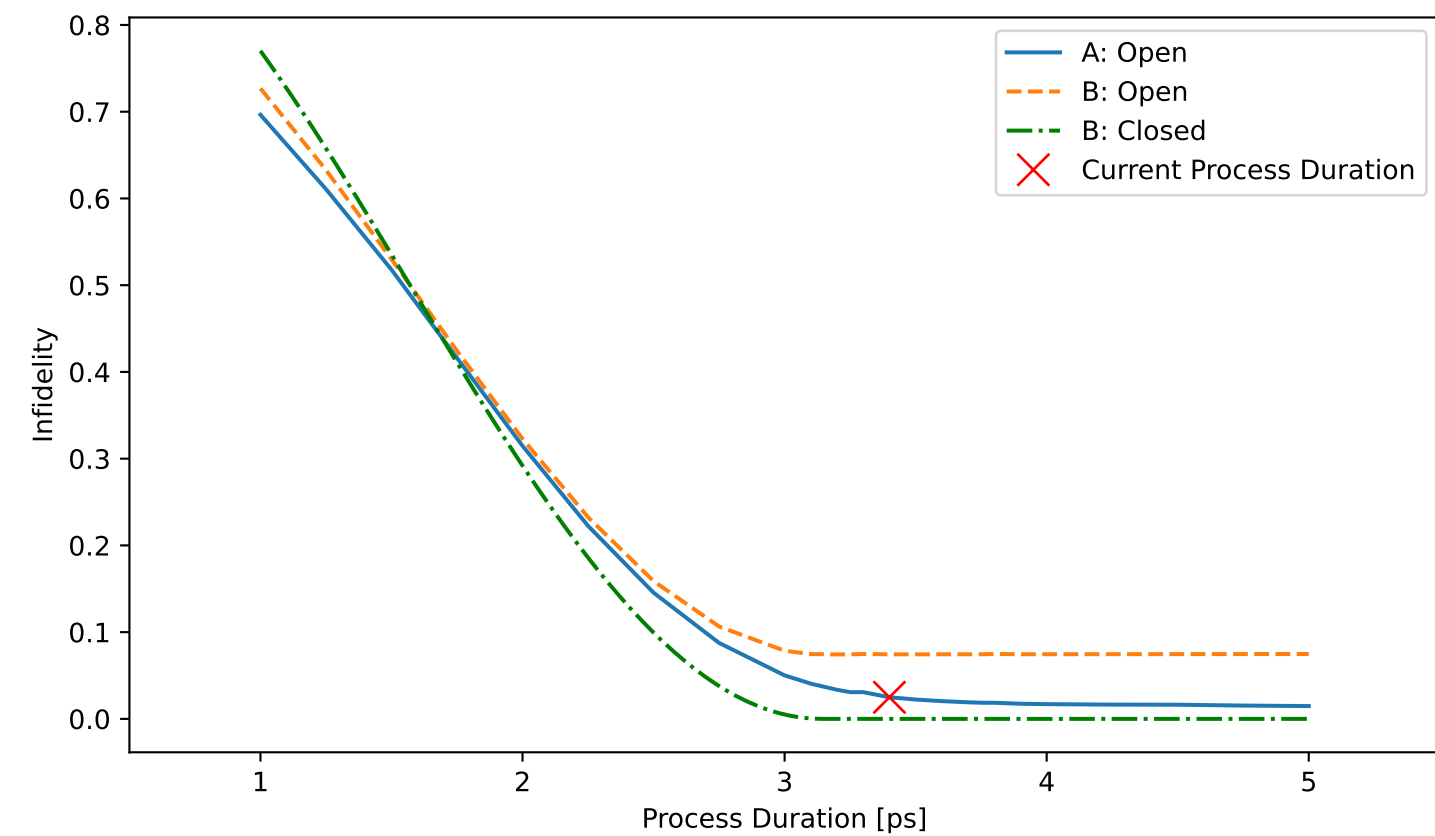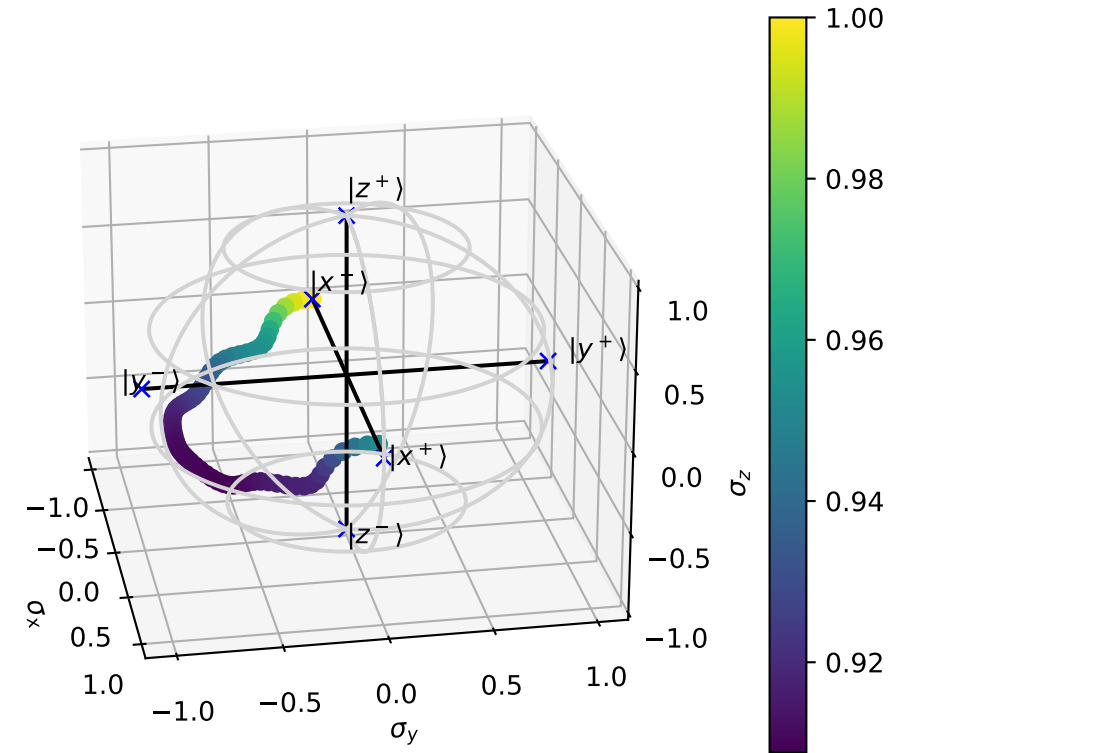

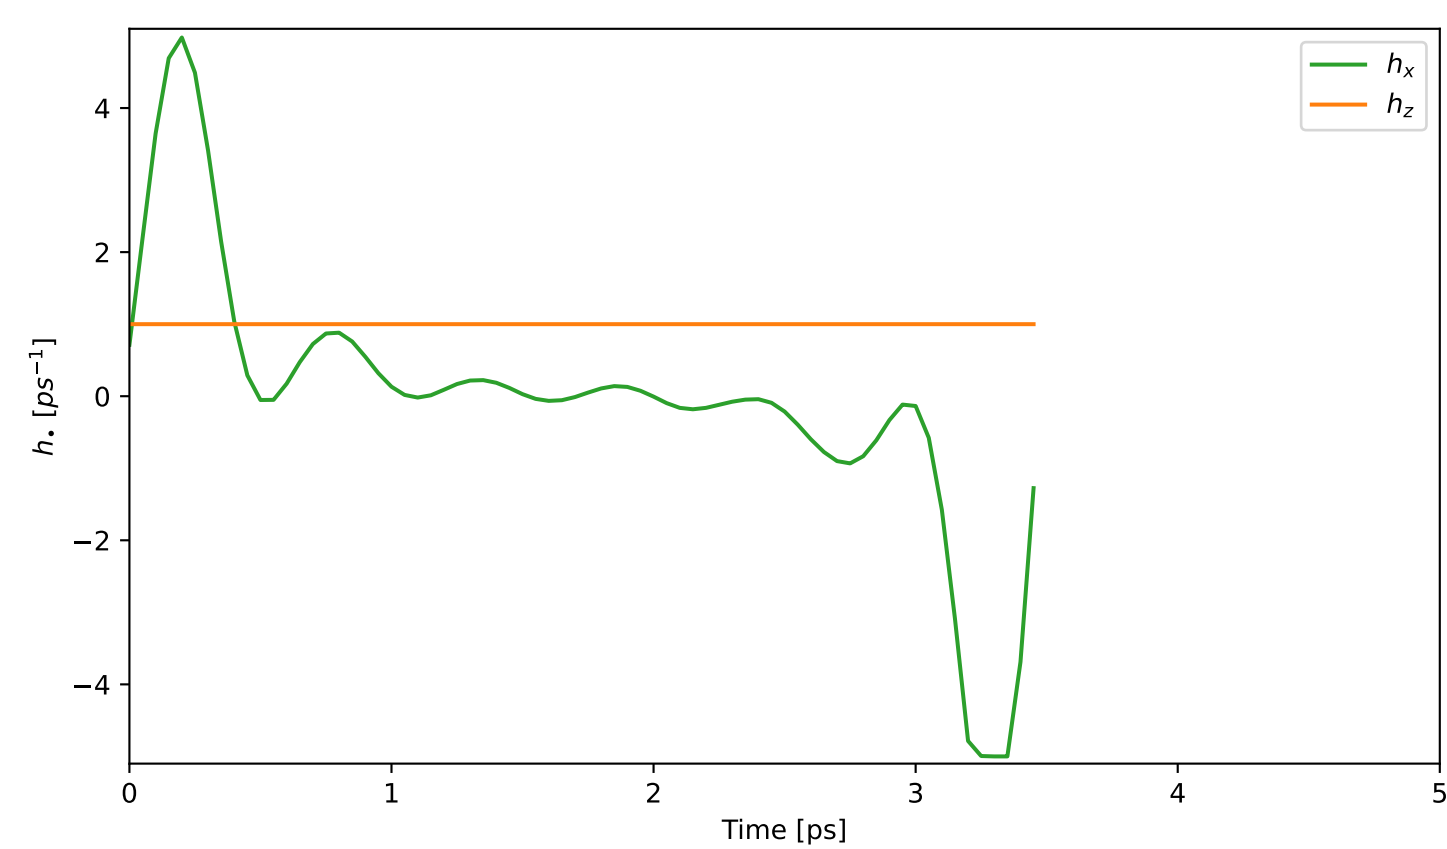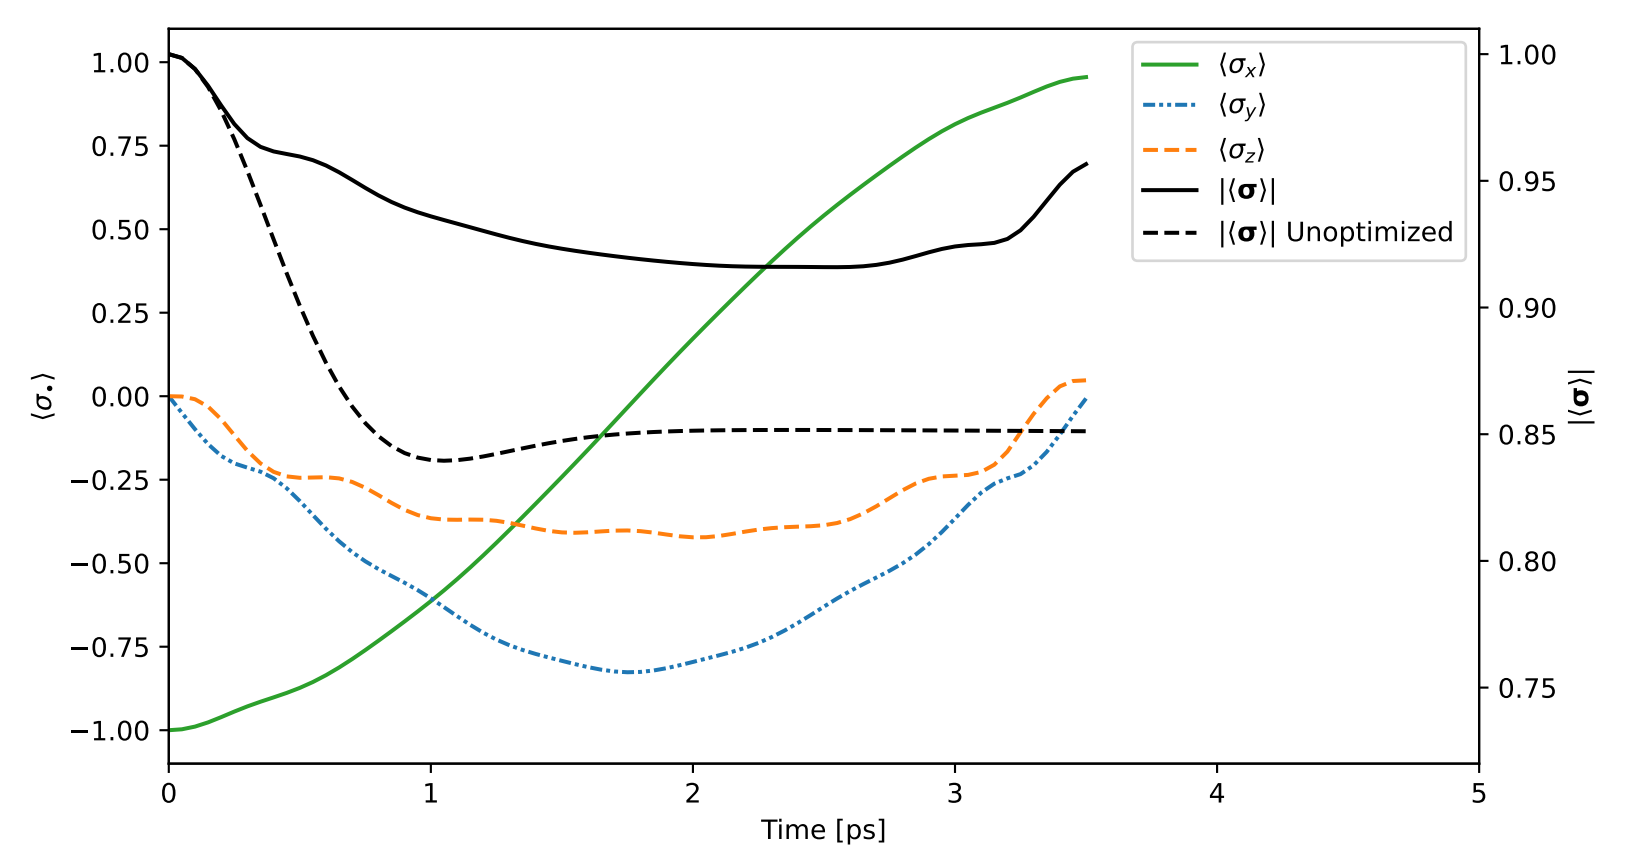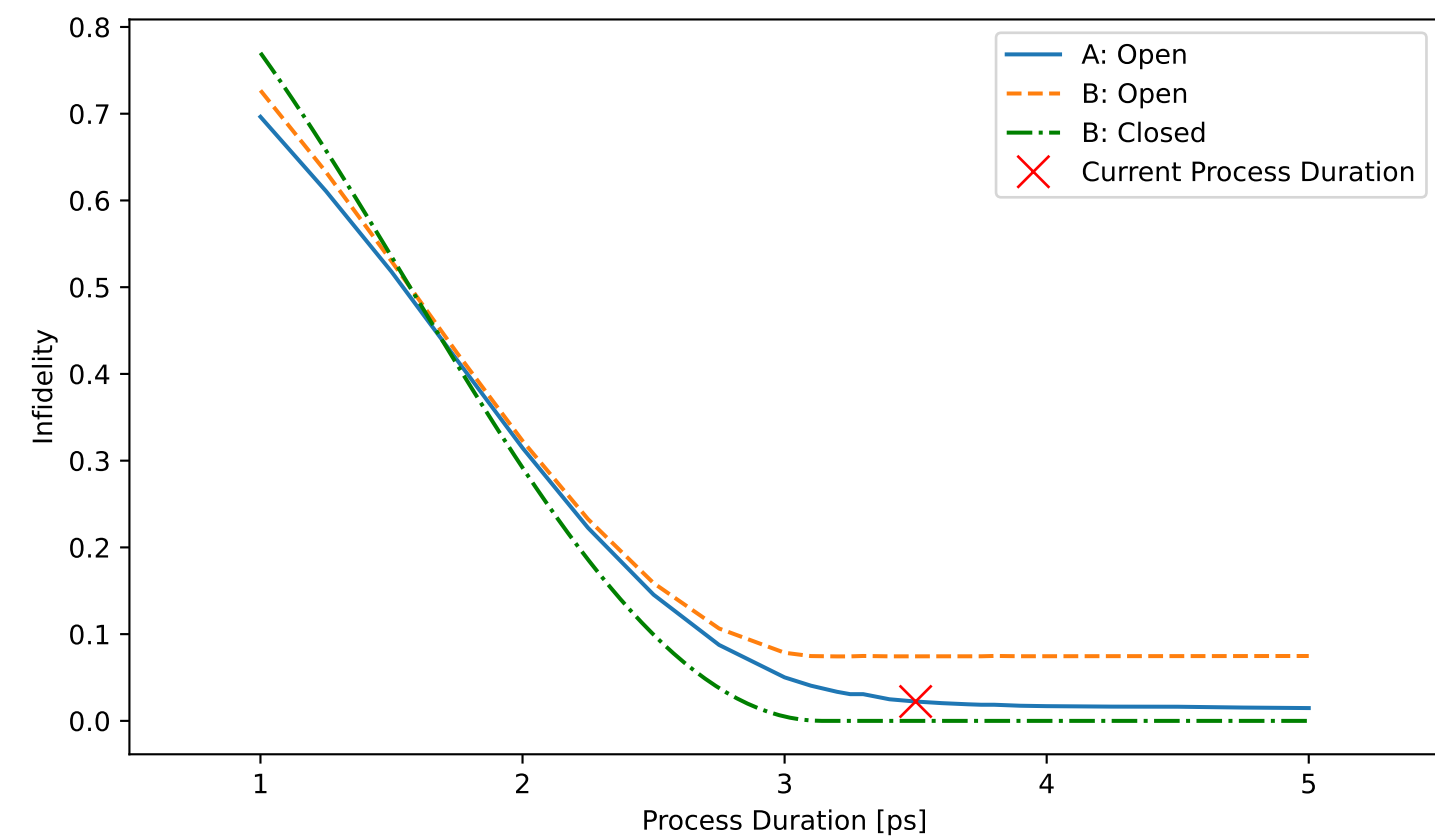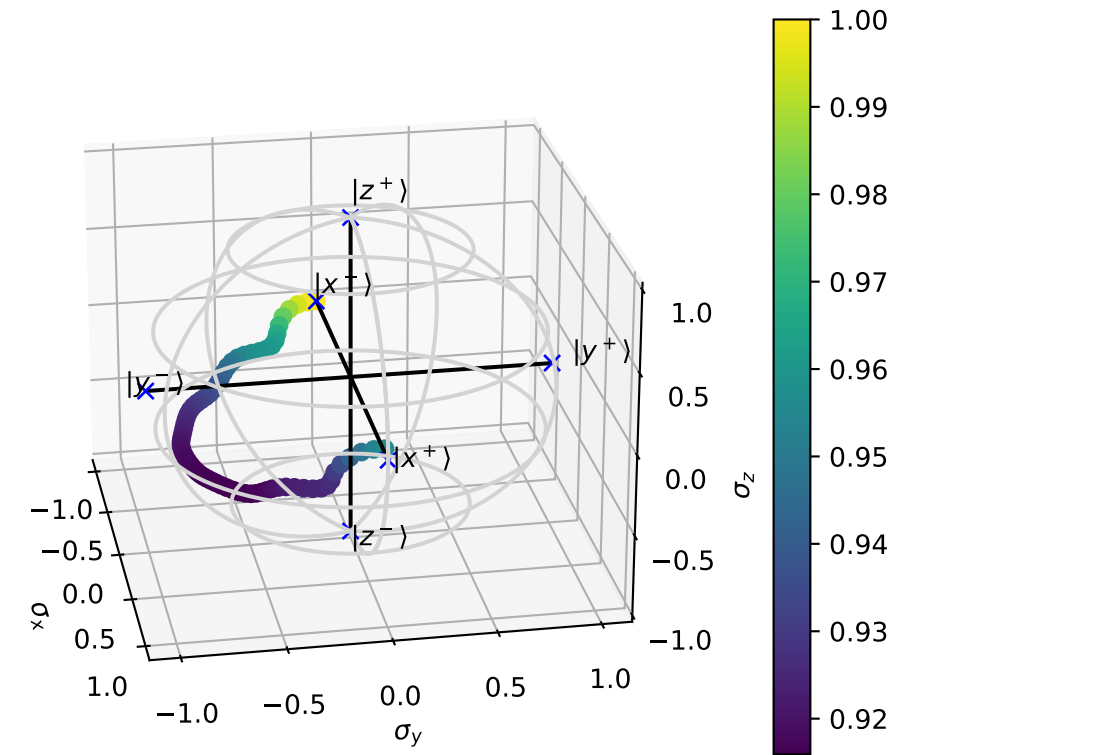



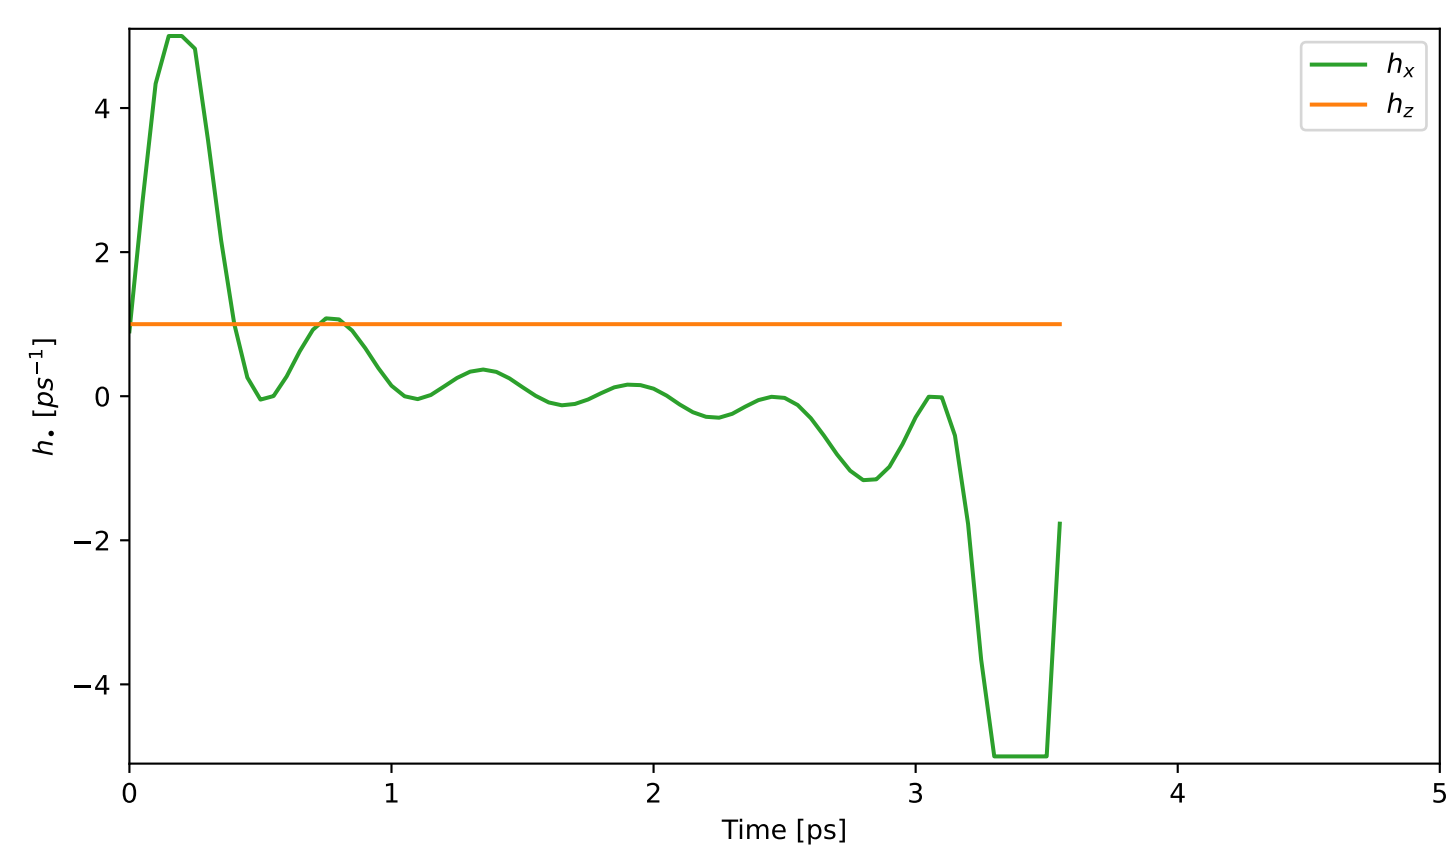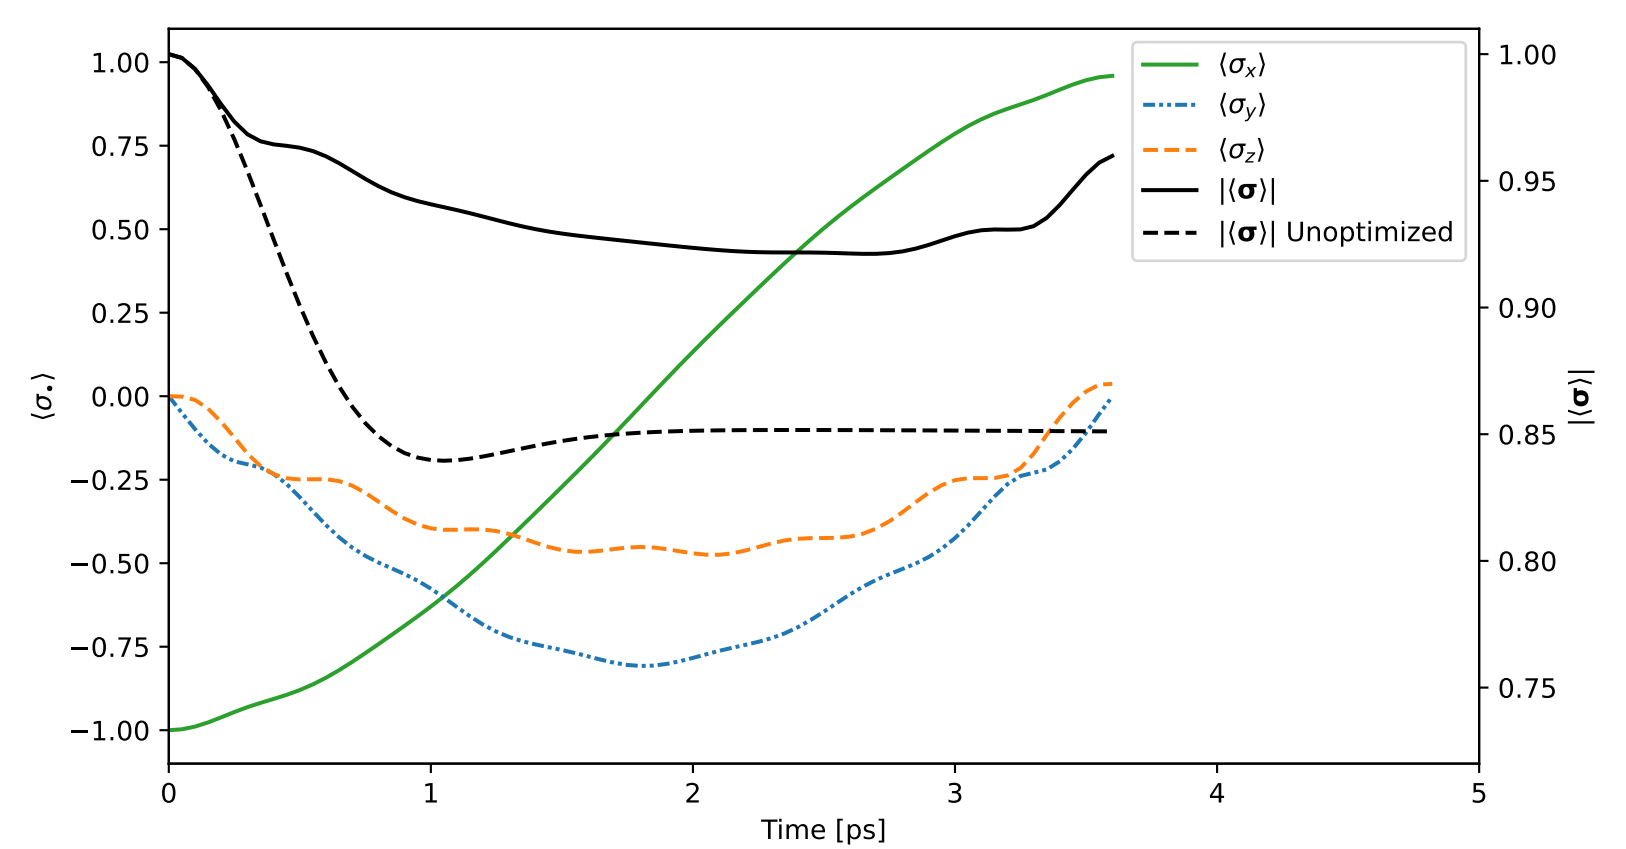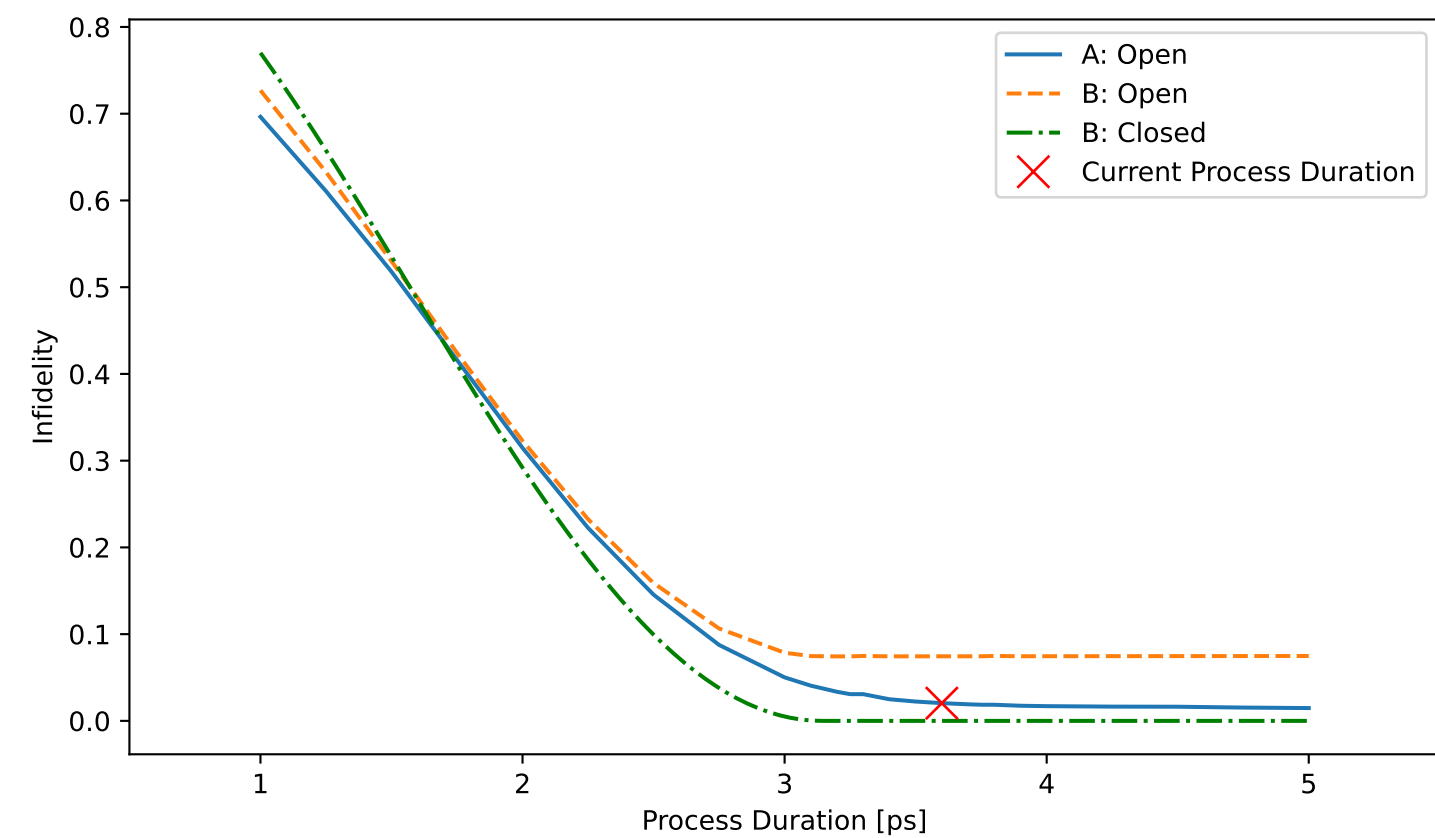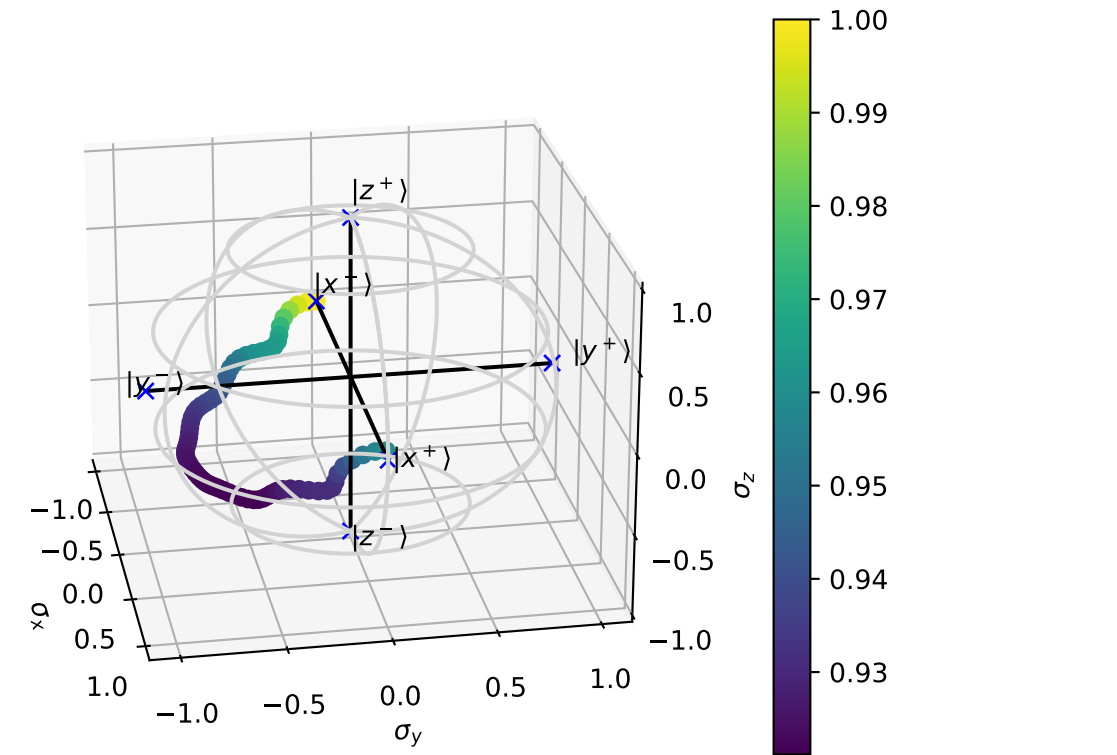

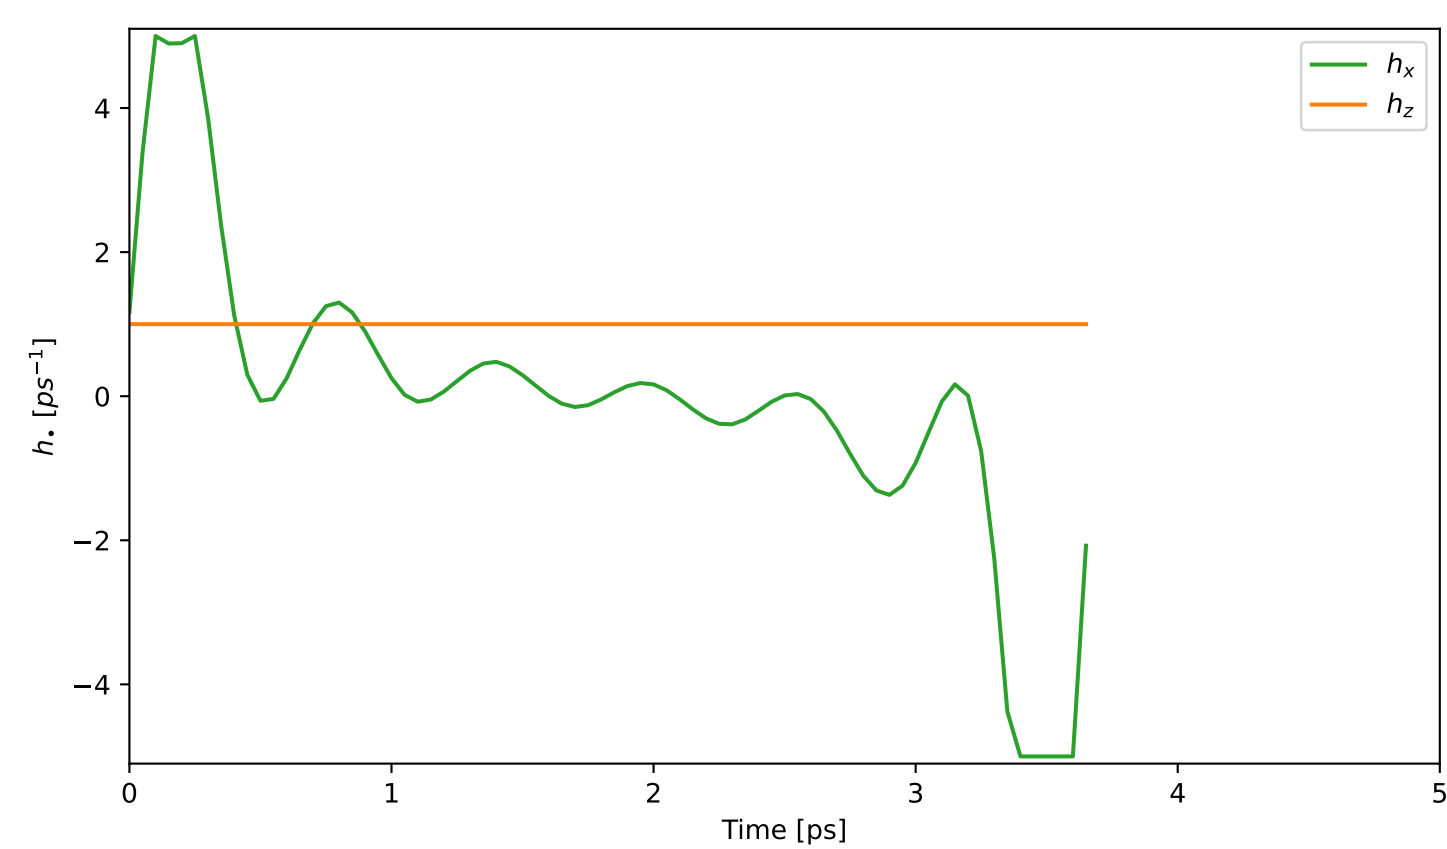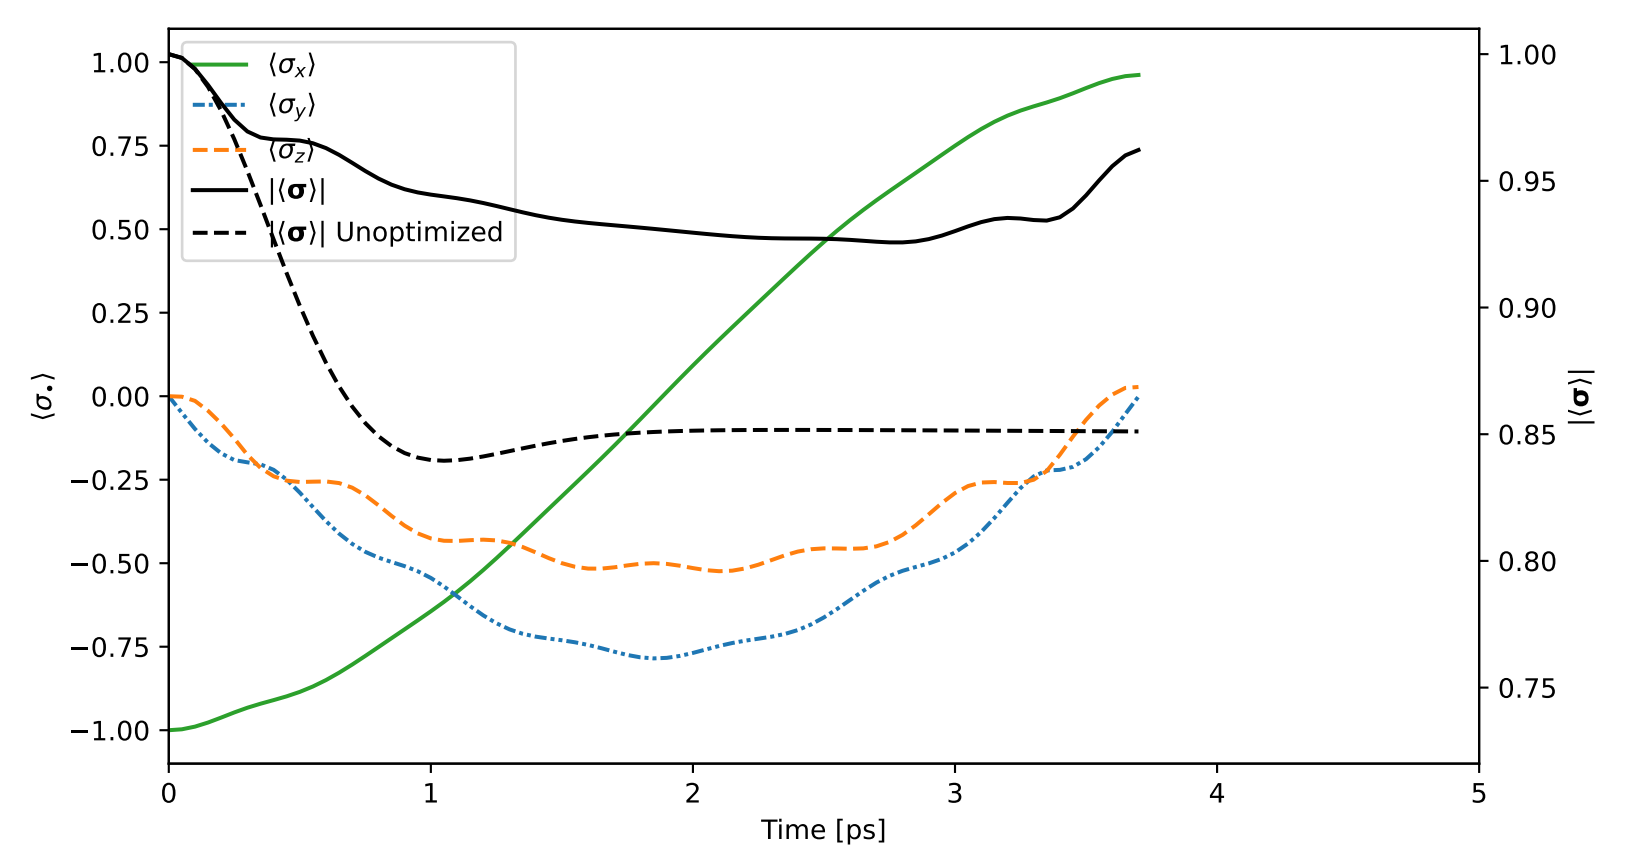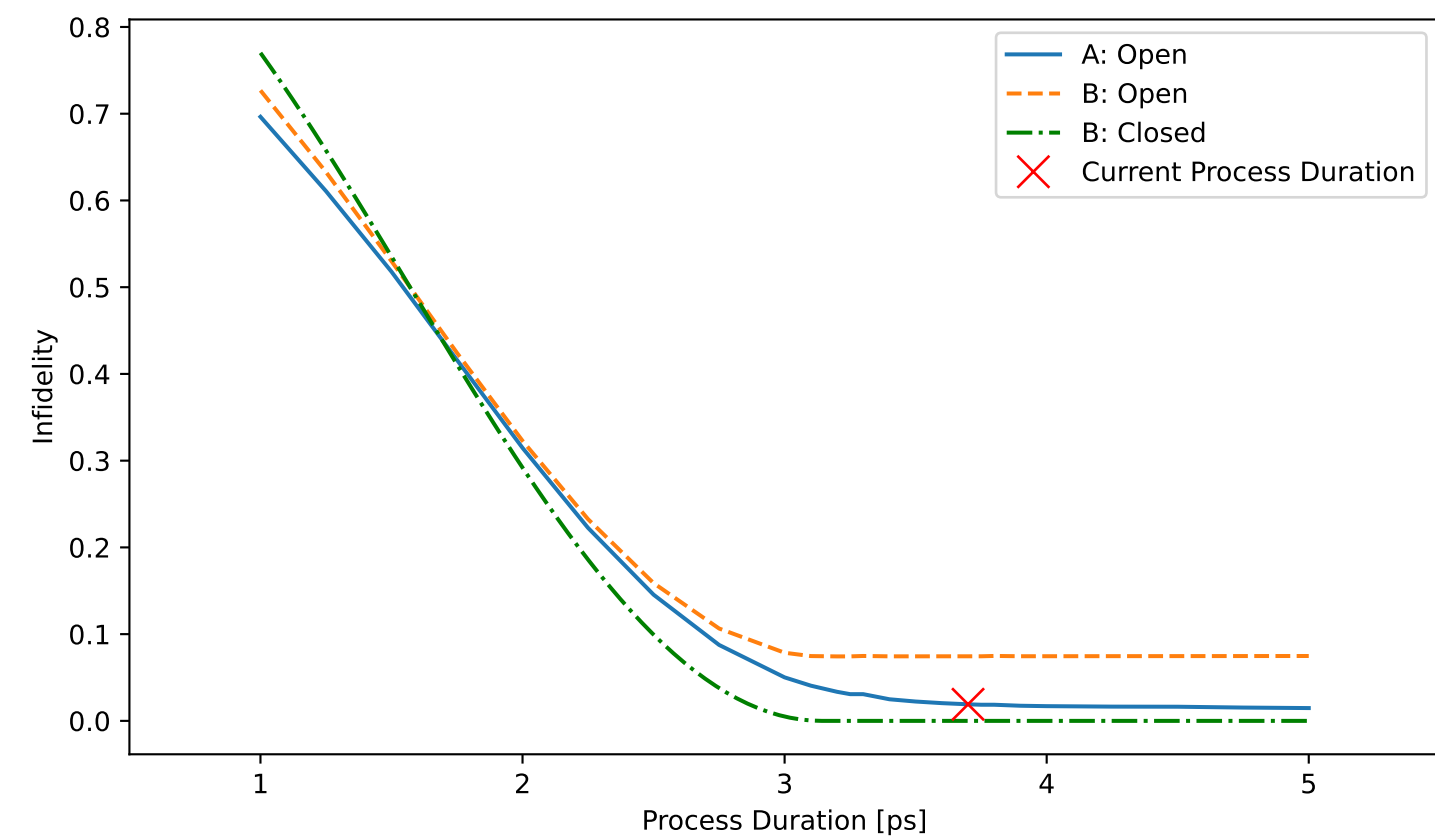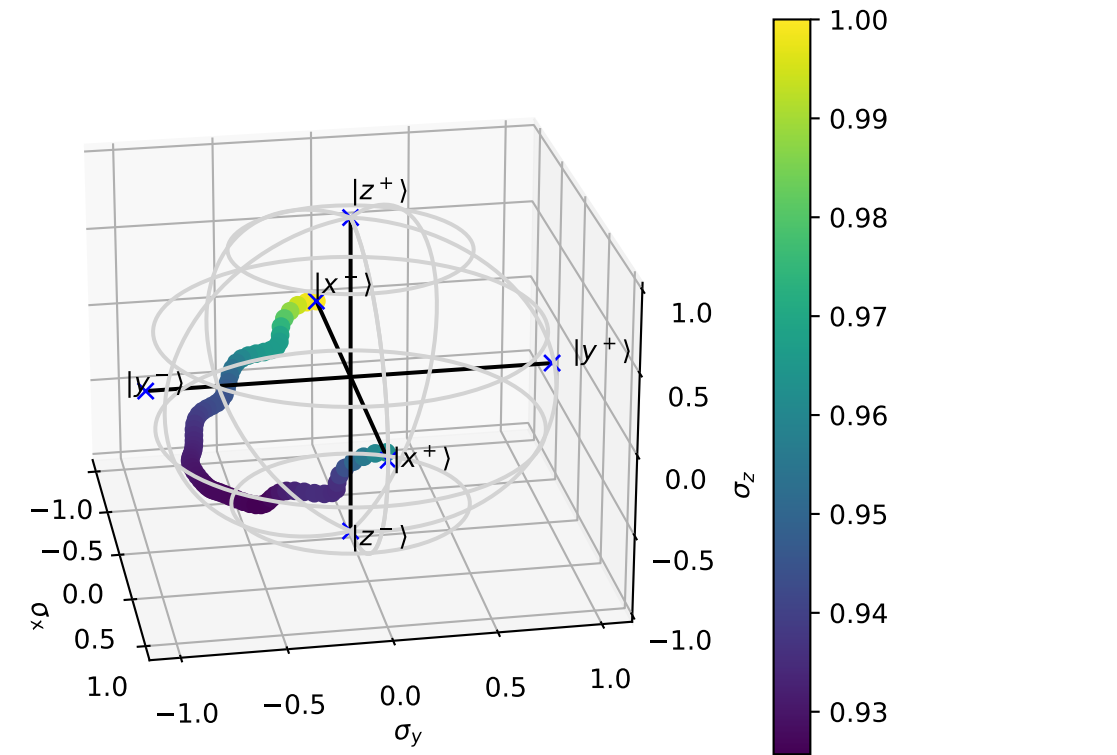

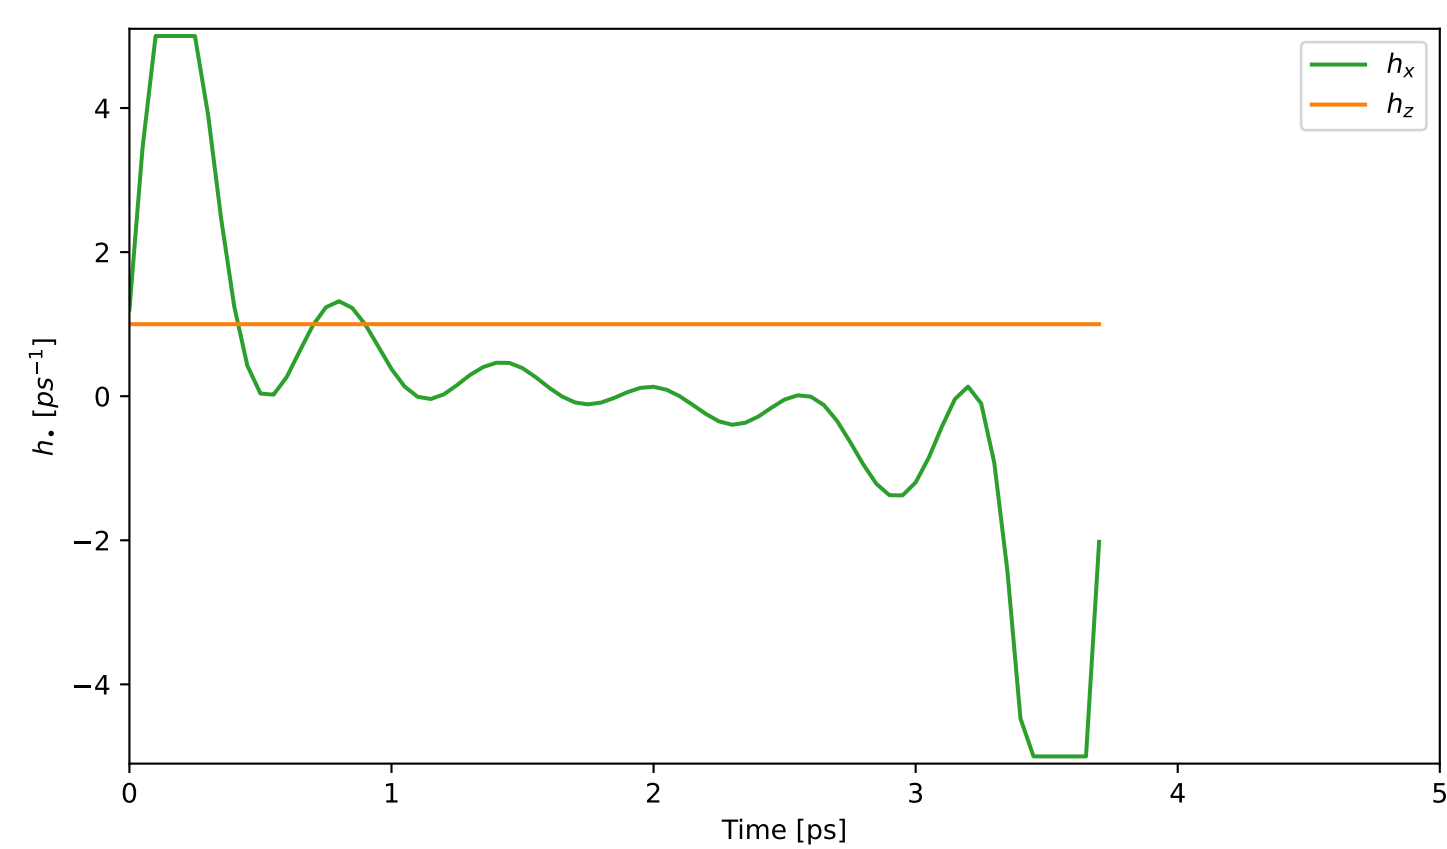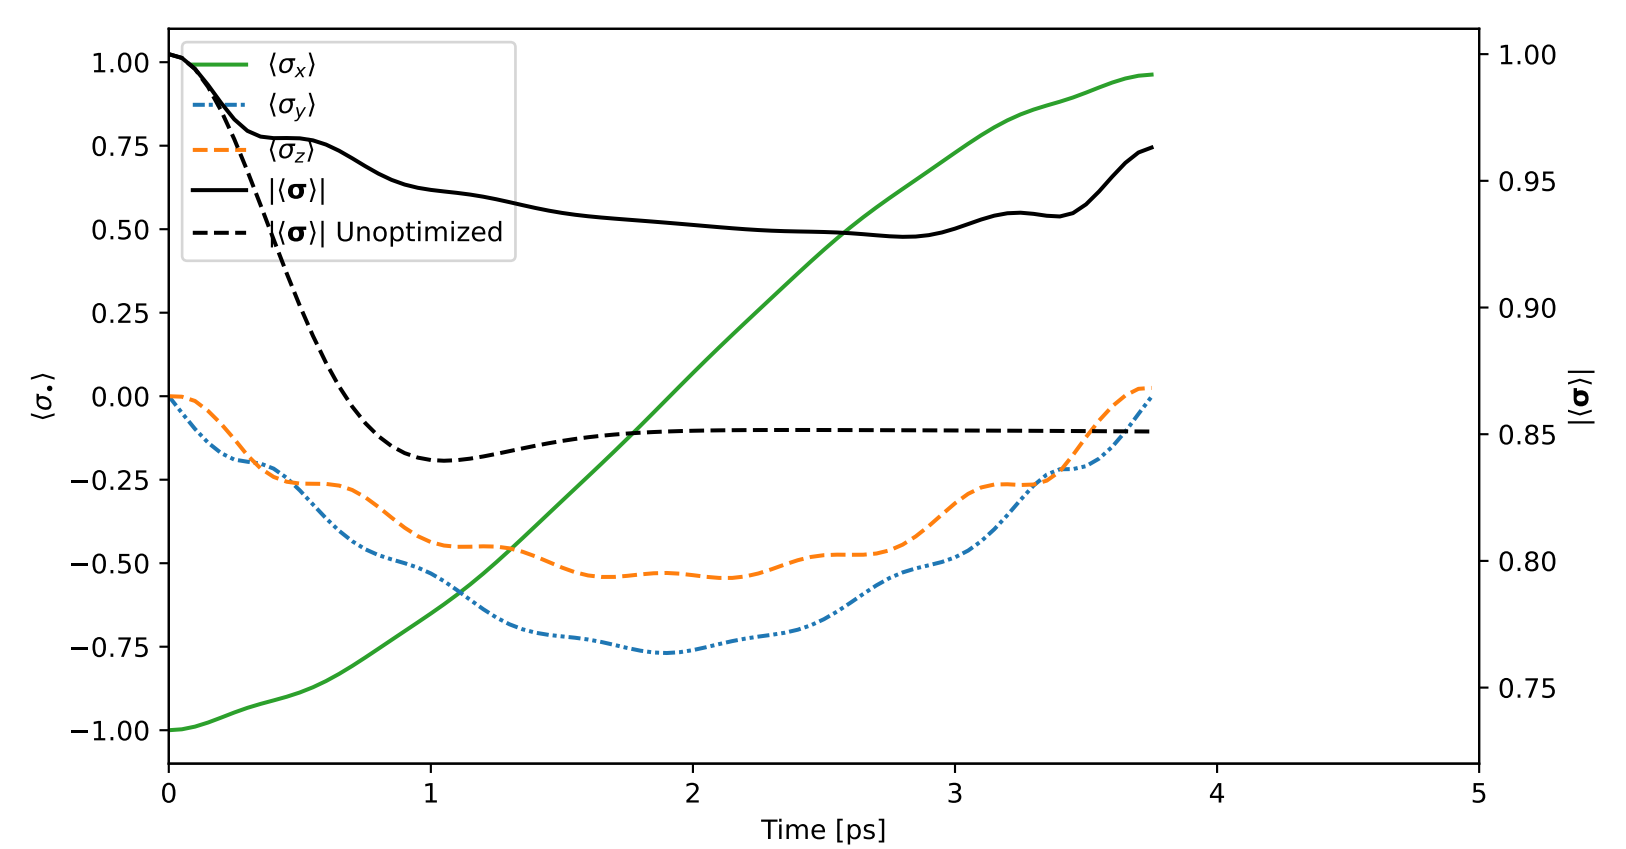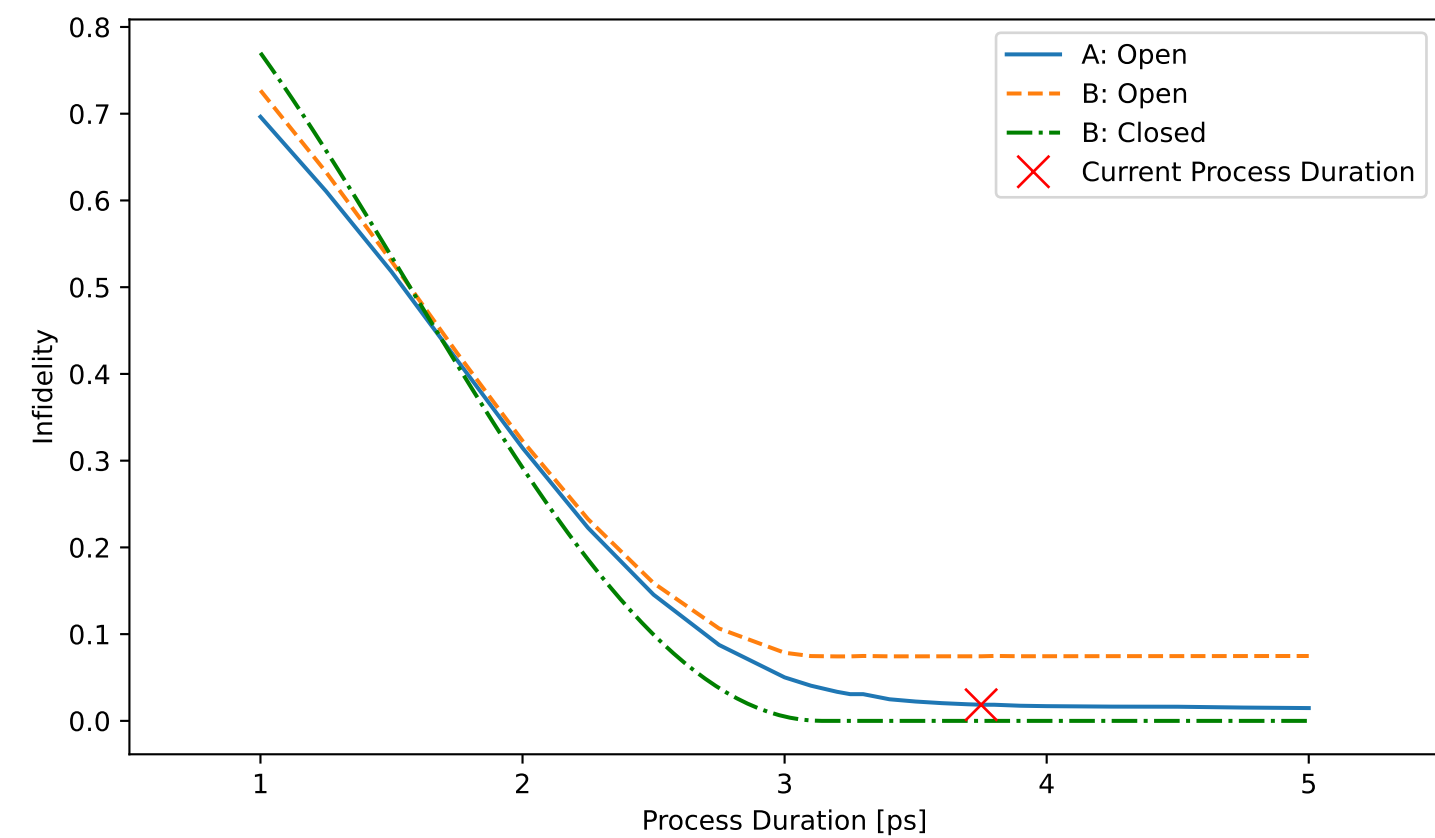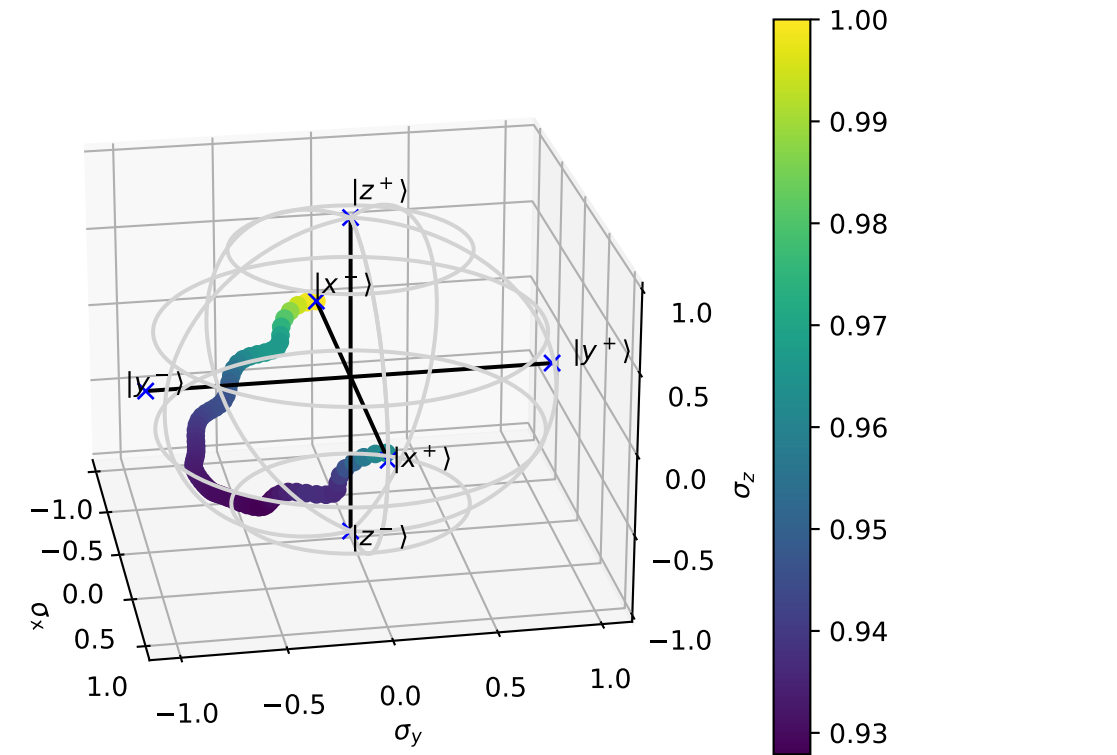

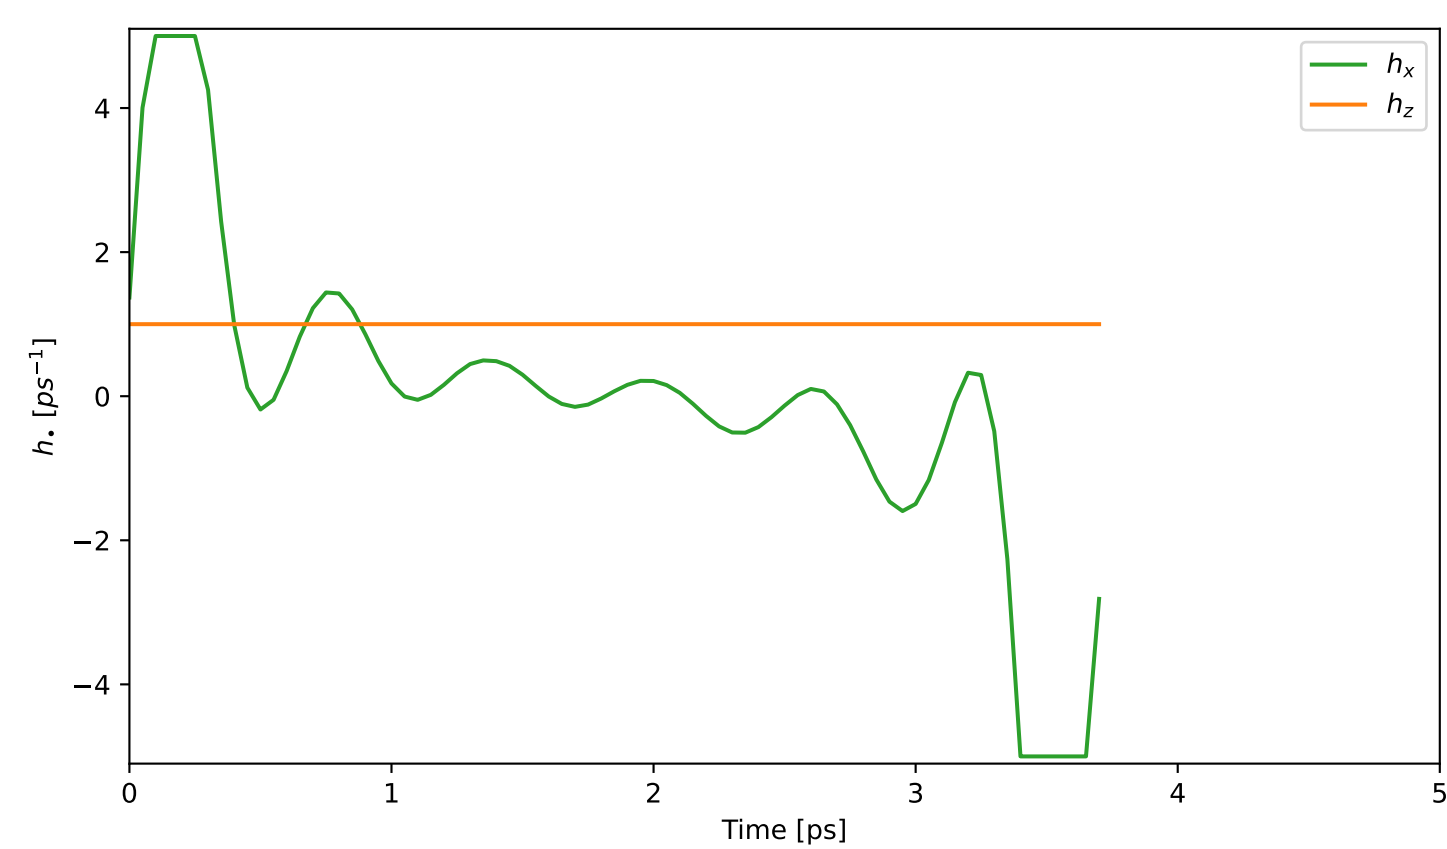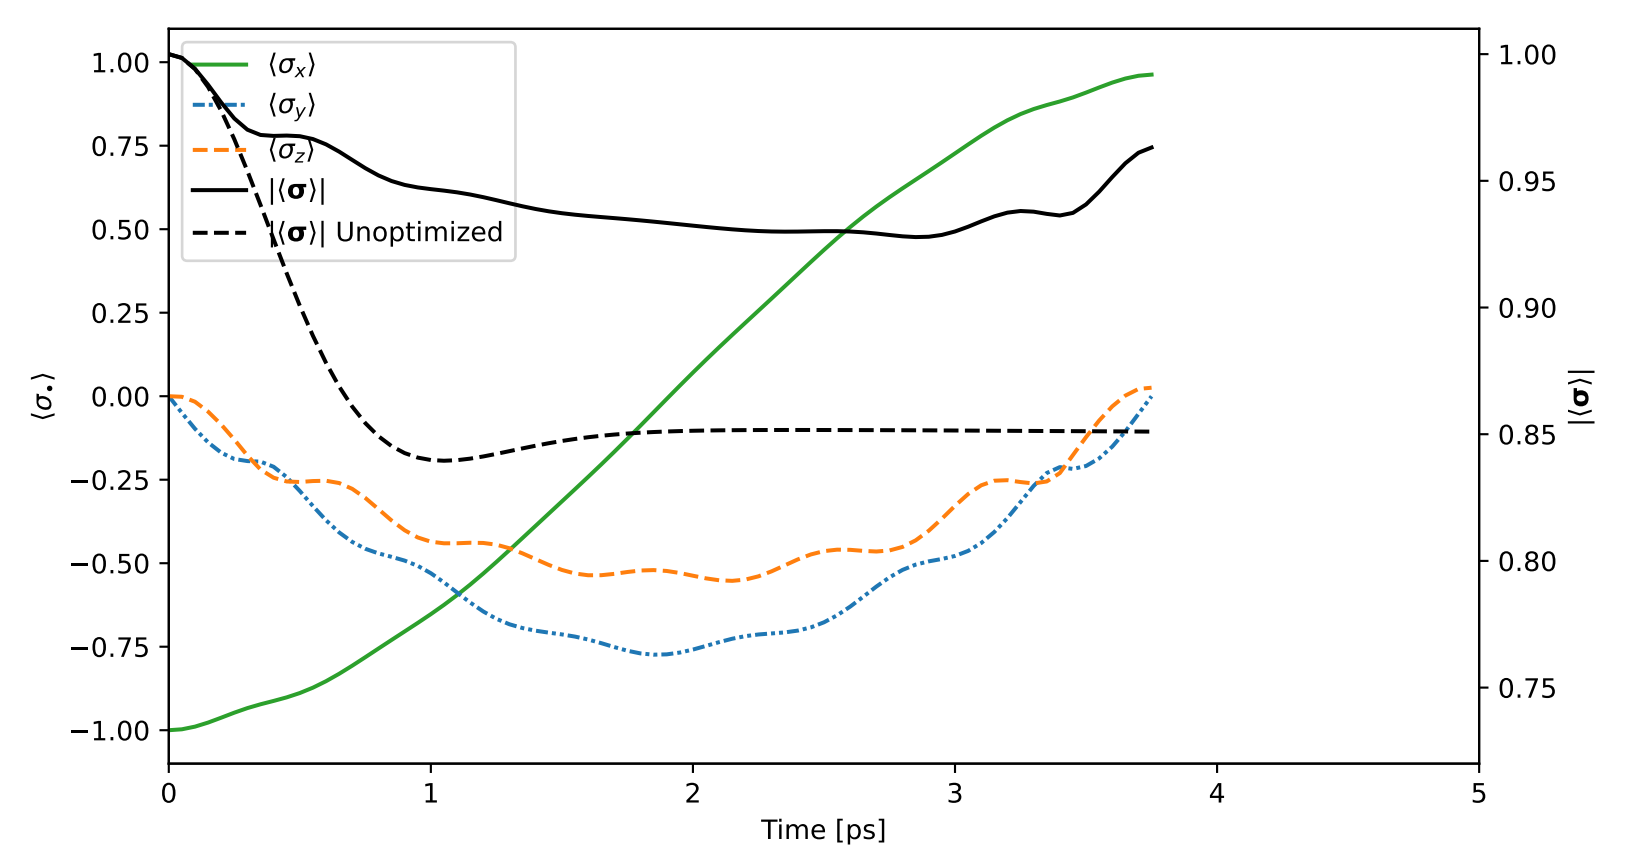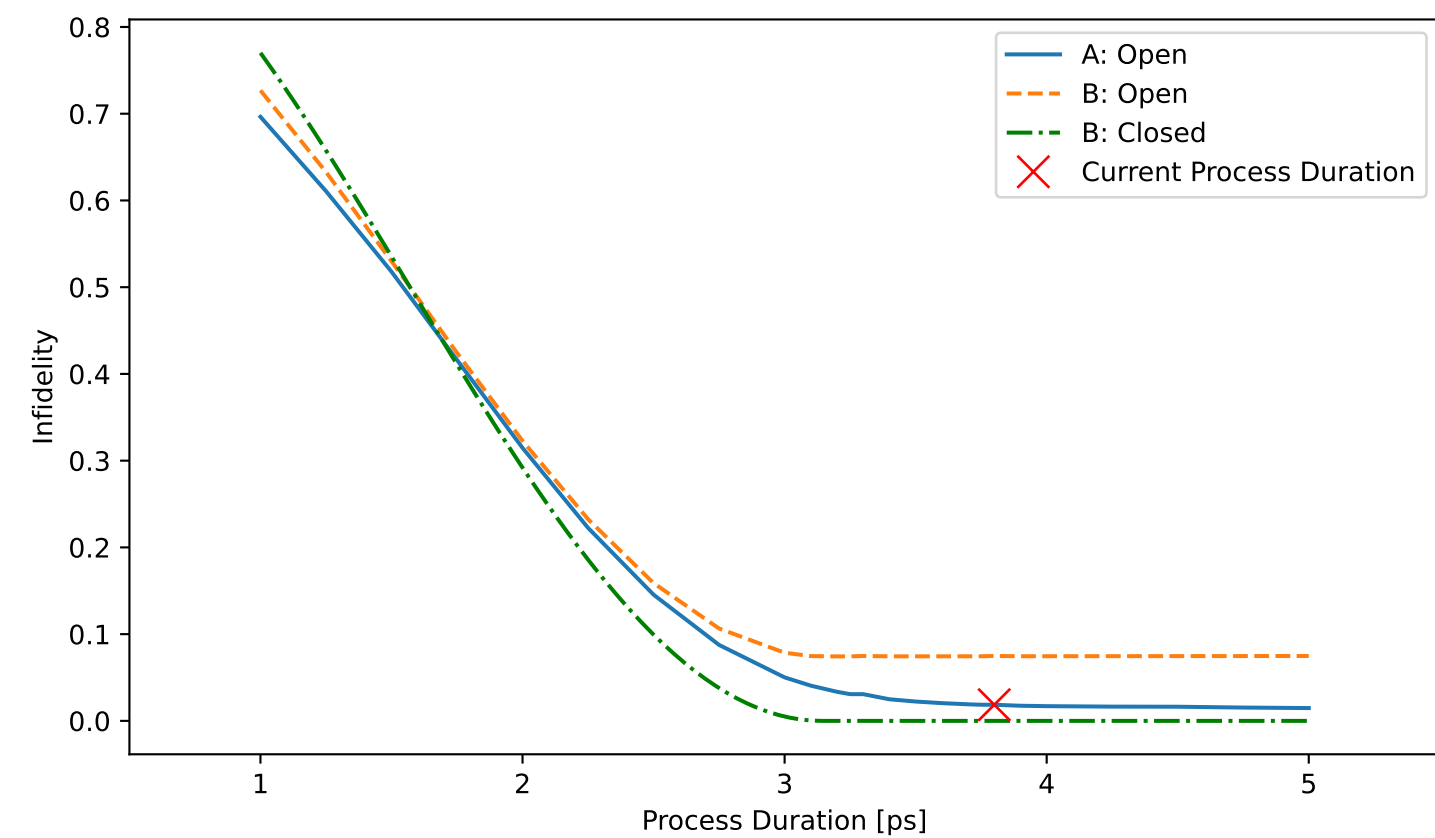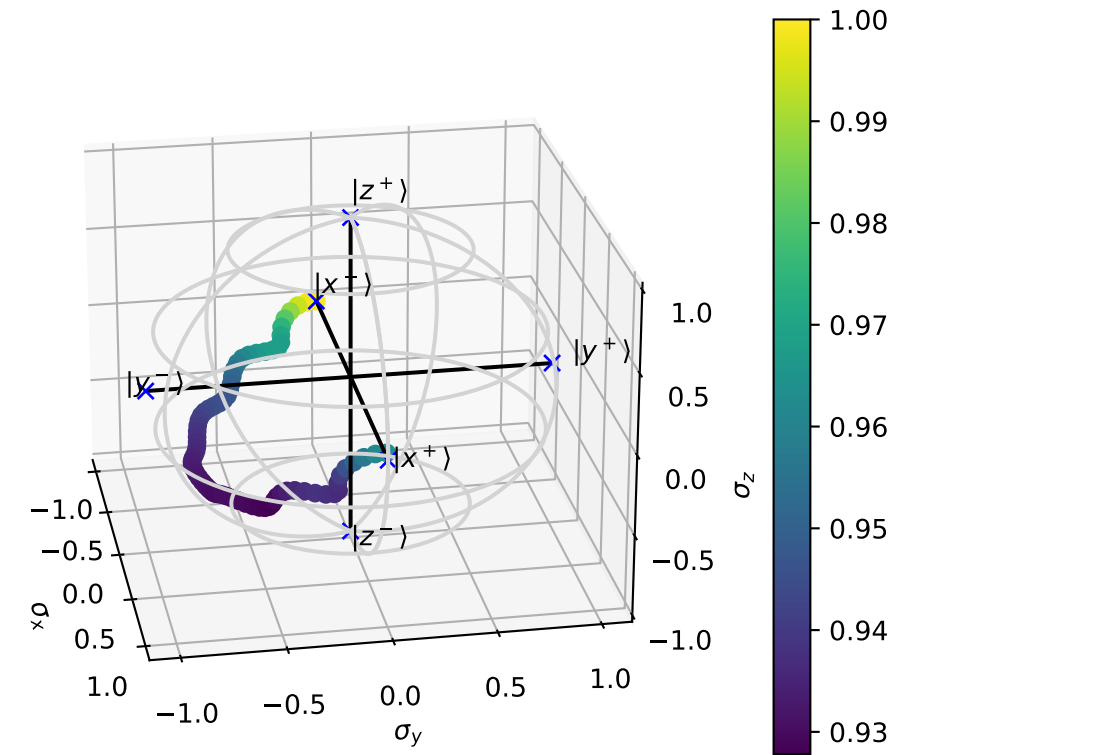

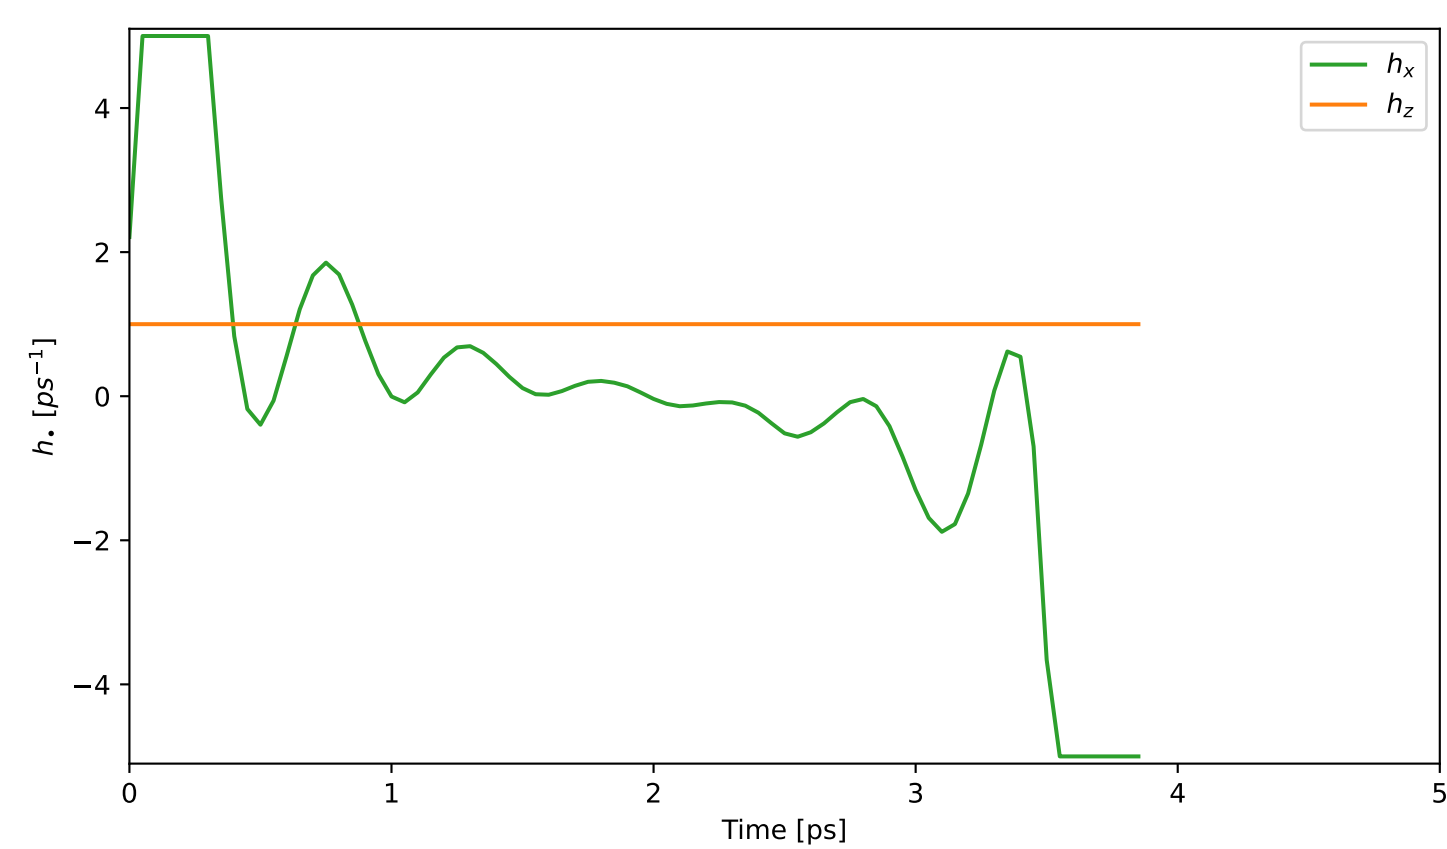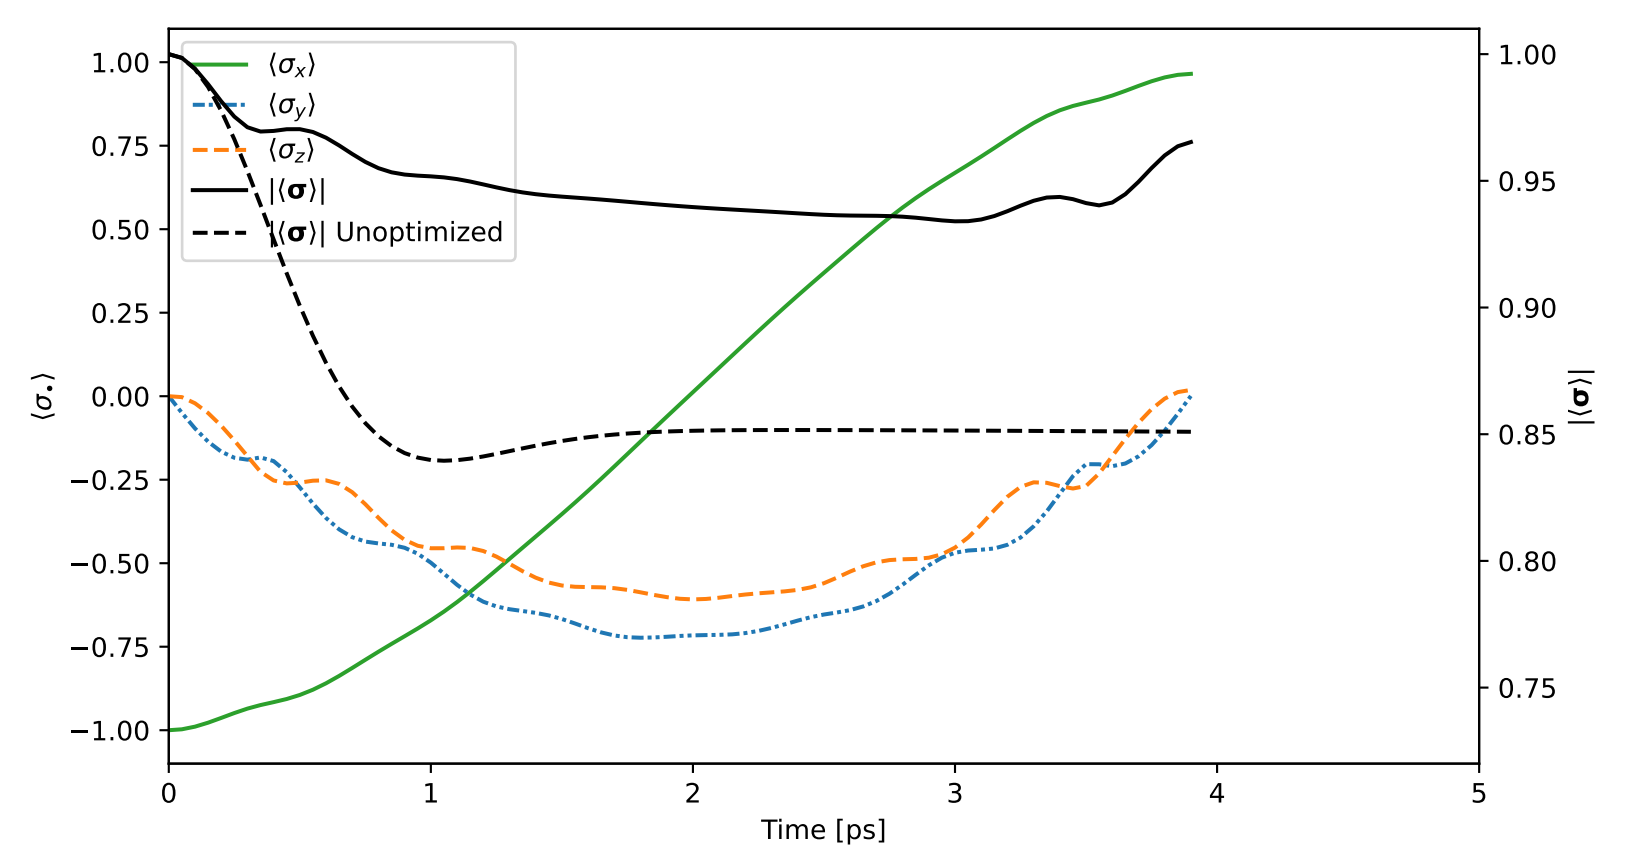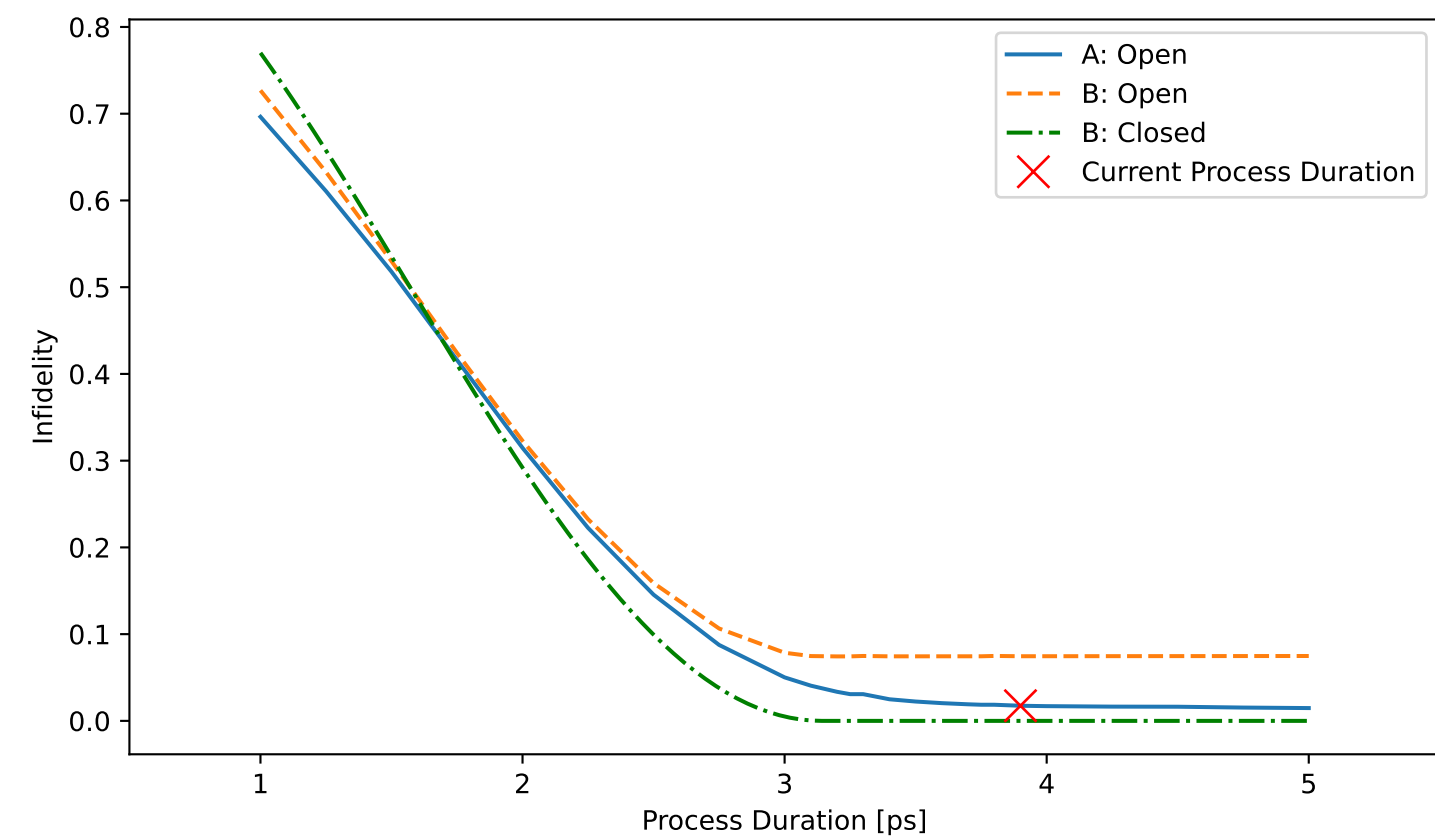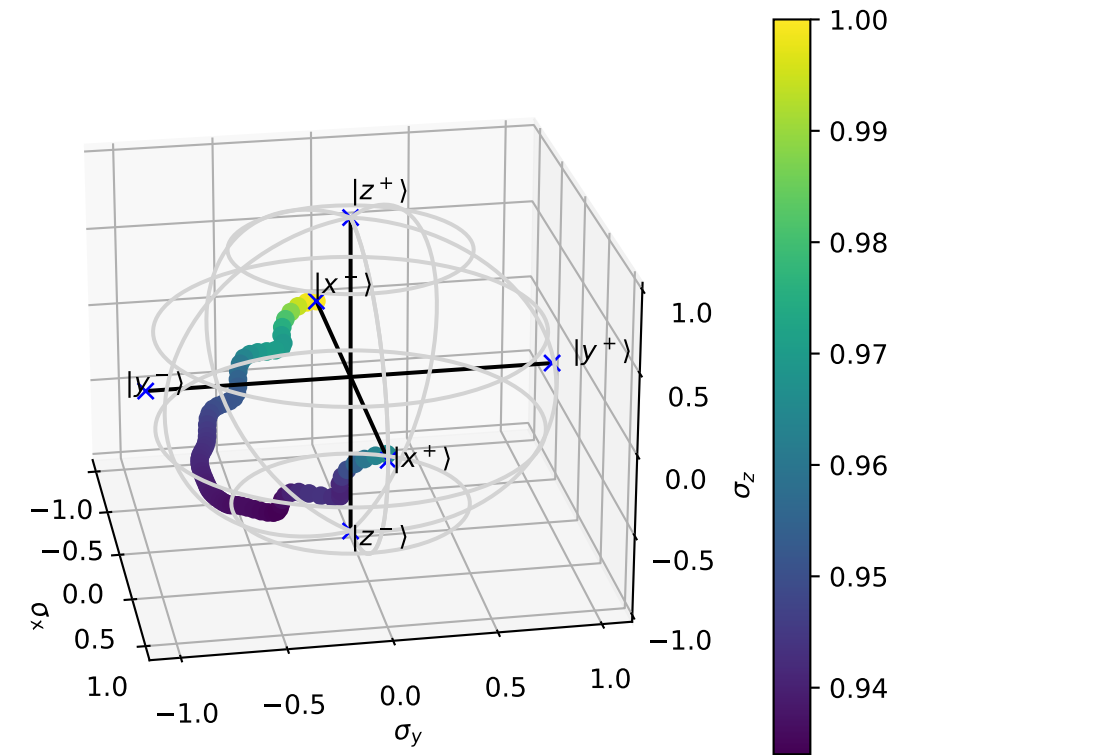

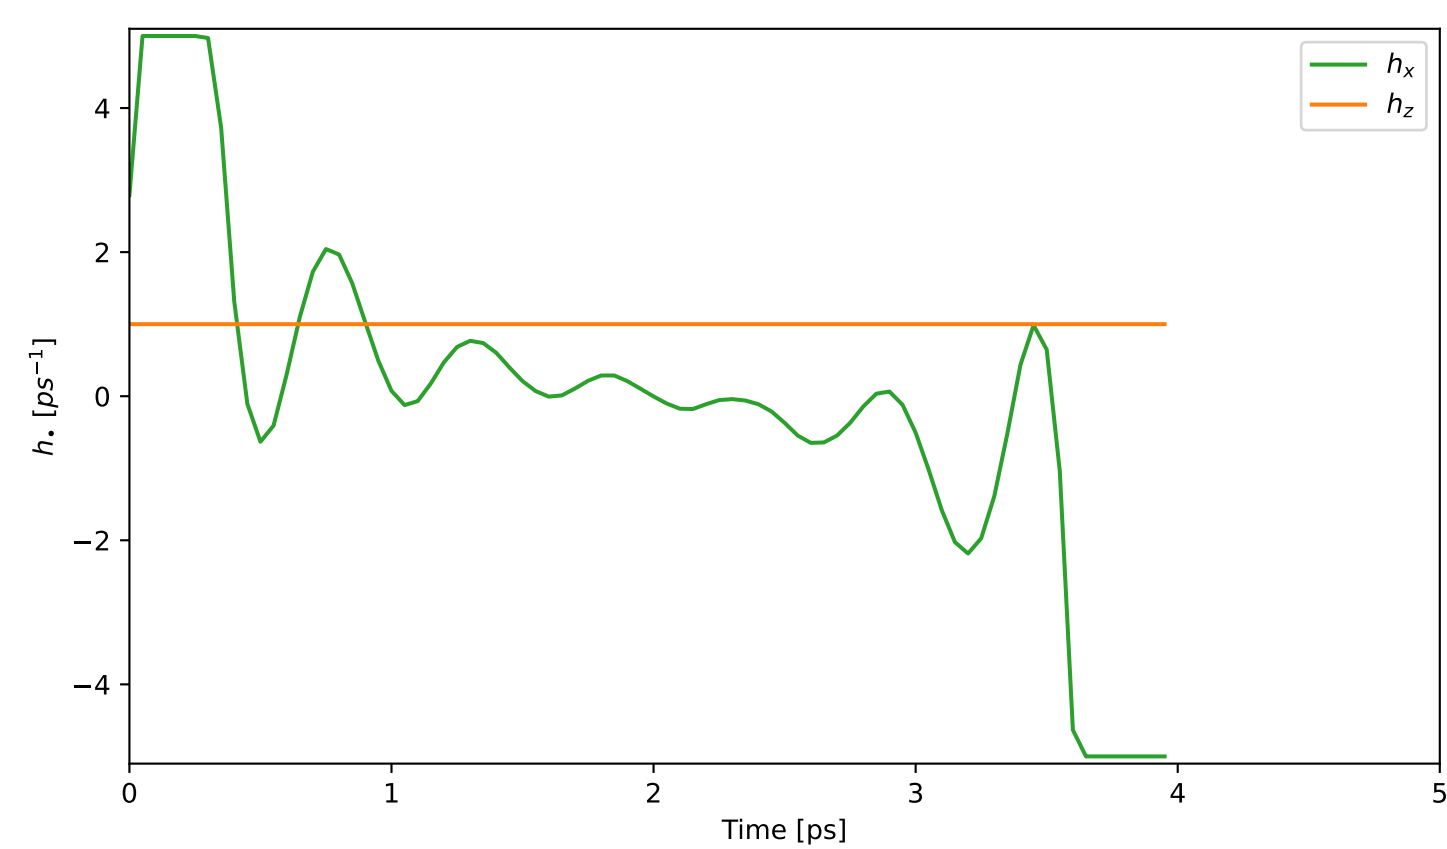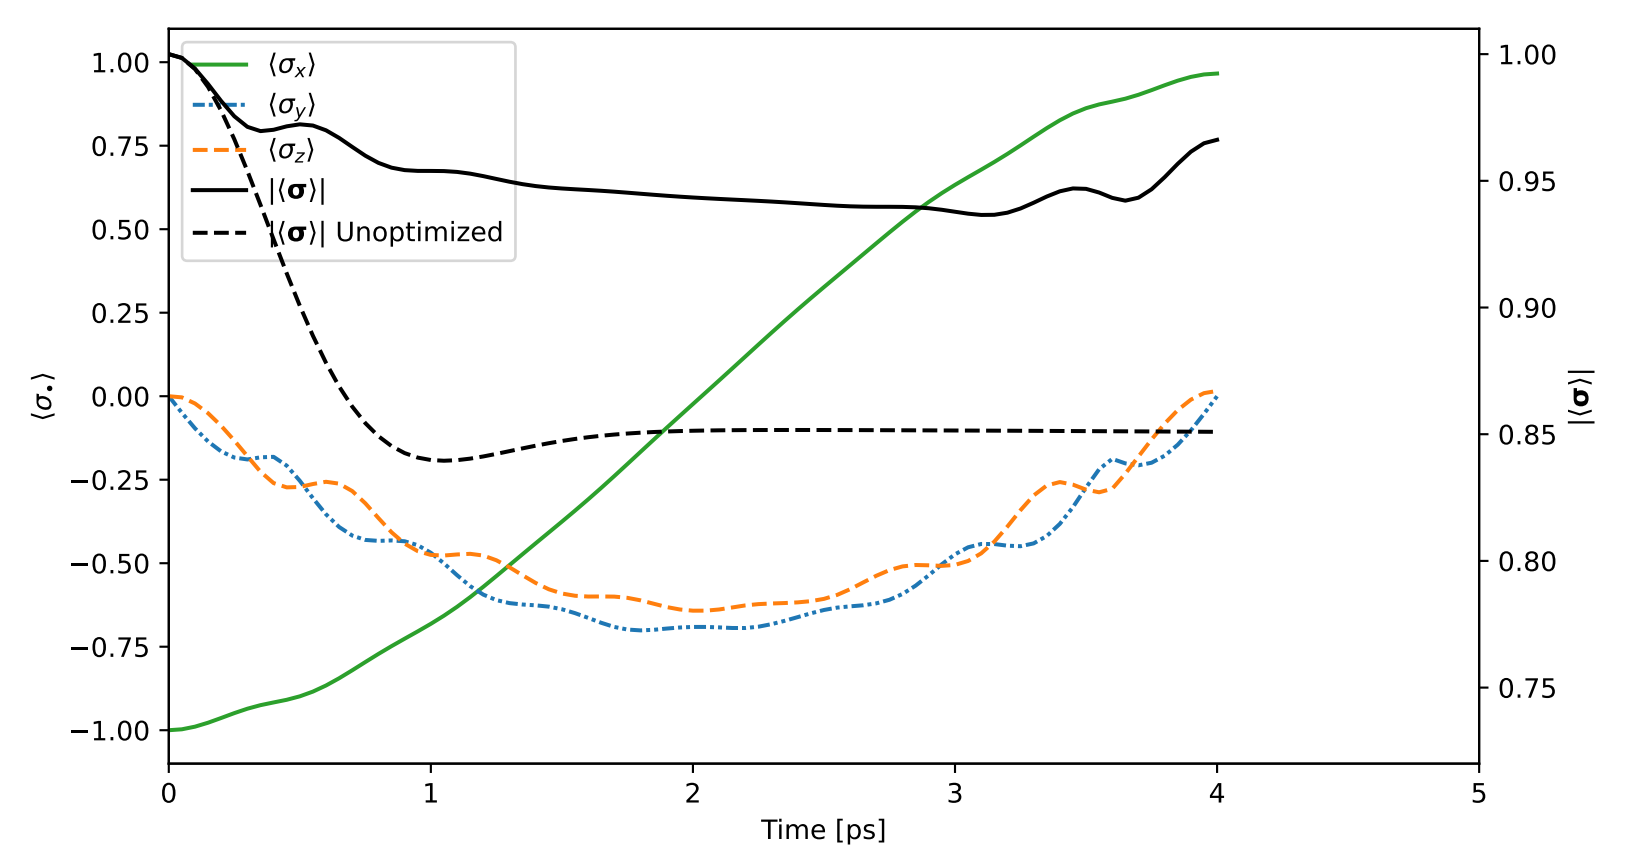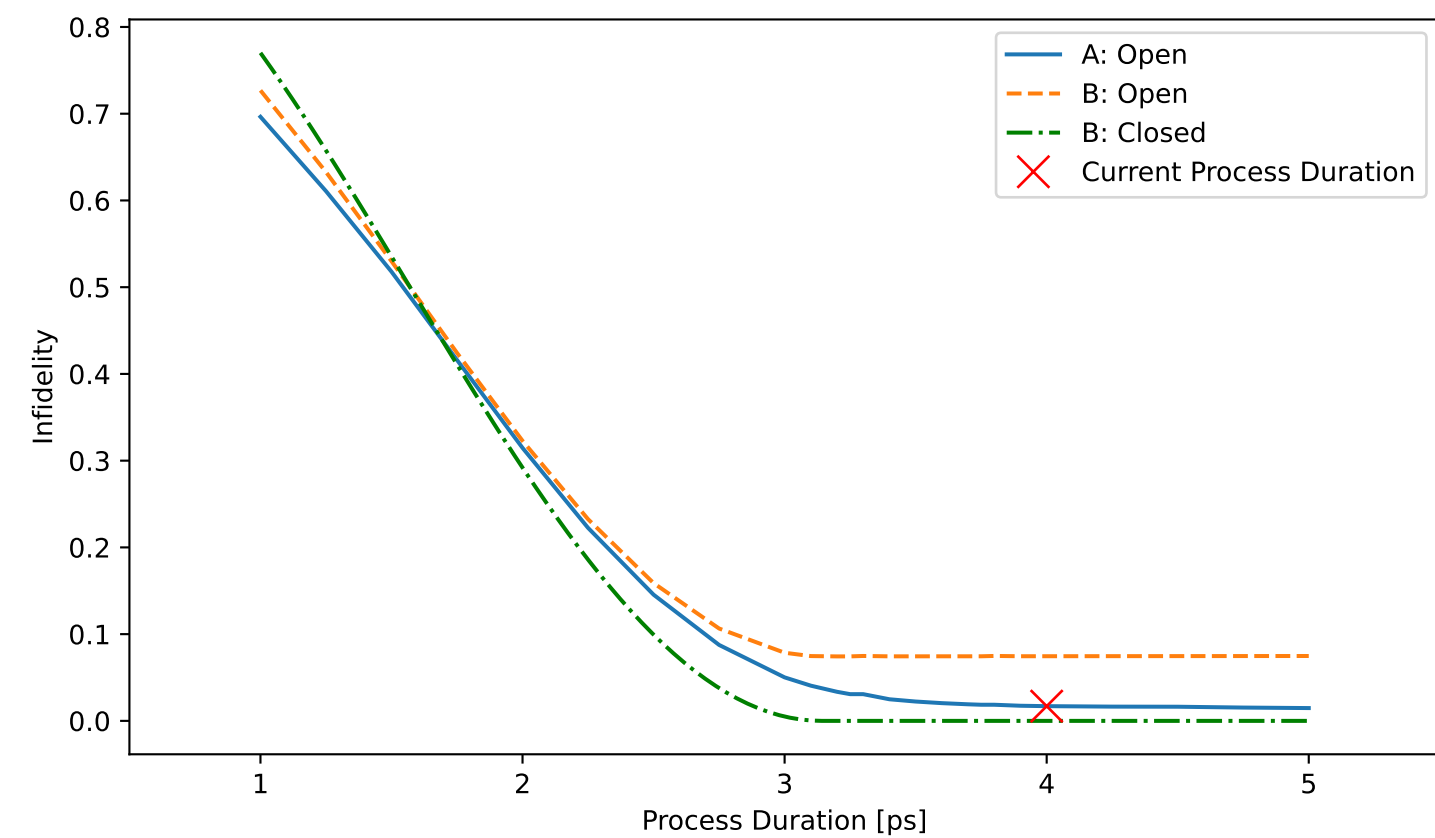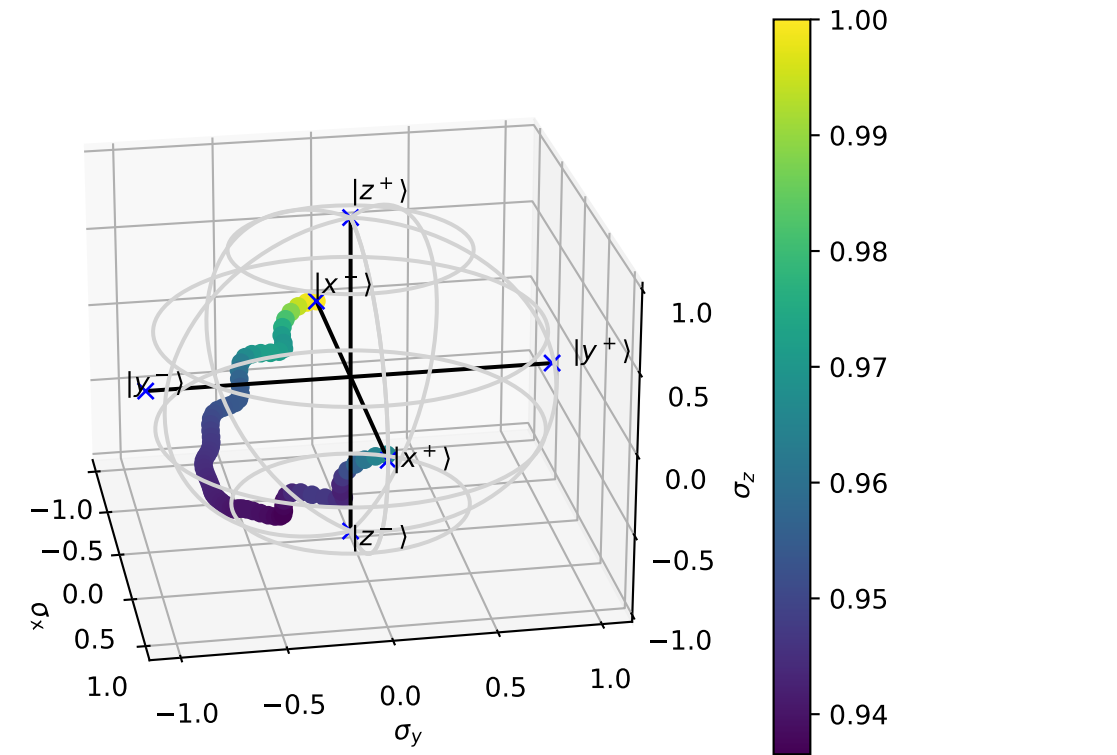

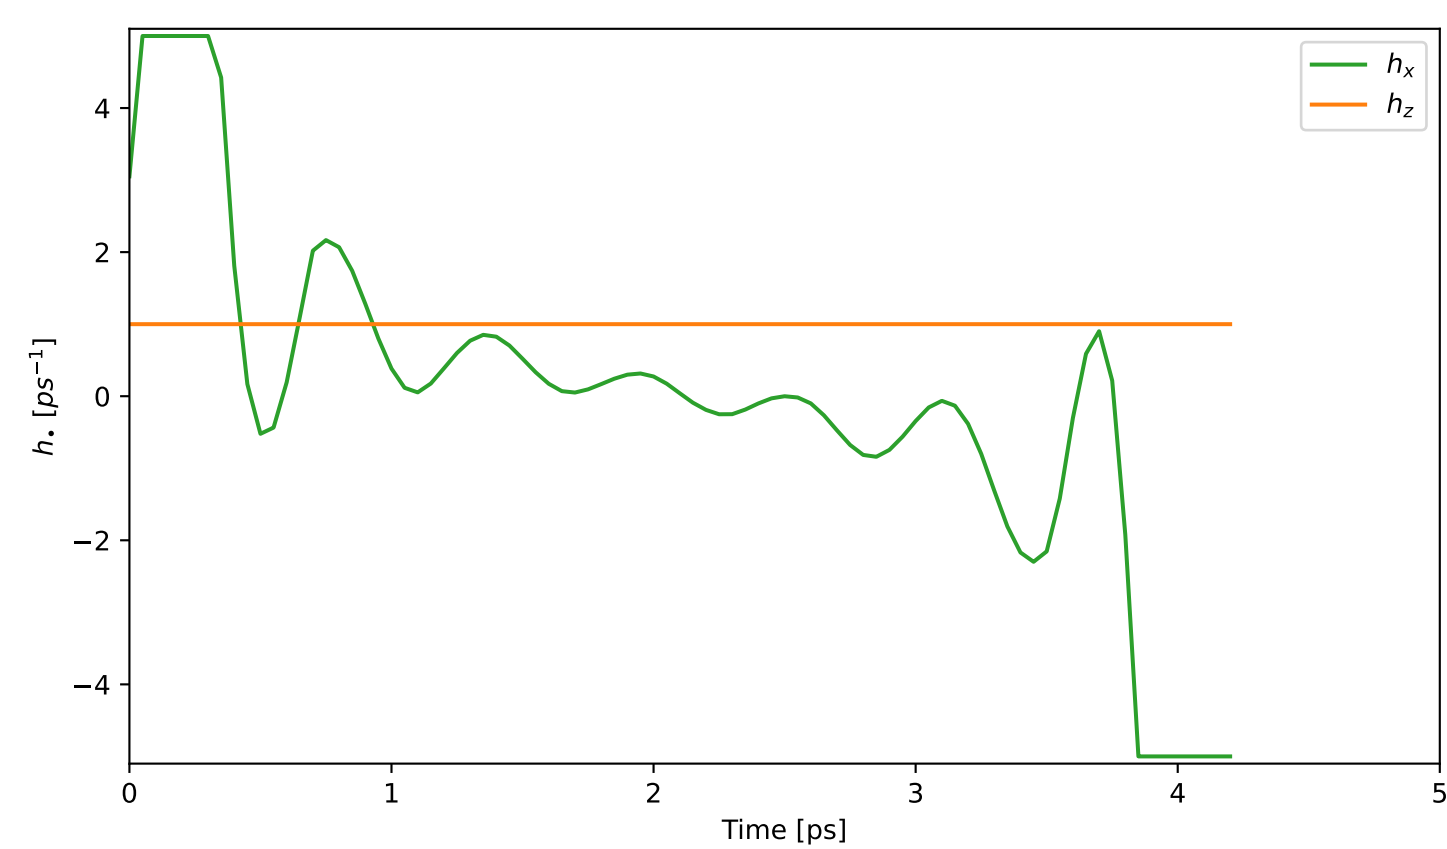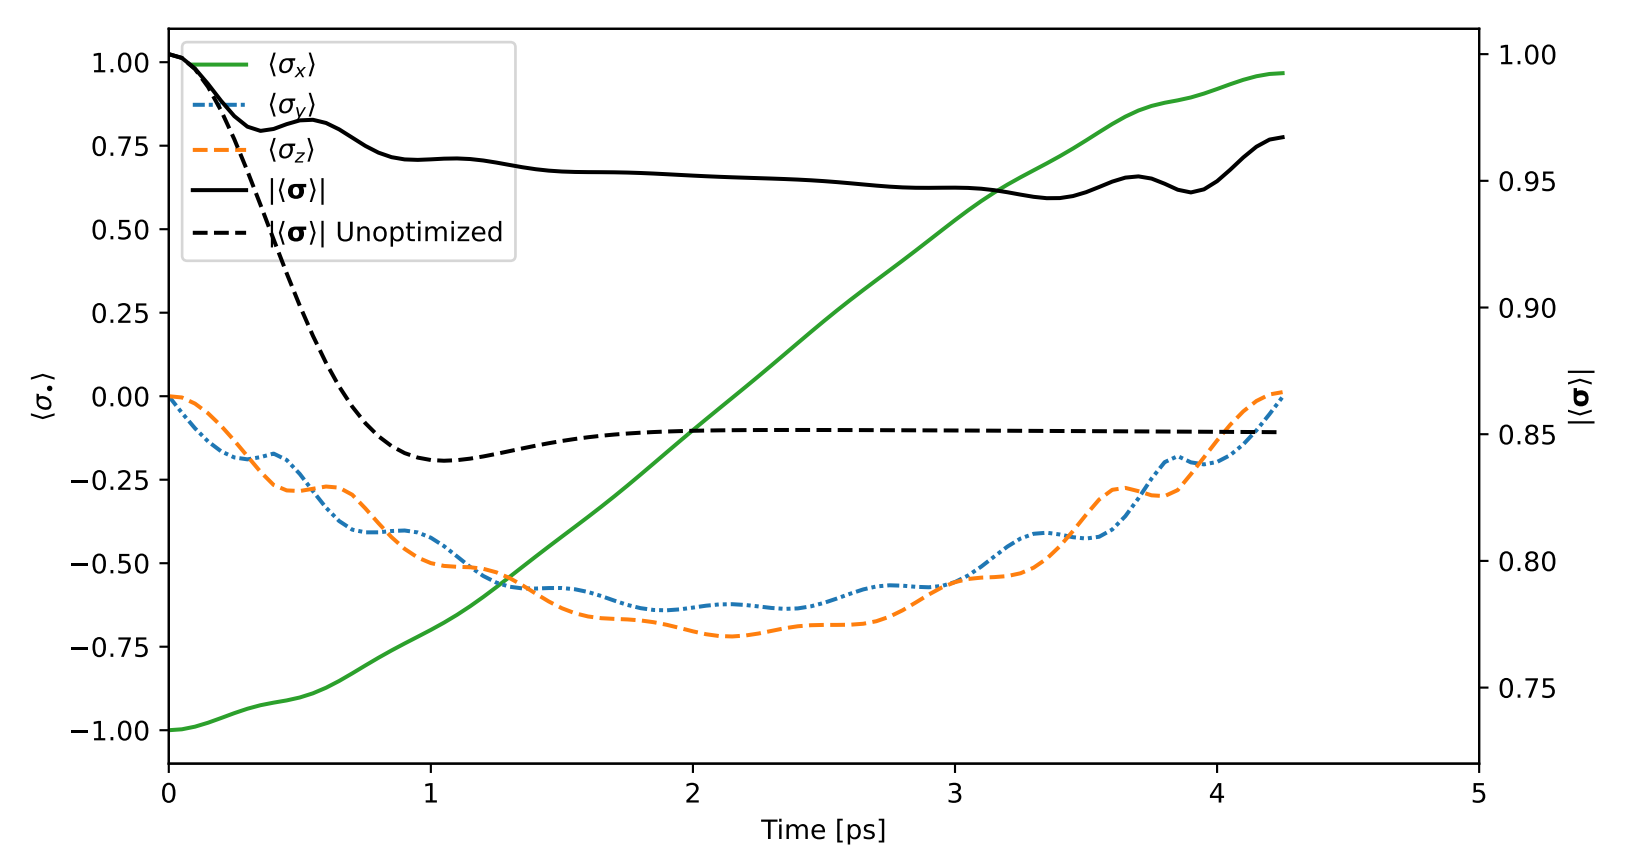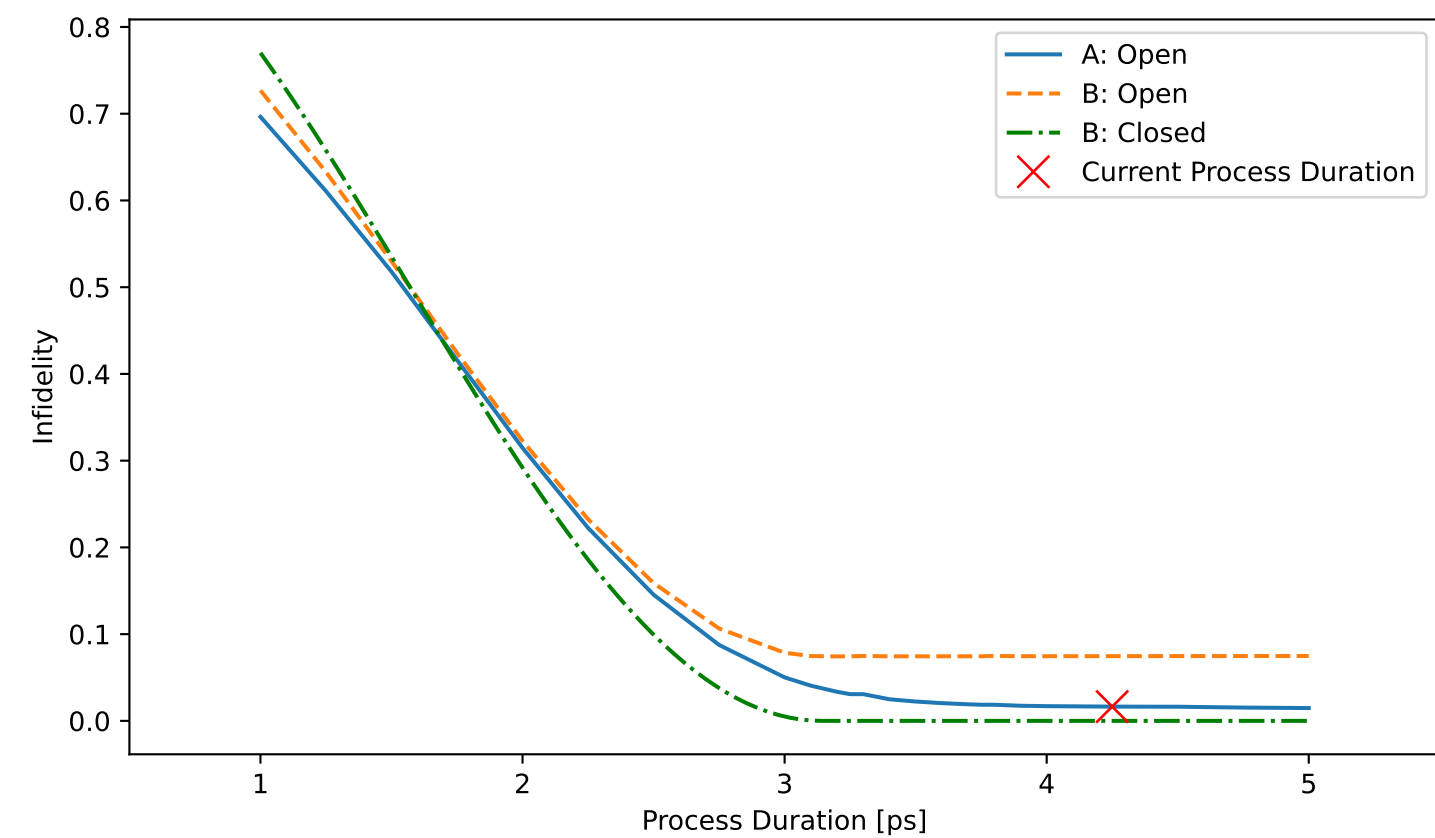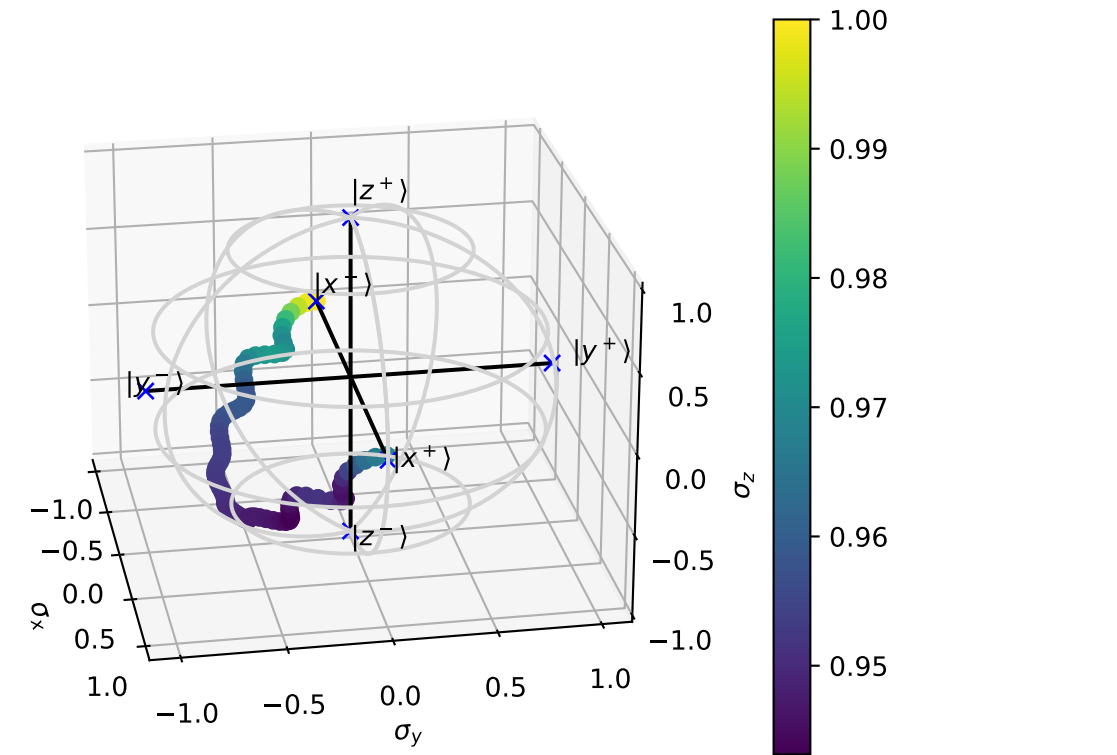

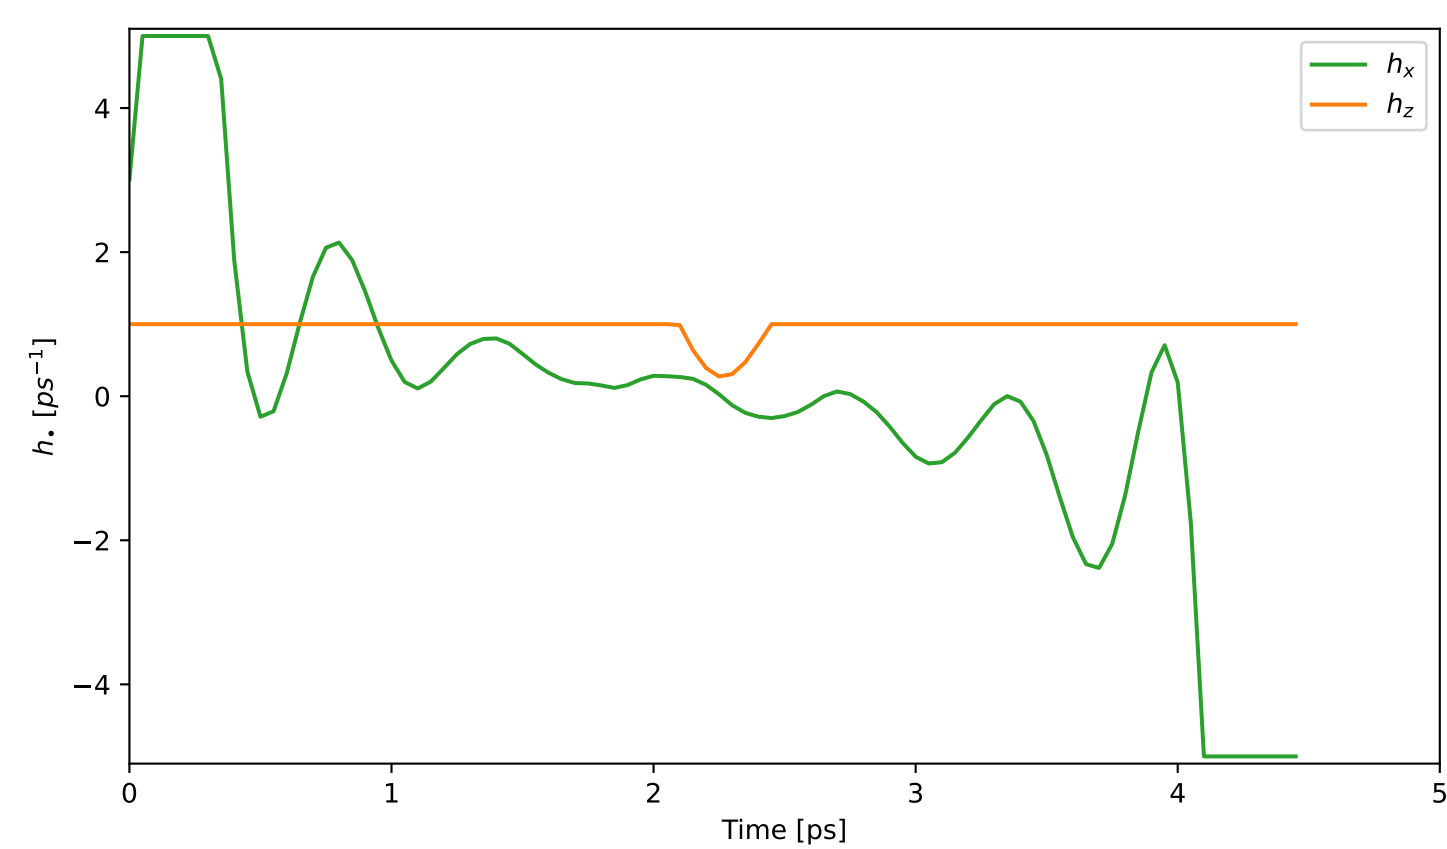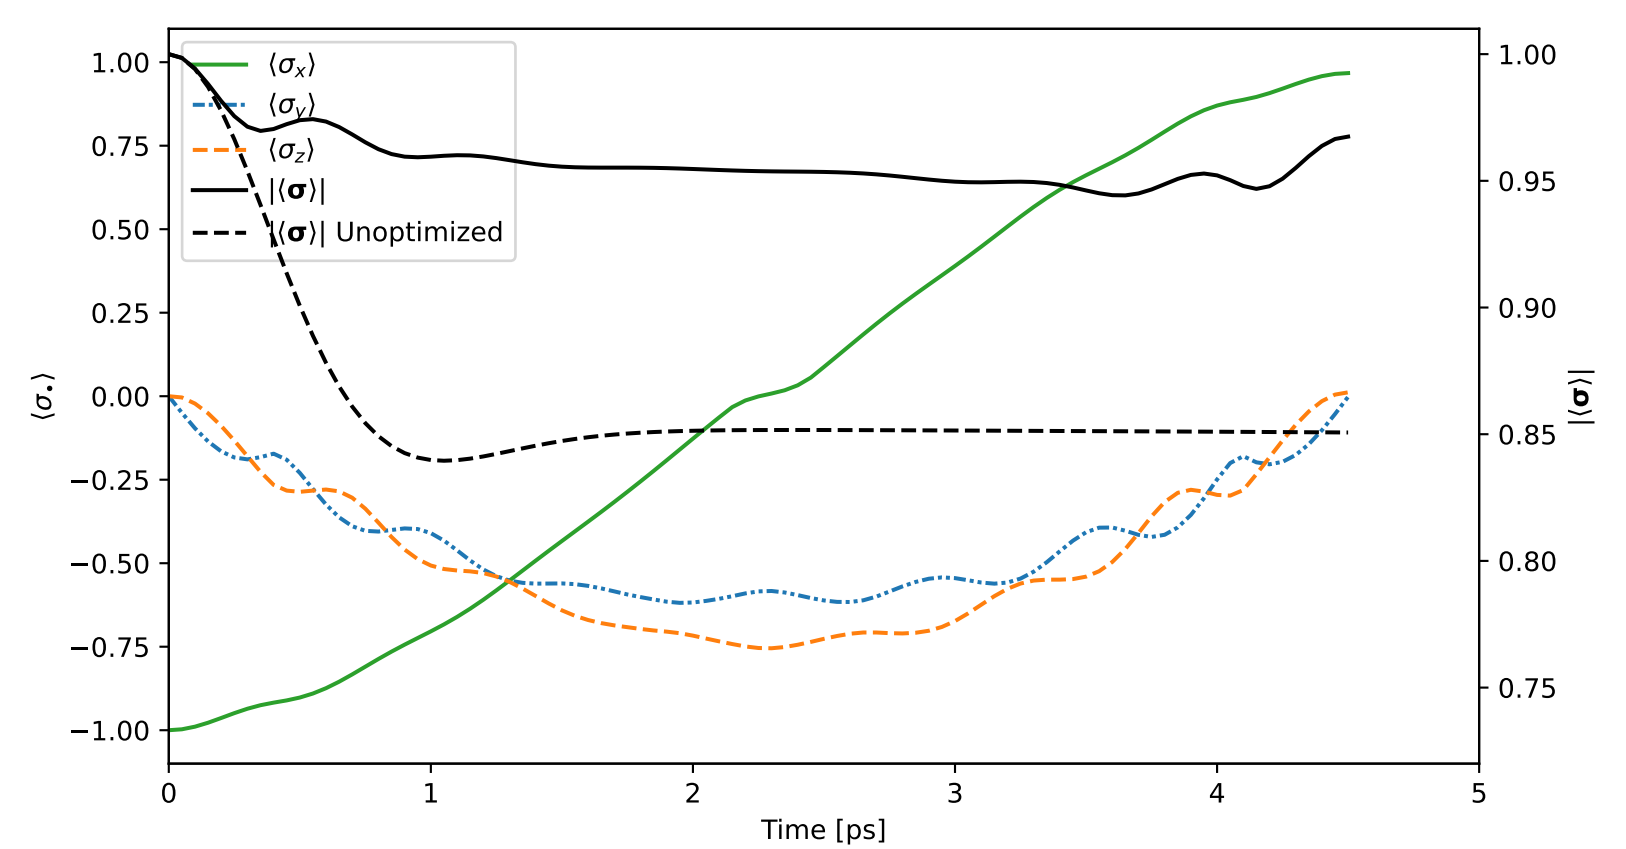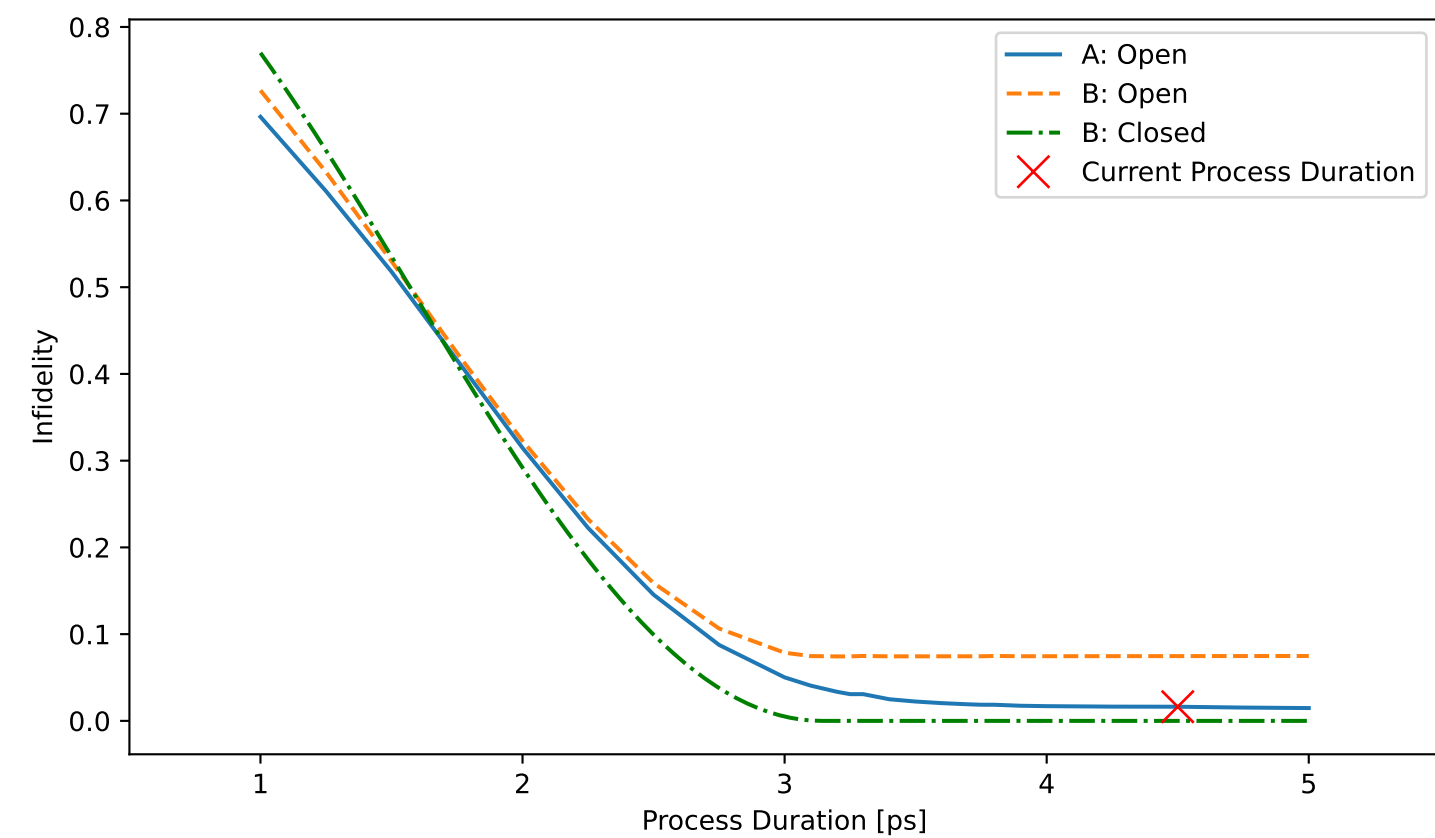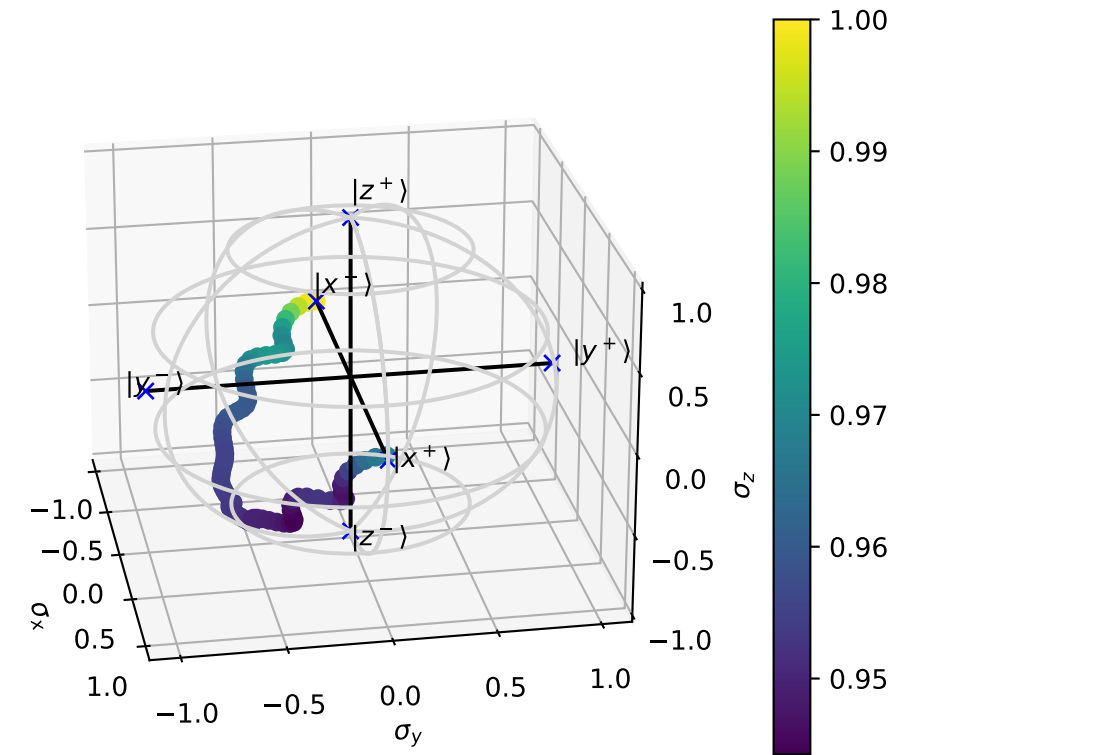



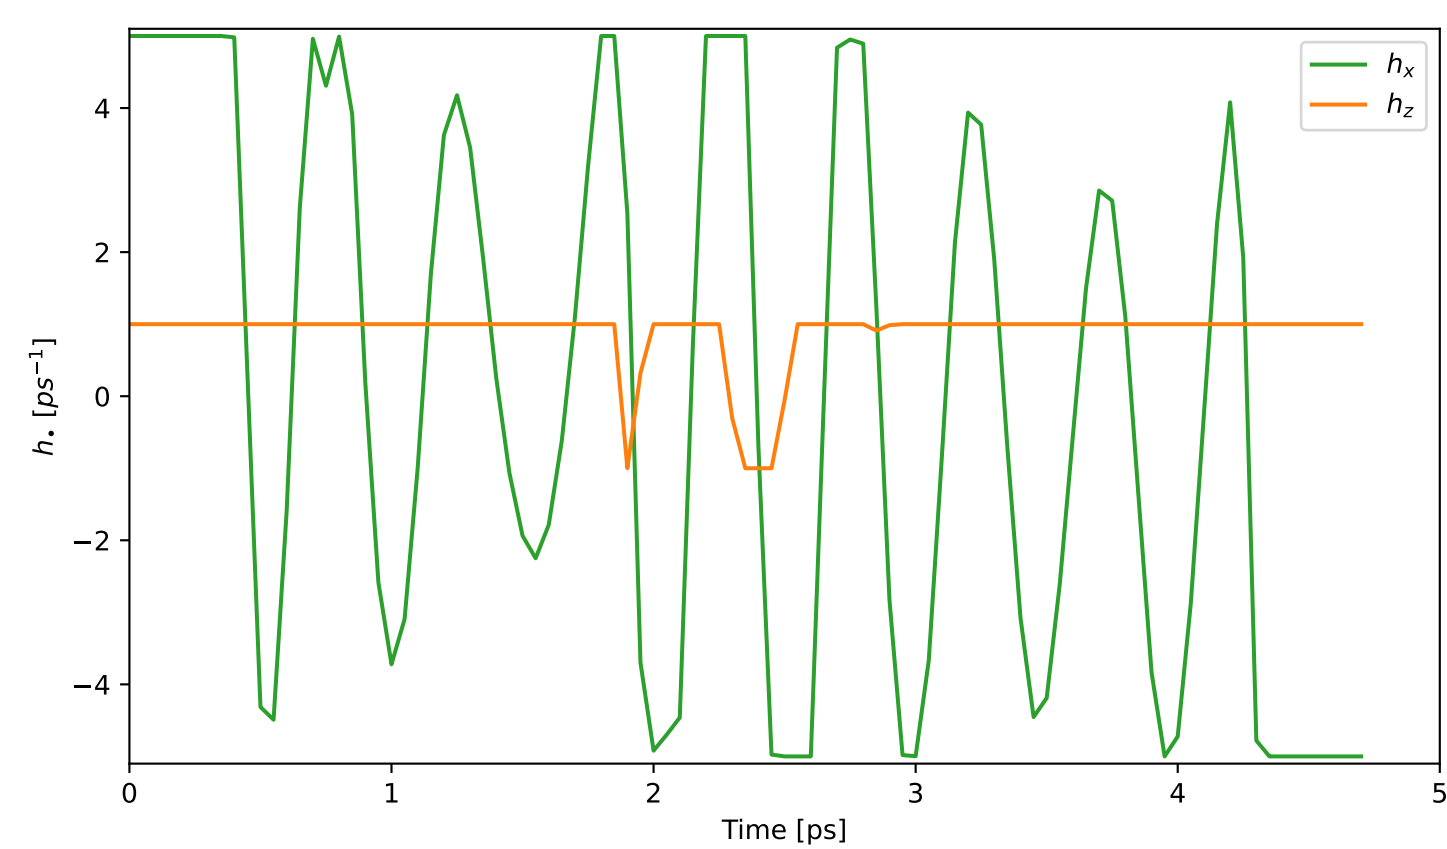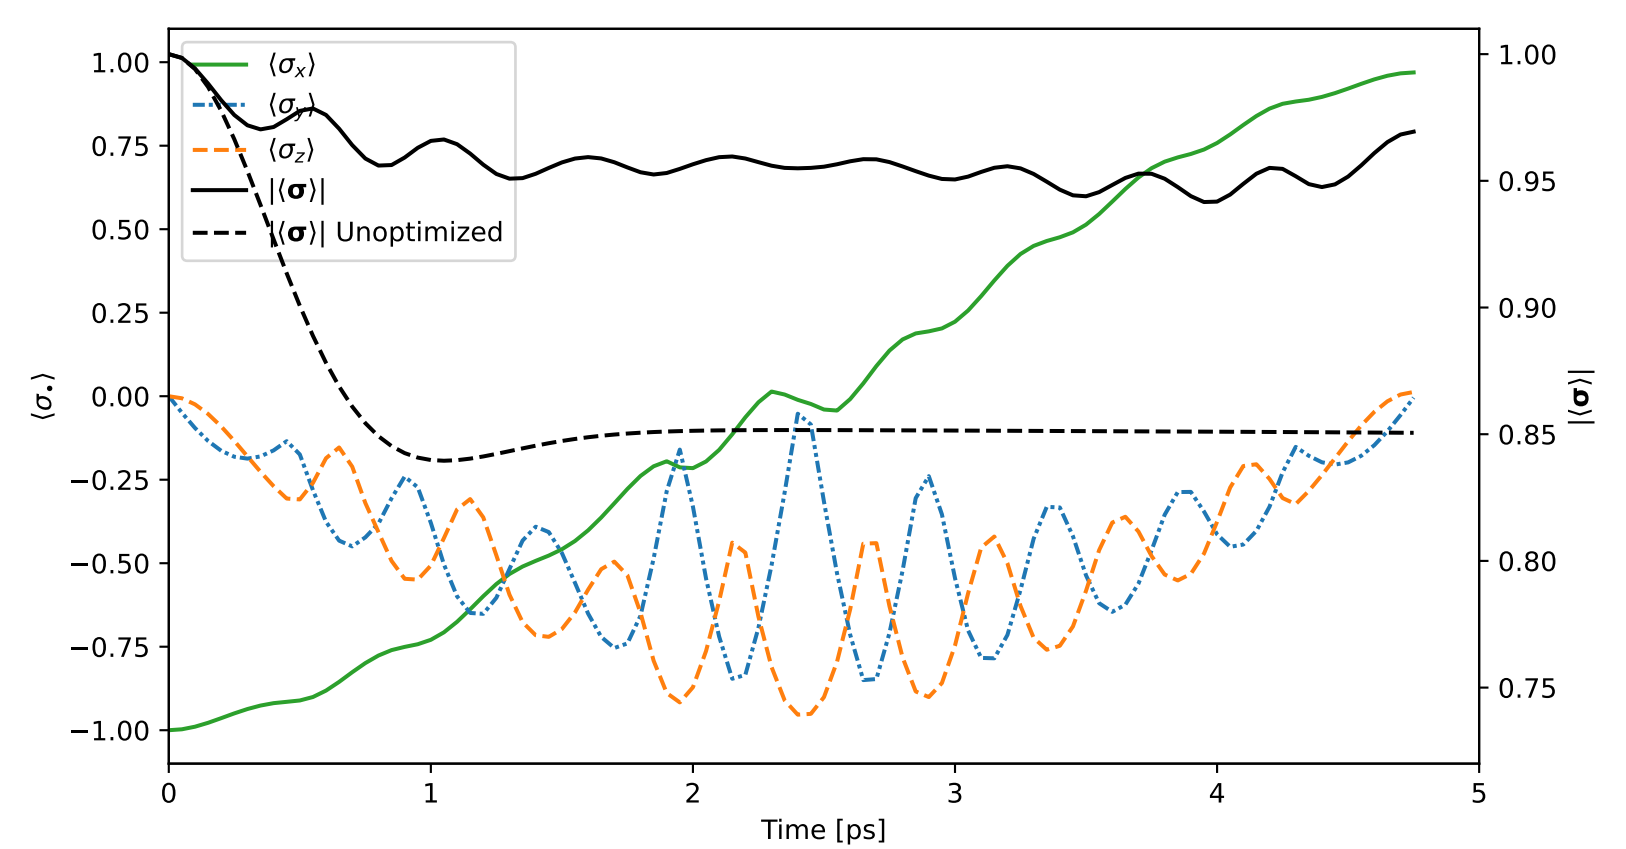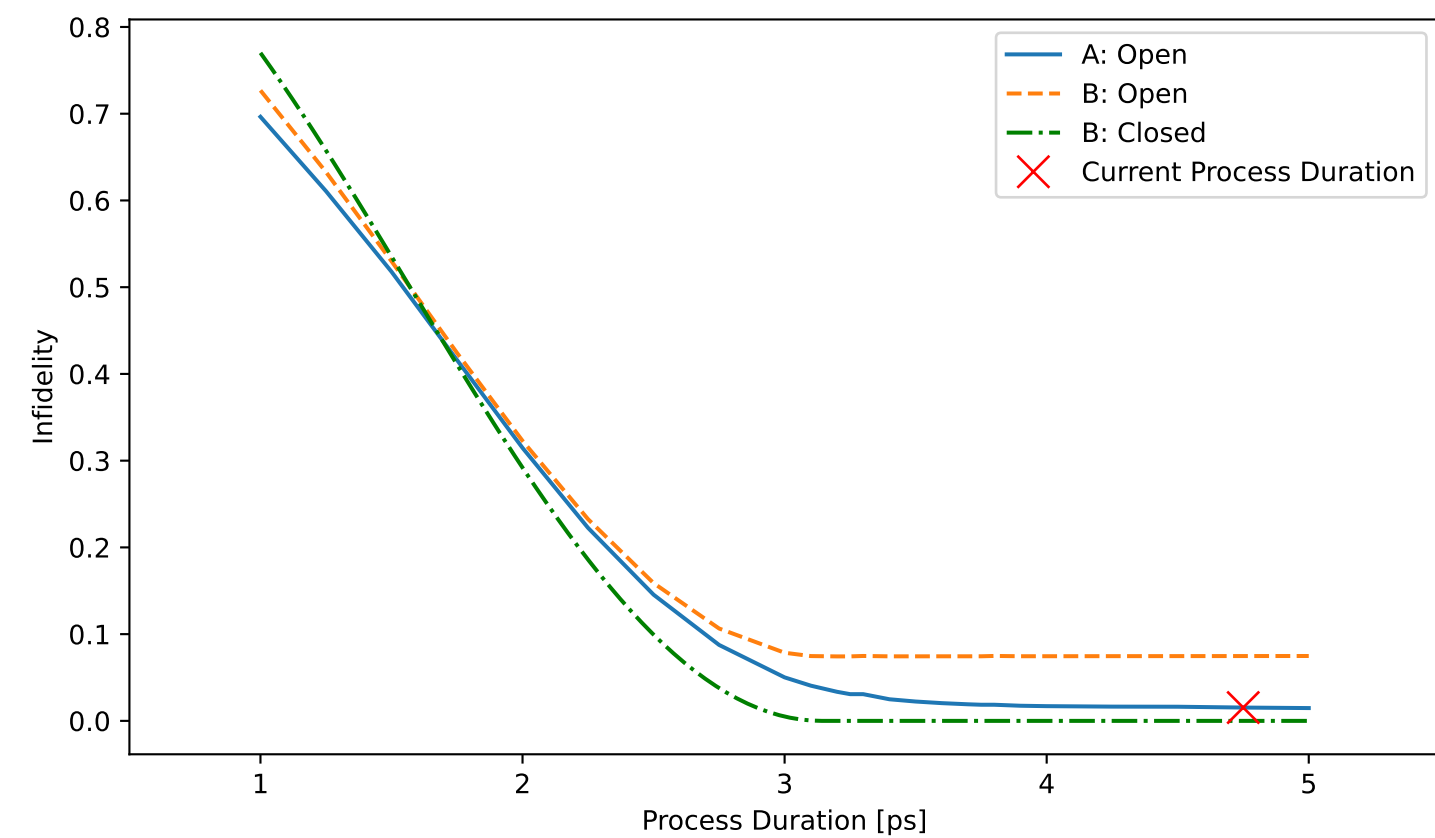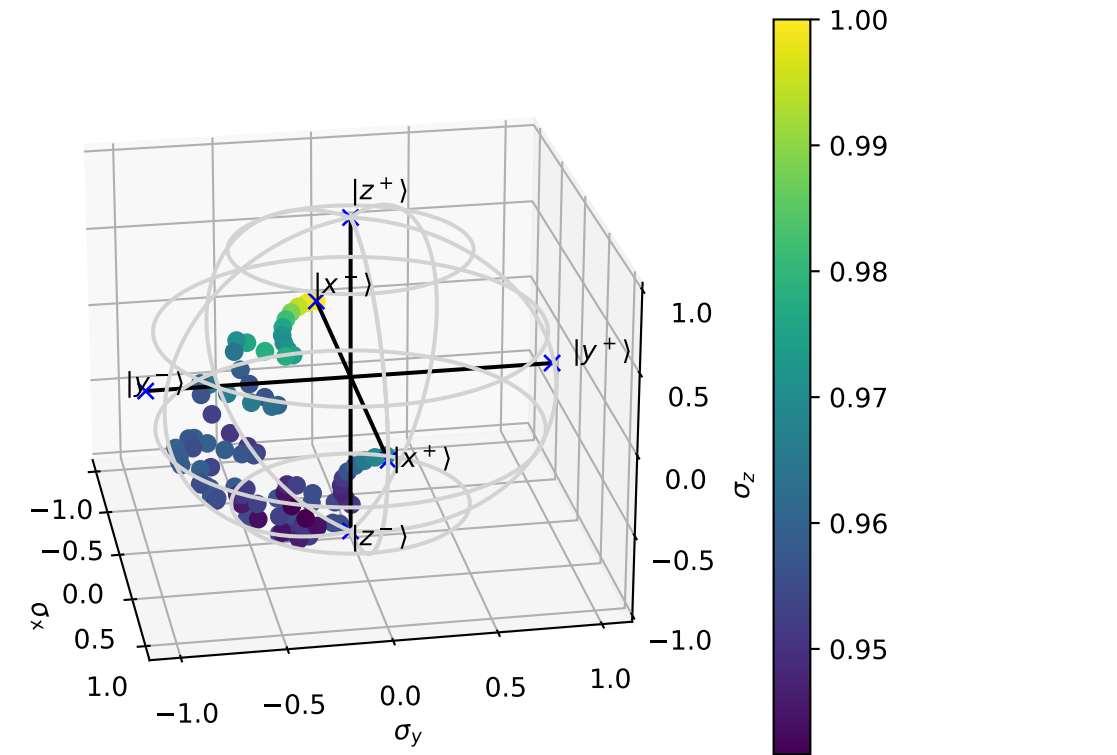

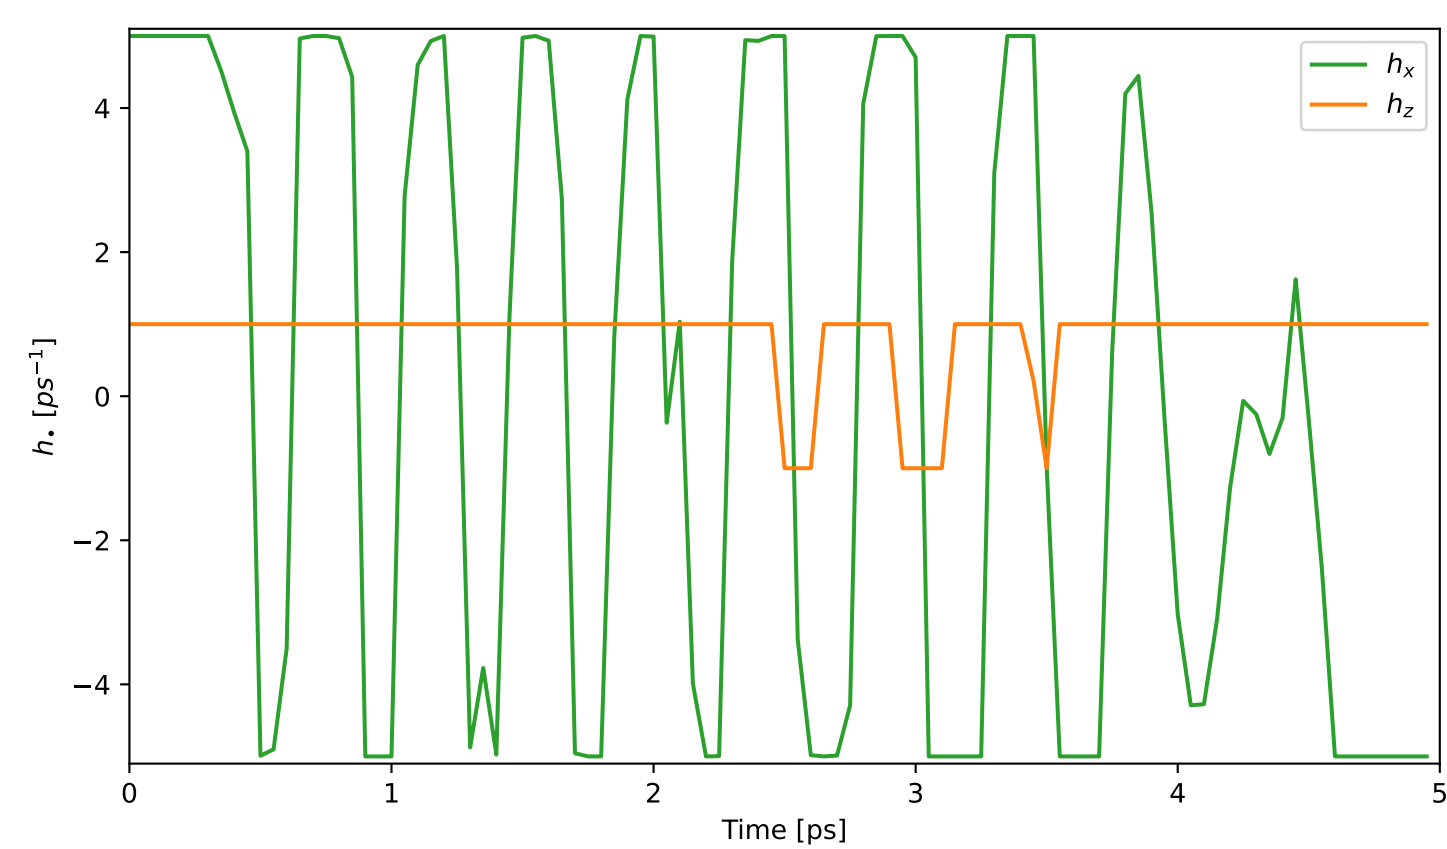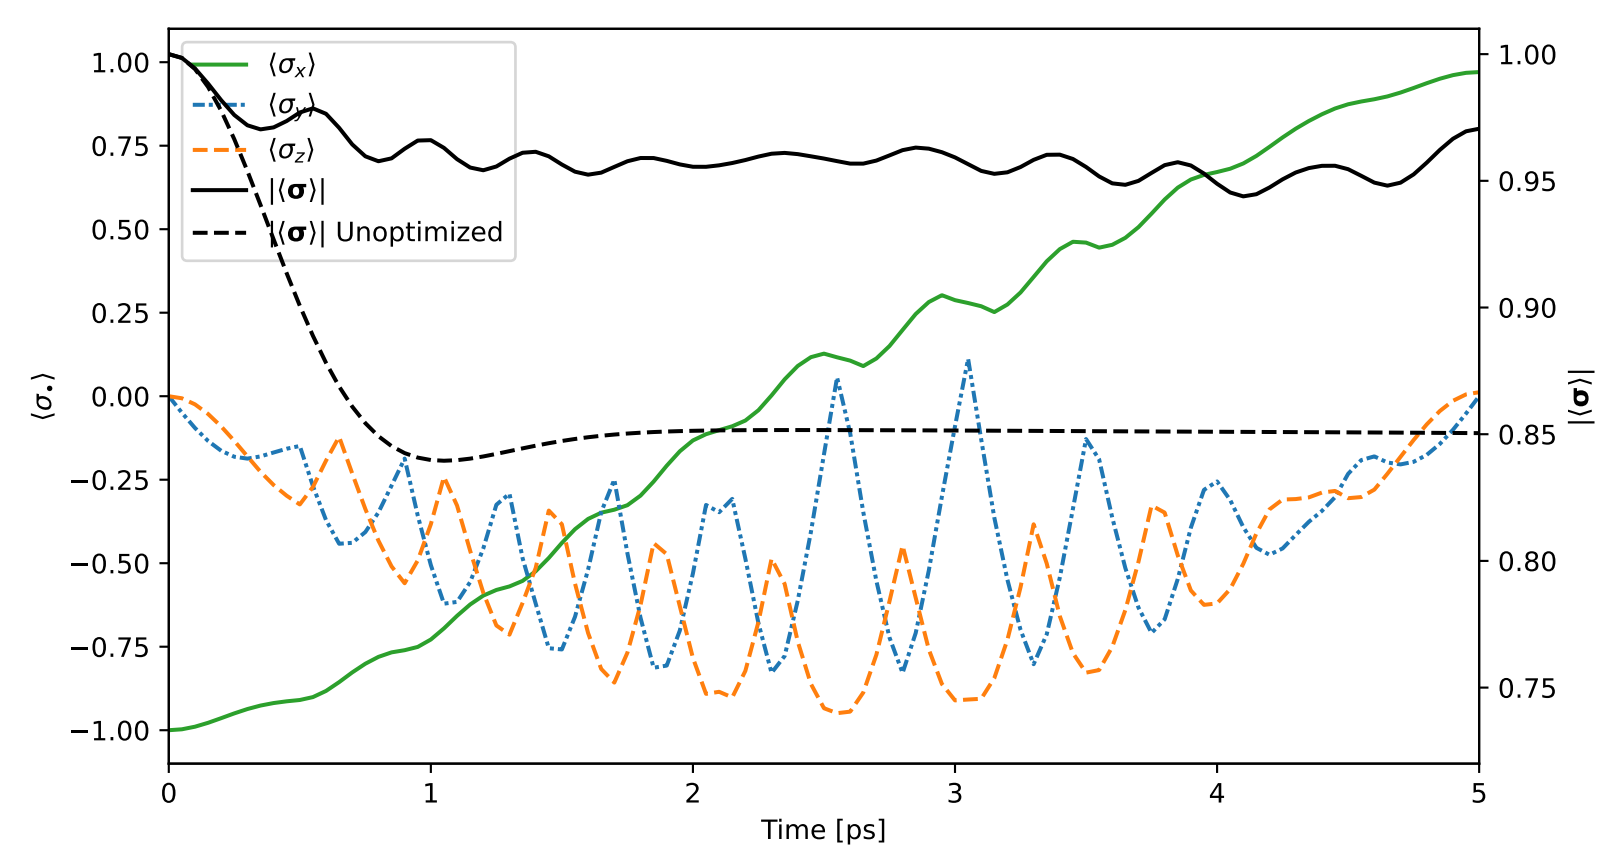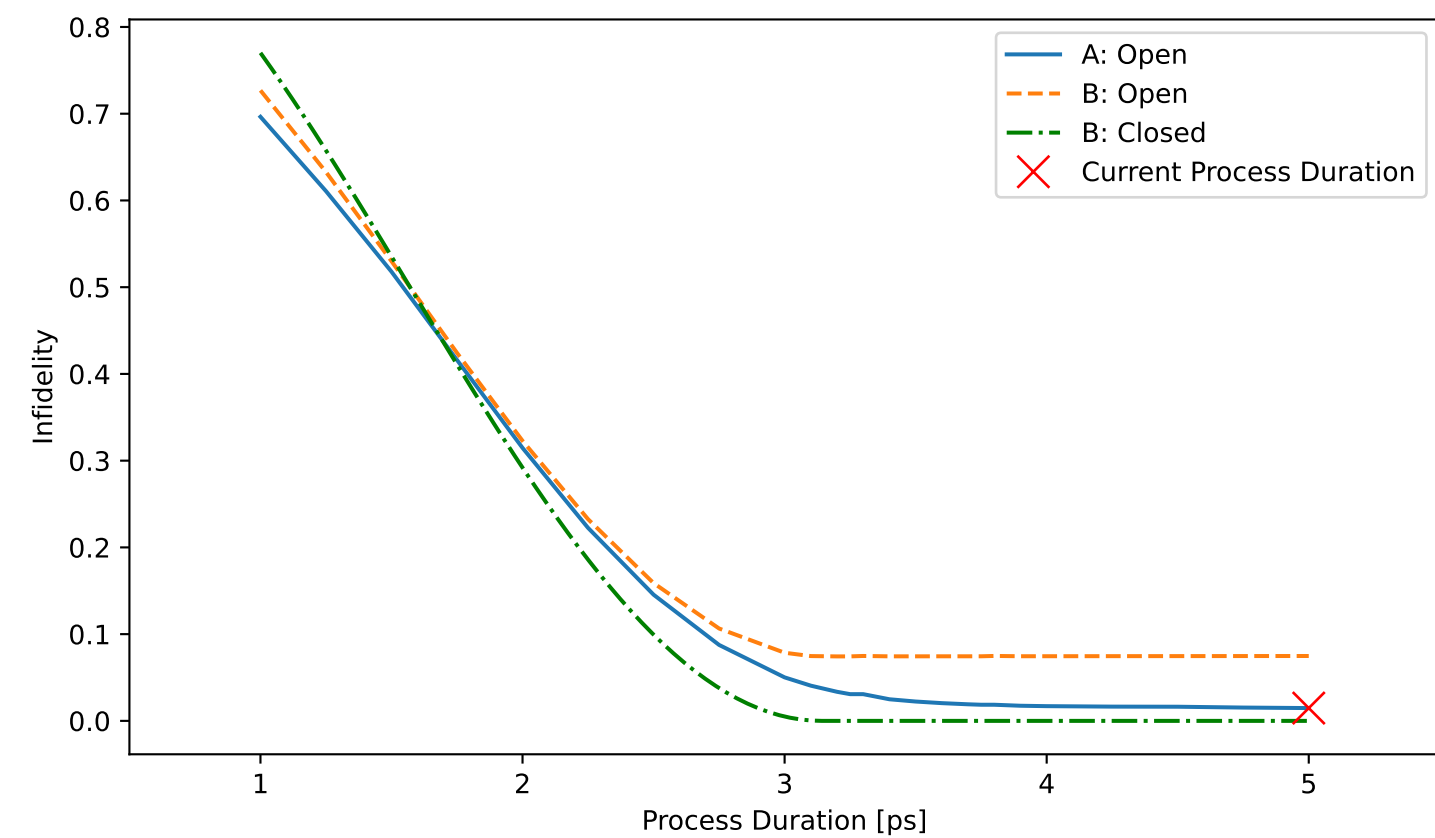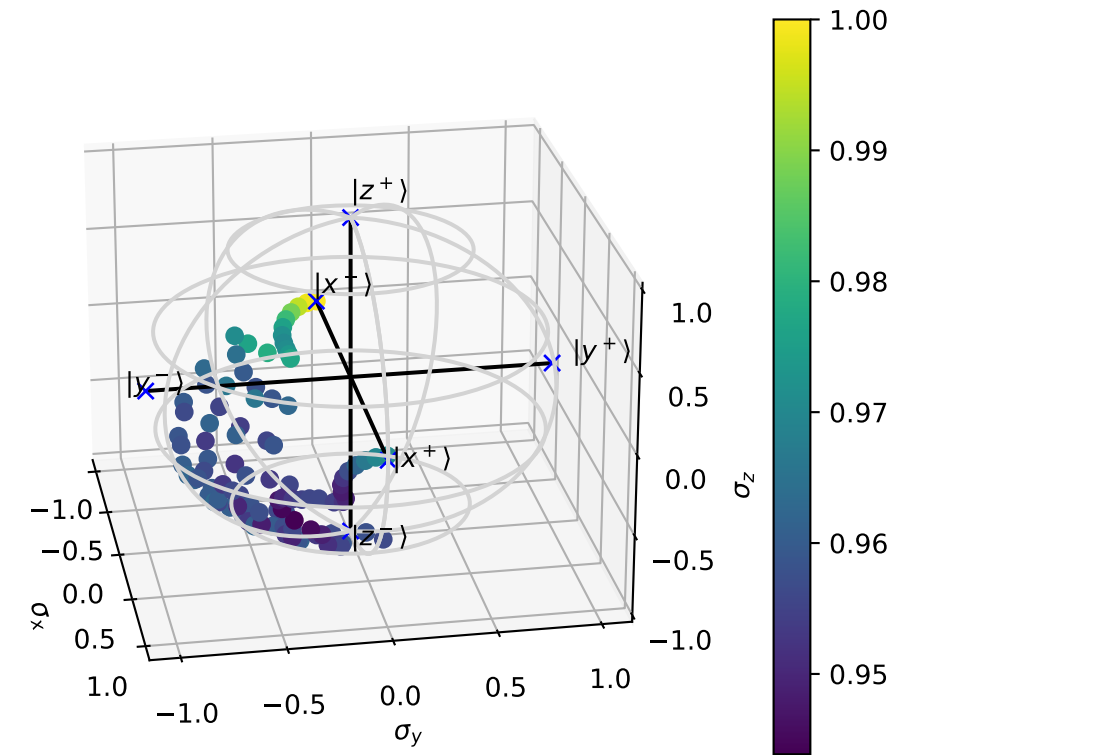

Supplement: Supplementary file 1 [file SI_slideshow.pdf]
